# Supplementary material for: Parametrization of cross sections for elementary hadronic collisions involving strange particles
Source: arXiv:1805.01655 ancillary file (2018-05-04)
Supplement: Supplementary file 1 [file tabulation.pdf]

| Momentum<br>(MeV/c) | A1/A0   | A2/A0    | A3/A0   | A4/A0    | A5/A0    | A6/A0    | A7/A0 | A8/A0 | A9/A0 | A10/A0 |
|---------------------|---------|----------|---------|----------|----------|----------|-------|-------|-------|--------|
| 225                 | 0.14007 | -0.1329  | 0.00044 | -0.00469 | -0.00254 | -0.00011 | 0     | 0     | 0     | 0      |
| 230                 | 0.14143 | -0.1335  | 0.00058 | -0.00417 | -0.00248 | -4E-05   | 0     | 0     | 0     | 0      |
| 235                 | 0.14283 | -0.1179  | 0.00077 | -0.00364 | -0.00243 | 2E-05    | 0     | 0     | 0     | 0      |
| 240                 | 0.14428 | -0.08345 | 0.00102 | -0.00312 | -0.00238 | 9E-05    | 0     | 0     | 0     | 0      |
| 245                 | 0.14582 | -0.04111 | 0.00133 | -0.00259 | -0.00232 | 0.00015  | 0     | 0     | 0     | 0      |
| 250                 | 0.14746 | -0.00771 | 0.00173 | -0.00206 | -0.00226 | 0.00022  | 0     | 0     | 0     | 0      |
| 255                 | 0.14924 | 0.00768  | 0.00222 | -0.00153 | -0.0022  | 0.00028  | 0     | 0     | 0     | 0      |
| 260                 | 0.15117 | 0.00618  | 0.00283 | -0.00098 | -0.00214 | 0.00035  | 0     | 0     | 0     | 0      |
| 265                 | 0.15327 | -0.00651 | 0.00358 | -0.00043 | -0.00206 | 0.00041  | 0     | 0     | 0     | 0      |
| 270                 | 0.15552 | -0.02353 | 0.00449 | 0.00014  | -0.00198 | 0.00048  | 0     | 0     | 0     | 0      |
| 275                 | 0.15793 | -0.03863 | 0.00558 | 0.00072  | -0.0019  | 0.00054  | 0     | 0     | 0     | 0      |
| 280                 | 0.16051 | -0.04941 | 0.00685 | 0.00131  | -0.0018  | 0.0006   | 0     | 0     | 0     | 0      |
| 285                 | 0.16325 | -0.05717 | 0.00834 | 0.00192  | -0.00168 | 0.00067  | 0     | 0     | 0     | 0      |
| 290                 | 0.16617 | -0.06091 | 0.01006 | 0.00255  | -0.00155 | 0.00073  | 0     | 0     | 0     | 0      |
| 295                 | 0.16926 | -0.05462 | 0.01201 | 0.0032   | -0.00141 | 0.00079  | 0     | 0     | 0     | 0      |
| 300                 | 0.17254 | -0.03426 | 0.0142  | 0.00387  | -0.00124 | 0.00085  | 0     | 0     | 0     | 0      |
| 305                 | 0.17599 | -0.00416 | 0.01663 | 0.00457  | -0.00105 | 0.00091  | 0     | 0     | 0     | 0      |
| 310                 | 0.17961 | 0.02807  | 0.01931 | 0.00529  | -0.00084 | 0.00097  | 0     | 0     | 0     | 0      |
| 315                 | 0.18341 | 0.05924  | 0.02221 | 0.00603  | -0.0006  | 0.00102  | 0     | 0     | 0     | 0      |
| 320                 | 0.18737 | 0.09129  | 0.02534 | 0.00681  | -0.00033 | 0.00107  | 0     | 0     | 0     | 0      |
| 325                 | 0.19147 | 0.12688  | 0.02868 | 0.0076   | -2E-05   | 0.00112  | 0     | 0     | 0     | 0      |
| 330                 | 0.19568 | 0.16704  | 0.03221 | 0.00841  | 0.00032  | 0.00116  | 0     | 0     | 0     | 0      |
| 335                 | 0.20001 | 0.21052  | 0.03591 | 0.00927  | 0.0007   | 0.0012   | 0     | 0     | 0     | 0      |
| 340                 | 0.20444 | 0.25417  | 0.03977 | 0.01019  | 0.00113  | 0.00123  | 0     | 0     | 0     | 0      |
| 345                 | 0.20897 | 0.29637  | 0.04374 | 0.01121  | 0.0016   | 0.00125  | 0     | 0     | 0     | 0      |
| 350                 | 0.21361 | 0.34404  | 0.04781 | 0.01235  | 0.00211  | 0.00126  | 0     | 0     | 0     | 0      |
| 355                 | 0.21836 | 0.41178  | 0.05192 | 0.01363  | 0.00268  | 0.00126  | 0     | 0     | 0     | 0      |
| 360                 | 0.22323 | 0.51001  | 0.05605 | 0.01505  | 0.00329  | 0.00125  | 0     | 0     | 0     | 0      |
| 365                 | 0.22824 | 0.63548  | 0.06014 | 0.01663  | 0.00396  | 0.00123  | 0     | 0     | 0     | 0      |
| 370                 | 0.2334  | 0.7775   | 0.06415 | 0.01839  | 0.00469  | 0.0012   | 0     | 0     | 0     | 0      |
| 375                 | 0.23875 | 0.92674  | 0.06804 | 0.02031  | 0.00548  | 0.00114  | 0     | 0     | 0     | 0      |
| 380                 | 0.24435 | 1.07258  | 0.07178 | 0.02238  | 0.00632  | 0.00107  | 0     | 0     | 0     | 0      |
| 385                 | 0.25024 | 1.19622  | 0.07534 | 0.0246   | 0.00723  | 0.00099  | 1E-05 | 0     | 0     | 0      |
| 390                 | 0.25648 | 1.27148  | 0.07871 | 0.02695  | 0.00819  | 0.00088  | 1E-05 | 0     | 0     | 0      |
| 395                 | 0.26314 | 1.27773  | 0.08191 | 0.02941  | 0.00922  | 0.00074  | 1E-05 | 0     | 0     | 0      |
| 400                 | 0.2703  | 1.21317  | 0.08493 | 0.03197  | 0.0103   | 0.00058  | 1E-05 | 0     | 0     | 0      |
| 405                 | 0.27805 | 1.09842  | 0.08781 | 0.03461  | 0.01144  | 0.0004   | 1E-05 | 0     | 0     | 0      |
| 410                 | 0.28645 | 0.96106  | 0.09058 | 0.03732  | 0.01264  | 0.00018  | 1E-05 | 0     | 0     | 0      |
| 415                 | 0.29558 | 0.82322  | 0.09326 | 0.04009  | 0.01389  | -7E-05   | 1E-05 | 0     | 0     | 0      |
| 420                 | 0.30549 | 0.70361  | 0.09589 | 0.04293  | 0.01518  | -0.00035 | 2E-05 | 0     | 0     | 0      |
| 425                 | 0.31624 | 0.61949  | 0.09849 | 0.04579  | 0.01652  | -0.00067 | 2E-05 | 0     | 0     | 0      |
| 430                 | 0.32784 | 0.57051  | 0.10106 | 0.04865  | 0.0179   | -0.00102 | 2E-05 | 0     | 0     | 0      |
| 435                 | 0.34034 | 0.53542  | 0.10361 | 0.05148  | 0.0193   | -0.00142 | 2E-05 | 0     | 0     | 0      |
| 440                 | 0.35375 | 0.49078  | 0.10615 | 0.05423  | 0.02072  | -0.00186 | 2E-05 | 0     | 0     | 0      |
| 445                 | 0.36809 | 0.42743  | 0.10865 | 0.05688  | 0.02216  | -0.00234 | 2E-05 | 0     | 0     | 0      |

Table 1: Normalized Legendre coefficients in  $K^-p \rightarrow K^-p$  (1/10)

| Momentum<br>(MeV/c) | A1/A0   | A2/A0   | A3/A0   | A4/A0   | A5/A0   | A6/A0    | A7/A0    | A8/A0  | A9/A0 | A10/A0 |
|---------------------|---------|---------|---------|---------|---------|----------|----------|--------|-------|--------|
| 450                 | 0.38335 | 0.35685 | 0.11111 | 0.05938 | 0.02361 | -0.00287 | 3E-05    | 0      | 0     | 0      |
| 455                 | 0.39954 | 0.29473 | 0.11352 | 0.0617  | 0.02506 | -0.00345 | 3E-05    | 0      | 0     | 0      |
| 460                 | 0.41664 | 0.24563 | 0.11587 | 0.0638  | 0.02653 | -0.00407 | 3E-05    | 0      | 0     | 0      |
| 465                 | 0.43459 | 0.21189 | 0.11819 | 0.06569 | 0.02798 | -0.00474 | 3E-05    | 0      | 0     | 0      |
| 470                 | 0.45332 | 0.19982 | 0.12049 | 0.06737 | 0.0294  | -0.00546 | 3E-05    | 0      | 0     | 0      |
| 475                 | 0.47275 | 0.20898 | 0.12283 | 0.06886 | 0.03078 | -0.00623 | 4E-05    | 0      | 0     | 0      |
| 480                 | 0.49282 | 0.22837 | 0.12528 | 0.07016 | 0.03211 | -0.00705 | 4E-05    | 0      | 0     | 0      |
| 485                 | 0.51344 | 0.24427 | 0.12795 | 0.0713  | 0.03337 | -0.00791 | 4E-05    | 0      | 0     | 0      |
| 490                 | 0.53457 | 0.25093 | 0.13095 | 0.07231 | 0.03456 | -0.00882 | 4E-05    | 0      | 0     | 0      |
| 495                 | 0.55613 | 0.25424 | 0.13442 | 0.07322 | 0.03567 | -0.00977 | 4E-05    | 0      | 0     | 0      |
| 500                 | 0.57806 | 0.26108 | 0.13848 | 0.07406 | 0.03671 | -0.01076 | 4E-05    | 0      | 0     | 0      |
| 505                 | 0.60029 | 0.27305 | 0.14325 | 0.07486 | 0.03765 | -0.01179 | 5E-05    | 0      | 0     | 0      |
| 510                 | 0.62275 | 0.2865  | 0.14878 | 0.07566 | 0.03851 | -0.01285 | 5E-05    | 0      | 0     | 0      |
| 515                 | 0.64538 | 0.30095 | 0.15509 | 0.07648 | 0.03926 | -0.01394 | 5E-05    | 0      | 0     | 0      |
| 520                 | 0.66812 | 0.32366 | 0.16211 | 0.07734 | 0.03992 | -0.01506 | 5E-05    | 0      | 0     | 0      |
| 525                 | 0.69093 | 0.35704 | 0.16973 | 0.07824 | 0.04047 | -0.0162  | 5E-05    | 0      | 0     | 0      |
| 530                 | 0.71377 | 0.36827 | 0.17776 | 0.07915 | 0.04093 | -0.01737 | 4E-05    | 0      | 0     | 0      |
| 535                 | 0.7366  | 0.38051 | 0.18596 | 0.08008 | 0.0413  | -0.01855 | 4E-05    | 0      | 0     | 0      |
| 540                 | 0.75939 | 0.39356 | 0.19409 | 0.08101 | 0.04158 | -0.01975 | 4E-05    | -1E-05 | 0     | 0      |
| 545                 | 0.78211 | 0.40692 | 0.20194 | 0.08198 | 0.04178 | -0.02094 | 4E-05    | -1E-05 | 0     | 0      |
| 550                 | 0.80474 | 0.42044 | 0.20931 | 0.083   | 0.04194 | -0.02212 | 3E-05    | -1E-05 | 0     | 0      |
| 555                 | 0.82725 | 0.43387 | 0.21611 | 0.08409 | 0.04205 | -0.02328 | 3E-05    | -1E-05 | 0     | 0      |
| 560                 | 0.84963 | 0.447   | 0.2222  | 0.08529 | 0.04216 | -0.02441 | 2E-05    | -1E-05 | 0     | 0      |
| 565                 | 0.87184 | 0.45974 | 0.22759 | 0.08661 | 0.04226 | -0.0255  | 2E-05    | -1E-05 | 0     | 0      |
| 570                 | 0.89386 | 0.47209 | 0.23233 | 0.08808 | 0.04239 | -0.02654 | 1E-05    | -1E-05 | 0     | 0      |
| 575                 | 0.91567 | 0.4841  | 0.23658 | 0.08972 | 0.04255 | -0.02752 | 0        | -1E-05 | 0     | 0      |
| 580                 | 0.93726 | 0.4957  | 0.24036 | 0.09155 | 0.04277 | -0.02843 | -1E-05   | -1E-05 | 0     | 0      |
| 585                 | 0.95862 | 0.50708 | 0.24394 | 0.09359 | 0.04306 | -0.02924 | -2E-05   | -1E-05 | 0     | 0      |
| 590                 | 0.97974 | 0.51822 | 0.24738 | 0.09584 | 0.04344 | -0.02996 | -3E-05   | -1E-05 | 0     | 0      |
| 595                 | 1.00062 | 0.52933 | 0.25094 | 0.09833 | 0.04391 | -0.03055 | -4E-05   | -1E-05 | 0     | 0      |
| 600                 | 1.02125 | 0.54045 | 0.2547  | 0.10105 | 0.0445  | -0.03102 | -6E-05   | -1E-05 | 0     | 0      |
| 605                 | 1.04163 | 0.55179 | 0.25885 | 0.10403 | 0.04522 | -0.03134 | -7E-05   | -1E-05 | 0     | 0      |
| 610                 | 1.06175 | 0.56353 | 0.2635  | 0.10727 | 0.04608 | -0.03151 | -9E-05   | -1E-05 | 0     | 0      |
| 615                 | 1.08161 | 0.57592 | 0.26878 | 0.1108  | 0.0471  | -0.0315  | -0.00011 | -1E-05 | 0     | 0      |
| 620                 | 1.10122 | 0.58905 | 0.27473 | 0.1146  | 0.0483  | -0.03132 | -0.00013 | -1E-05 | 0     | 0      |
| 625                 | 1.12057 | 0.6033  | 0.28148 | 0.11868 | 0.0497  | -0.03096 | -0.00015 | -1E-05 | 0     | 0      |
| 630                 | 1.13968 | 0.61885 | 0.28905 | 0.12305 | 0.05131 | -0.03043 | -0.00017 | 0      | 0     | 0      |
| 635                 | 1.15854 | 0.63595 | 0.2975  | 0.1277  | 0.05316 | -0.02972 | -0.0002  | 0      | 0     | 0      |
| 640                 | 1.17716 | 0.65493 | 0.30687 | 0.13264 | 0.05526 | -0.02883 | -0.00022 | 0      | 0     | 0      |
| 645                 | 1.19553 | 0.67602 | 0.31718 | 0.13783 | 0.05761 | -0.02778 | -0.00025 | 0      | 0     | 0      |
| 650                 | 1.21364 | 0.69939 | 0.32841 | 0.14324 | 0.06018 | -0.02657 | -0.00028 | 0      | 0     | 0      |
| 655                 | 1.23147 | 0.72528 | 0.34057 | 0.14882 | 0.06296 | -0.02522 | -0.00031 | 0      | 0     | 0      |
| 660                 | 1.249   | 0.7539  | 0.35367 | 0.15454 | 0.06592 | -0.02375 | -0.00034 | 0      | 0     | 0      |
| 665                 | 1.26621 | 0.78533 | 0.36764 | 0.16034 | 0.06903 | -0.02217 | -0.00038 | 0      | 0     | 0      |

Table 2: Normalized Legendre coefficients in  $K^-p \rightarrow K^-p$  (2/10)

| Momentum<br>(MeV/c) | A1/A0   | A2/A0   | A3/A0   | A4/A0   | A5/A0   | A6/A0    | A7/A0    | A8/A0   | A9/A0  | A10/A0 |
|---------------------|---------|---------|---------|---------|---------|----------|----------|---------|--------|--------|
| 670                 | 1.28308 | 0.8195  | 0.3824  | 0.1662  | 0.07229 | -0.0205  | -0.00041 | 0       | 0      | 0      |
| 675                 | 1.29958 | 0.85642 | 0.39788 | 0.17209 | 0.07568 | -0.01875 | -0.00045 | 0       | 1E-05  | 0      |
| 680                 | 1.31567 | 0.89591 | 0.41398 | 0.17799 | 0.07917 | -0.01692 | -0.00049 | 1E-05   | 1E-05  | 0      |
| 685                 | 1.3313  | 0.93777 | 0.43055 | 0.1839  | 0.08278 | -0.01503 | -0.00052 | 1E-05   | 1E-05  | 0      |
| 690                 | 1.3464  | 0.98156 | 0.44745 | 0.1898  | 0.08648 | -0.01309 | -0.00056 | 1E-05   | 1E-05  | 0      |
| 695                 | 1.36092 | 1.02685 | 0.46446 | 0.19569 | 0.09029 | -0.01109 | -0.0006  | 1E-05   | 1E-05  | 0      |
| 700                 | 1.3748  | 1.07309 | 0.48139 | 0.20155 | 0.09418 | -0.00906 | -0.00064 | 2E-05   | 1E-05  | 0      |
| 705                 | 1.38798 | 1.11974 | 0.49805 | 0.20738 | 0.09815 | -0.00698 | -0.00068 | 2E-05   | 1E-05  | 0      |
| 710                 | 1.4004  | 1.16608 | 0.51421 | 0.21317 | 0.10219 | -0.00489 | -0.00072 | 2E-05   | 1E-05  | 0      |
| 715                 | 1.41199 | 1.2115  | 0.52966 | 0.21892 | 0.10629 | -0.00279 | -0.00076 | 2E-05   | 1E-05  | 0      |
| 720                 | 1.4227  | 1.25536 | 0.54424 | 0.22461 | 0.11042 | -0.00069 | -0.0008  | 3E-05   | 2E-05  | 0      |
| 725                 | 1.43247 | 1.29714 | 0.55781 | 0.23025 | 0.11459 | 0.00139  | -0.00083 | 3E-05   | 2E-05  | 0      |
| 730                 | 1.44128 | 1.33634 | 0.57029 | 0.23586 | 0.11881 | 0.00347  | -0.00087 | 4E-05   | 2E-05  | 0      |
| 735                 | 1.4491  | 1.37258 | 0.58161 | 0.24145 | 0.12307 | 0.00557  | -0.0009  | 4E-05   | 2E-05  | 0      |
| 740                 | 1.4559  | 1.40563 | 0.59178 | 0.24704 | 0.1274  | 0.0077   | -0.00092 | 4E-05   | 2E-05  | 0      |
| 745                 | 1.46166 | 1.43537 | 0.60085 | 0.25266 | 0.1318  | 0.00989  | -0.00094 | 5E-05   | 2E-05  | 0      |
| 750                 | 1.4664  | 1.46184 | 0.60893 | 0.25834 | 0.1363  | 0.01213  | -0.00096 | 5E-05   | 3E-05  | 0      |
| 755                 | 1.47012 | 1.48507 | 0.61613 | 0.2641  | 0.14092 | 0.01446  | -0.00097 | 6E-05   | 3E-05  | 0      |
| 760                 | 1.47283 | 1.50532 | 0.62261 | 0.27    | 0.14569 | 0.01687  | -0.00098 | 6E-05   | 3E-05  | 0      |
| 765                 | 1.47454 | 1.52274 | 0.62849 | 0.27606 | 0.15063 | 0.01938  | -0.00097 | 7E-05   | 3E-05  | 0      |
| 770                 | 1.47527 | 1.5377  | 0.634   | 0.2823  | 0.15572 | 0.02196  | -0.00096 | 7E-05   | 3E-05  | 0      |
| 775                 | 1.47506 | 1.55045 | 0.63926 | 0.28875 | 0.16095 | 0.02458  | -0.00094 | 8E-05   | 3E-05  | 0      |
| 780                 | 1.47395 | 1.56132 | 0.64445 | 0.29542 | 0.16628 | 0.02721  | -0.0009  | 8E-05   | 3E-05  | 0      |
| 785                 | 1.47197 | 1.57062 | 0.64973 | 0.30235 | 0.17174 | 0.02983  | -0.00086 | 9E-05   | 4E-05  | 0      |
| 790                 | 1.46919 | 1.5787  | 0.65524 | 0.30957 | 0.1773  | 0.03242  | -0.0008  | 9E-05   | 4E-05  | 0      |
| 795                 | 1.46566 | 1.58579 | 0.66108 | 0.31709 | 0.18297 | 0.03496  | -0.00072 | 0.0001  | 4E-05  | 0      |
| 800                 | 1.46143 | 1.59213 | 0.66731 | 0.32494 | 0.18871 | 0.03743  | -0.00063 | 0.0001  | 4E-05  | 0      |
| 805                 | 1.45658 | 1.59801 | 0.67402 | 0.33312 | 0.19452 | 0.03981  | -0.00052 | 0.00011 | 4E-05  | 0      |
| 810                 | 1.45114 | 1.60371 | 0.68124 | 0.34165 | 0.20038 | 0.04209  | -0.00039 | 0.00011 | 4E-05  | 0      |
| 815                 | 1.44519 | 1.60936 | 0.68893 | 0.35054 | 0.20629 | 0.04424  | -0.00023 | 0.00011 | 4E-05  | 0      |
| 820                 | 1.43878 | 1.61515 | 0.69704 | 0.35982 | 0.21224 | 0.04625  | -6E-05   | 0.00012 | 4E-05  | 0      |
| 825                 | 1.43195 | 1.62131 | 0.70553 | 0.36949 | 0.21824 | 0.04813  | 0.00015  | 0.00012 | 4E-05  | 0      |
| 830                 | 1.42477 | 1.62791 | 0.71427 | 0.37956 | 0.22429 | 0.04984  | 0.00038  | 0.00012 | 3E-05  | 0      |
| 835                 | 1.41729 | 1.63504 | 0.72318 | 0.39006 | 0.23038 | 0.05138  | 0.00064  | 0.00012 | 3E-05  | 0      |
| 840                 | 1.40956 | 1.64282 | 0.73218 | 0.401   | 0.23651 | 0.05274  | 0.00093  | 0.00012 | 3E-05  | 0      |
| 845                 | 1.40161 | 1.65132 | 0.74124 | 0.41239 | 0.2427  | 0.05393  | 0.00126  | 0.00012 | 2E-05  | 0      |
| 850                 | 1.3935  | 1.66056 | 0.7503  | 0.42424 | 0.24895 | 0.05496  | 0.00162  | 0.00011 | 2E-05  | 0      |
| 855                 | 1.38526 | 1.67054 | 0.75937 | 0.43656 | 0.25527 | 0.05582  | 0.00201  | 0.00011 | 1E-05  | 0      |
| 860                 | 1.37693 | 1.68128 | 0.76851 | 0.44938 | 0.26166 | 0.05654  | 0.00245  | 0.0001  | 1E-05  | 0      |
| 865                 | 1.36855 | 1.69275 | 0.77776 | 0.46269 | 0.26815 | 0.05712  | 0.00292  | 9E-05   | 0      | 0      |
| 870                 | 1.36017 | 1.70495 | 0.78724 | 0.47652 | 0.27478 | 0.05759  | 0.00343  | 8E-05   | -1E-05 | 0      |
| 875                 | 1.35182 | 1.71783 | 0.79705 | 0.49087 | 0.28156 | 0.05797  | 0.00399  | 7E-05   | -2E-05 | 0      |
| 880                 | 1.34355 | 1.73135 | 0.80728 | 0.50576 | 0.28853 | 0.05828  | 0.00458  | 5E-05   | -3E-05 | 0      |
| 885                 | 1.33538 | 1.74545 | 0.81803 | 0.52118 | 0.29569 | 0.05854  | 0.00522  | 4E-05   | -4E-05 | 0      |

Table 3: Normalized Legendre coefficients in  $K^-p \rightarrow K^-p$  (3/10)

| Momentum<br>(MeV/c) | A1/A0   | A2/A0   | A3/A0   | A4/A0   | A5/A0   | A6/A0    | A7/A0   | A8/A0    | A9/A0    | A10/A0 |
|---------------------|---------|---------|---------|---------|---------|----------|---------|----------|----------|--------|
| 890                 | 1.32737 | 1.76009 | 0.82938 | 0.53712 | 0.30306 | 0.05876  | 0.00589 | 1E-05    | -5E-05   | 0      |
| 895                 | 1.31955 | 1.77516 | 0.8414  | 0.55357 | 0.31064 | 0.05896  | 0.00661 | -1E-05   | -7E-05   | 0      |
| 900                 | 1.31195 | 1.79066 | 0.85422 | 0.57052 | 0.31846 | 0.05916  | 0.00737 | -4E-05   | -8E-05   | 0      |
| 905                 | 1.30462 | 1.80645 | 0.86774 | 0.58794 | 0.32651 | 0.05937  | 0.00817 | -7E-05   | -0.0001  | 0      |
| 910                 | 1.29758 | 1.82248 | 0.88204 | 0.60577 | 0.33479 | 0.05957  | 0.009   | -0.0001  | -0.00012 | 0      |
| 915                 | 1.29087 | 1.83865 | 0.89711 | 0.62396 | 0.34327 | 0.05975  | 0.00987 | -0.00014 | -0.00014 | 0      |
| 920                 | 1.28451 | 1.85489 | 0.91289 | 0.64244 | 0.35194 | 0.05992  | 0.01077 | -0.00019 | -0.00016 | 0      |
| 925                 | 1.27854 | 1.87113 | 0.92941 | 0.66113 | 0.36077 | 0.06006  | 0.01169 | -0.00024 | -0.00018 | 0      |
| 930                 | 1.27299 | 1.88729 | 0.94663 | 0.67995 | 0.36971 | 0.06017  | 0.01263 | -0.00029 | -0.00021 | 0      |
| 935                 | 1.26789 | 1.90333 | 0.9646  | 0.69881 | 0.37872 | 0.06024  | 0.01358 | -0.00034 | -0.00024 | 0      |
| 940                 | 1.26327 | 1.91917 | 0.98329 | 0.71765 | 0.38775 | 0.06027  | 0.01453 | -0.00041 | -0.00026 | 0      |
| 945                 | 1.25914 | 1.93478 | 1.00276 | 0.73636 | 0.39678 | 0.06025  | 0.01548 | -0.00047 | -0.00029 | 0      |
| 950                 | 1.25553 | 1.95014 | 1.02309 | 0.75486 | 0.40576 | 0.06017  | 0.01642 | -0.00054 | -0.00032 | 0      |
| 955                 | 1.25247 | 1.96526 | 1.04444 | 0.77305 | 0.41466 | 0.06003  | 0.01733 | -0.00062 | -0.00036 | 0      |
| 960                 | 1.24996 | 1.98014 | 1.06695 | 0.79084 | 0.42344 | 0.05981  | 0.0182  | -0.0007  | -0.00039 | 0      |
| 965                 | 1.24804 | 1.99479 | 1.09078 | 0.80815 | 0.43208 | 0.0595   | 0.01902 | -0.00079 | -0.00042 | 0      |
| 970                 | 1.24672 | 2.00926 | 1.11616 | 0.82491 | 0.44055 | 0.0591   | 0.01979 | -0.00088 | -0.00046 | 0      |
| 975                 | 1.24601 | 2.02357 | 1.14324 | 0.84102 | 0.44882 | 0.05858  | 0.02051 | -0.00098 | -0.00049 | 0      |
| 980                 | 1.24594 | 2.03775 | 1.17221 | 0.8564  | 0.45685 | 0.05794  | 0.02117 | -0.00108 | -0.00053 | 0      |
| 985                 | 1.2465  | 2.0518  | 1.20312 | 0.87098 | 0.46461 | 0.05716  | 0.02178 | -0.00118 | -0.00057 | 0      |
| 990                 | 1.24771 | 2.06568 | 1.23594 | 0.88468 | 0.47206 | 0.05623  | 0.02233 | -0.00129 | -0.0006  | 0      |
| 995                 | 1.24956 | 2.0793  | 1.27044 | 0.89743 | 0.47913 | 0.05514  | 0.02282 | -0.0014  | -0.00064 | 0      |
| 1000                | 1.25203 | 2.09256 | 1.30631 | 0.90917 | 0.48577 | 0.05388  | 0.02322 | -0.00151 | -0.00067 | 0      |
| 1005                | 1.25511 | 2.10532 | 1.34305 | 0.91985 | 0.49192 | 0.05246  | 0.02355 | -0.00162 | -0.0007  | 0      |
| 1010                | 1.2588  | 2.11731 | 1.37985 | 0.92939 | 0.49755 | 0.05085  | 0.02379 | -0.00174 | -0.00073 | 0      |
| 1015                | 1.26308 | 2.12833 | 1.41594 | 0.93779 | 0.5026  | 0.04907  | 0.02393 | -0.00185 | -0.00076 | 0      |
| 1020                | 1.26795 | 2.13814 | 1.45041 | 0.94503 | 0.50705 | 0.0471   | 0.02399 | -0.00197 | -0.00078 | 0      |
| 1025                | 1.27338 | 2.14656 | 1.48242 | 0.95109 | 0.51088 | 0.04496  | 0.02395 | -0.00208 | -0.0008  | 0      |
| 1030                | 1.27938 | 2.15331 | 1.51104 | 0.95597 | 0.51404 | 0.04264  | 0.02382 | -0.00219 | -0.00082 | 0      |
| 1035                | 1.28592 | 2.15832 | 1.53575 | 0.95964 | 0.51651 | 0.04015  | 0.0236  | -0.00229 | -0.00083 | 0      |
| 1040                | 1.293   | 2.16155 | 1.55614 | 0.96211 | 0.51826 | 0.03747  | 0.02327 | -0.00239 | -0.00083 | 0      |
| 1045                | 1.30061 | 2.163   | 1.57204 | 0.96334 | 0.51926 | 0.03463  | 0.02286 | -0.00249 | -0.00083 | 0      |
| 1050                | 1.30872 | 2.16272 | 1.58343 | 0.96336 | 0.51949 | 0.03161  | 0.02235 | -0.00257 | -0.00082 | 0      |
| 1055                | 1.31732 | 2.16081 | 1.5905  | 0.96221 | 0.51898 | 0.02843  | 0.02175 | -0.00264 | -0.00081 | 0      |
| 1060                | 1.32638 | 2.15741 | 1.59355 | 0.95996 | 0.51774 | 0.0251   | 0.02108 | -0.00271 | -0.00078 | 0      |
| 1065                | 1.33587 | 2.15274 | 1.59306 | 0.95665 | 0.51581 | 0.02165  | 0.02035 | -0.00275 | -0.00074 | 0      |
| 1070                | 1.34578 | 2.14696 | 1.58939 | 0.95236 | 0.51321 | 0.01808  | 0.01956 | -0.00278 | -0.00069 | 0      |
| 1075                | 1.35609 | 2.14027 | 1.58309 | 0.94716 | 0.50999 | 0.01443  | 0.01874 | -0.0028  | -0.00063 | 0      |
| 1080                | 1.36676 | 2.13286 | 1.57454 | 0.94113 | 0.50619 | 0.01071  | 0.01787 | -0.00279 | -0.00056 | 0      |
| 1085                | 1.37779 | 2.12492 | 1.56429 | 0.93433 | 0.50184 | 0.00695  | 0.01698 | -0.00275 | -0.00047 | 0      |
| 1090                | 1.38914 | 2.11665 | 1.55271 | 0.92686 | 0.49697 | 0.00317  | 0.01608 | -0.00269 | -0.00037 | 0      |
| 1095                | 1.40076 | 2.10821 | 1.54028 | 0.91878 | 0.49165 | -0.00062 | 0.01518 | -0.0026  | -0.00025 | 0      |
| 1100                | 1.41261 | 2.09974 | 1.52734 | 0.9102  | 0.4859  | -0.00439 | 0.01429 | -0.00247 | -0.00011 | 0      |
| 1105                | 1.42462 | 2.09138 | 1.51429 | 0.90121 | 0.47978 | -0.00813 | 0.01344 | -0.00231 | 5E-05    | 0      |

Table 4: Normalized Legendre coefficients in  $K^-p \rightarrow K^-p$  (4/10)

| Momentum<br>(MeV/c) | A1/A0   | A2/A0   | A3/A0   | A4/A0   | A5/A0   | A6/A0    | A7/A0   | A8/A0    | A9/A0   | A10/A0 |
|---------------------|---------|---------|---------|---------|---------|----------|---------|----------|---------|--------|
| 1110                | 1.43677 | 2.08324 | 1.50142 | 0.89189 | 0.47332 | -0.01183 | 0.01264 | -0.0021  | 0.00023 | 0      |
| 1115                | 1.44898 | 2.07537 | 1.48901 | 0.88234 | 0.46657 | -0.01546 | 0.0119  | -0.00185 | 0.00044 | 0      |
| 1120                | 1.46122 | 2.06783 | 1.4773  | 0.87264 | 0.45958 | -0.019   | 0.01126 | -0.00154 | 0.00066 | 0      |
| 1125                | 1.47343 | 2.06063 | 1.46643 | 0.86287 | 0.45238 | -0.02245 | 0.01072 | -0.00118 | 0.00091 | 0      |
| 1130                | 1.48556 | 2.05378 | 1.45653 | 0.85308 | 0.44503 | -0.02577 | 0.01029 | -0.00076 | 0.00119 | 0      |
| 1135                | 1.49758 | 2.04726 | 1.44767 | 0.84333 | 0.43758 | -0.02897 | 0.00999 | -0.00028 | 0.00149 | 0      |
| 1140                | 1.50943 | 2.04106 | 1.43987 | 0.83366 | 0.43008 | -0.03202 | 0.00984 | 0.00027  | 0.00183 | 0      |
| 1145                | 1.52109 | 2.03518 | 1.43314 | 0.82413 | 0.4226  | -0.03489 | 0.00984 | 0.00089  | 0.00219 | 0      |
| 1150                | 1.53252 | 2.0296  | 1.42743 | 0.81479 | 0.4152  | -0.03756 | 0.01    | 0.00159  | 0.00258 | 0      |
| 1155                | 1.54367 | 2.02432 | 1.42269 | 0.8057  | 0.4079  | -0.04002 | 0.01034 | 0.00238  | 0.003   | 0      |
| 1160                | 1.5545  | 2.01935 | 1.41883 | 0.79694 | 0.40076 | -0.04224 | 0.01087 | 0.00325  | 0.00345 | 0      |
| 1165                | 1.56496 | 2.01471 | 1.41576 | 0.78856 | 0.3938  | -0.04419 | 0.01158 | 0.00421  | 0.00393 | 0      |
| 1170                | 1.57503 | 2.01042 | 1.41337 | 0.78064 | 0.38707 | -0.04587 | 0.01249 | 0.00526  | 0.00444 | 0      |
| 1175                | 1.58469 | 2.1965  | 1.41155 | 0.77321 | 0.38061 | -0.04724 | 0.01361 | 0.00642  | 0.00498 | 0      |
| 1180                | 1.5939  | 2.00299 | 1.41016 | 0.76633 | 0.37444 | -0.04829 | 0.01496 | 0.00767  | 0.00554 | 0      |
| 1185                | 1.60265 | 1.9999  | 1.40908 | 0.76005 | 0.3686  | -0.049   | 0.01653 | 0.00902  | 0.00613 | 0      |
| 1190                | 1.61092 | 1.99724 | 1.40818 | 0.7544  | 0.36312 | -0.04934 | 0.01834 | 0.01048  | 0.00674 | 1E-05  |
| 1195                | 1.6187  | 1.99499 | 1.40729 | 0.7494  | 0.35805 | -0.0493  | 0.02039 | 0.01204  | 0.00737 | 1E-05  |
| 1200                | 1.62597 | 1.99317 | 1.40635 | 0.74509 | 0.35343 | -0.04887 | 0.02268 | 0.01371  | 0.00801 | 1E-05  |
| 1205                | 1.63272 | 1.99173 | 1.40521 | 0.74151 | 0.34931 | -0.04801 | 0.02523 | 0.01547  | 0.00866 | 1E-05  |
| 1210                | 1.63895 | 1.99063 | 1.40379 | 0.73867 | 0.34575 | -0.0467  | 0.02803 | 0.01733  | 0.00932 | 1E-05  |
| 1215                | 1.64465 | 1.98982 | 1.40203 | 0.73662 | 0.34282 | -0.0449  | 0.03109 | 0.01929  | 0.00997 | 1E-05  |
| 1220                | 1.64984 | 1.98925 | 1.39991 | 0.73538 | 0.34058 | -0.04259 | 0.03443 | 0.02134  | 0.01062 | 2E-05  |
| 1225                | 1.65456 | 1.98885 | 1.39743 | 0.73499 | 0.33906 | -0.03974 | 0.03803 | 0.02346  | 0.01124 | 2E-05  |
| 1230                | 1.65885 | 1.98857 | 1.39463 | 0.73546 | 0.33833 | -0.03633 | 0.0419  | 0.02566  | 0.01185 | 2E-05  |
| 1235                | 1.66276 | 1.9884  | 1.39163 | 0.73683 | 0.33842 | -0.03235 | 0.04604 | 0.02791  | 0.01241 | 3E-05  |
| 1240                | 1.66633 | 1.98832 | 1.38853 | 0.7391  | 0.33937 | -0.0278  | 0.05045 | 0.03022  | 0.01294 | 3E-05  |
| 1245                | 1.66959 | 1.98831 | 1.38547 | 0.74229 | 0.34116 | -0.02272 | 0.05512 | 0.03256  | 0.01341 | 3E-05  |
| 1250                | 1.67261 | 1.98841 | 1.38262 | 0.74638 | 0.34381 | -0.01713 | 0.06004 | 0.03492  | 0.01381 | 4E-05  |
| 1255                | 1.67544 | 1.98864 | 1.38016 | 0.75139 | 0.34735 | -0.01103 | 0.06523 | 0.03731  | 0.01416 | 4E-05  |
| 1260                | 1.67811 | 1.98907 | 1.37827 | 0.75735 | 0.35181 | -0.00444 | 0.07068 | 0.03972  | 0.01444 | 4E-05  |
| 1265                | 1.6807  | 1.98975 | 1.37713 | 0.76427 | 0.35722 | 0.00267  | 0.07642 | 0.04215  | 0.01467 | 5E-05  |
| 1270                | 1.68325 | 1.99077 | 1.37693 | 0.77218 | 0.36363 | 0.0103   | 0.08243 | 0.04461  | 0.01486 | 5E-05  |
| 1275                | 1.68581 | 1.99224 | 1.37785 | 0.7811  | 0.37107 | 0.01845  | 0.08874 | 0.0471   | 0.01499 | 5E-05  |
| 1280                | 1.68844 | 1.99422 | 1.38006 | 0.79104 | 0.37957 | 0.02713  | 0.09535 | 0.04962  | 0.01508 | 6E-05  |
| 1285                | 1.69117 | 1.99685 | 1.38376 | 0.80203 | 0.38917 | 0.03633  | 0.10226 | 0.05216  | 0.01514 | 6E-05  |
| 1290                | 1.69404 | 2.00021 | 1.38909 | 0.81409 | 0.39987 | 0.04604  | 0.10947 | 0.05472  | 0.01516 | 7E-05  |
| 1295                | 1.69705 | 2.00443 | 1.39628 | 0.8272  | 0.41163 | 0.05625  | 0.11694 | 0.05729  | 0.01514 | 7E-05  |
| 1300                | 1.70021 | 2.00965 | 1.4055  | 0.84135 | 0.42441 | 0.06693  | 0.12467 | 0.05985  | 0.01508 | 8E-05  |
| 1305                | 1.70353 | 2.01597 | 1.41698 | 0.85652 | 0.43817 | 0.07806  | 0.13261 | 0.0624   | 0.015   | 8E-05  |
| 1310                | 1.70703 | 2.02352 | 1.43096 | 0.87269 | 0.45284 | 0.08962  | 0.14074 | 0.06492  | 0.01488 | 8E-05  |
| 1315                | 1.7107  | 2.0324  | 1.44765 | 0.88983 | 0.46839 | 0.10157  | 0.14903 | 0.0674   | 0.01473 | 9E-05  |
| 1320                | 1.71455 | 2.04268 | 1.46721 | 0.90794 | 0.48476 | 0.11389  | 0.15746 | 0.06983  | 0.01456 | 9E-05  |
| 1325                | 1.7186  | 2.0544  | 1.48977 | 0.92699 | 0.50191 | 0.12657  | 0.166   | 0.0722   | 0.01435 | 9E-05  |

Table 5: Normalized Legendre coefficients in  $K^-p \rightarrow K^-p$  (5/10)

| Momentum<br>(MeV/c) | A1/A0   | A2/A0   | A3/A0   | A4/A0   | A5/A0   | A6/A0   | A7/A0   | A8/A0   | A9/A0    | A10/A0   |
|---------------------|---------|---------|---------|---------|---------|---------|---------|---------|----------|----------|
| 1330                | 1.72283 | 2.06752 | 1.51535 | 0.94694 | 0.5198  | 0.13956 | 0.17463 | 0.07448 | 0.01412  | 0.0001   |
| 1335                | 1.72726 | 2.082   | 1.54394 | 0.96778 | 0.53838 | 0.15284 | 0.18333 | 0.07669 | 0.01386  | 0.0001   |
| 1340                | 1.73188 | 2.09761 | 1.57517 | 0.98947 | 0.55762 | 0.16638 | 0.1921  | 0.07879 | 0.01357  | 0.0001   |
| 1345                | 1.73669 | 2.11416 | 1.60872 | 1.01198 | 0.57747 | 0.18014 | 0.2009  | 0.08078 | 0.01327  | 0.0001   |
| 1350                | 1.74168 | 2.13141 | 1.64411 | 1.03528 | 0.5979  | 0.19409 | 0.20973 | 0.08266 | 0.01294  | 0.0001   |
| 1355                | 1.74687 | 2.14911 | 1.68074 | 1.05933 | 0.61886 | 0.2082  | 0.21857 | 0.0844  | 0.01259  | 0.0001   |
| 1360                | 1.75224 | 2.16699 | 1.71798 | 1.08412 | 0.64031 | 0.22244 | 0.22739 | 0.086   | 0.01222  | 0.0001   |
| 1365                | 1.7578  | 2.1849  | 1.75528 | 1.1096  | 0.66221 | 0.23678 | 0.23619 | 0.08744 | 0.01183  | 0.0001   |
| 1370                | 1.76355 | 2.20267 | 1.79212 | 1.13575 | 0.68453 | 0.25118 | 0.24495 | 0.08872 | 0.01142  | 0.0001   |
| 1375                | 1.76948 | 2.22025 | 1.82818 | 1.16253 | 0.70722 | 0.26561 | 0.25364 | 0.08982 | 0.011    | 9E-05    |
| 1380                | 1.7756  | 2.23755 | 1.863   | 1.18992 | 0.73024 | 0.28004 | 0.26226 | 0.09073 | 0.01056  | 9E-05    |
| 1385                | 1.78191 | 2.25468 | 1.89666 | 1.21789 | 0.75355 | 0.29444 | 0.27078 | 0.09145 | 0.0101   | 8E-05    |
| 1390                | 1.78839 | 2.27153 | 1.92896 | 1.2464  | 0.77711 | 0.30879 | 0.2792  | 0.09196 | 0.00964  | 7E-05    |
| 1395                | 1.79506 | 2.28807 | 1.95988 | 1.2754  | 0.80087 | 0.32308 | 0.28749 | 0.0923  | 0.00916  | 6E-05    |
| 1400                | 1.80191 | 2.3043  | 1.9895  | 1.30486 | 0.8248  | 0.33732 | 0.29565 | 0.09246 | 0.00868  | 5E-05    |
| 1405                | 1.80892 | 2.32031 | 2.01814 | 1.33474 | 0.84883 | 0.35149 | 0.30367 | 0.09248 | 0.00819  | 4E-05    |
| 1410                | 1.81611 | 2.33611 | 2.04597 | 1.36499 | 0.87294 | 0.36561 | 0.31154 | 0.09237 | 0.00769  | 3E-05    |
| 1415                | 1.82347 | 2.35183 | 2.0734  | 1.39557 | 0.89707 | 0.37966 | 0.31924 | 0.09214 | 0.0072   | 1E-05    |
| 1420                | 1.83098 | 2.36761 | 2.10085 | 1.42644 | 0.92119 | 0.39364 | 0.32677 | 0.09182 | 0.0067   | -1E-05   |
| 1425                | 1.83866 | 2.3837  | 2.12881 | 1.45756 | 0.94524 | 0.40755 | 0.33411 | 0.09141 | 0.00621  | -3E-05   |
| 1430                | 1.8465  | 2.40026 | 2.15761 | 1.48889 | 0.96918 | 0.42139 | 0.34125 | 0.09094 | 0.00572  | -5E-05   |
| 1435                | 1.85448 | 2.41772 | 2.18799 | 1.52038 | 0.99296 | 0.43515 | 0.34818 | 0.09043 | 0.00524  | -7E-05   |
| 1440                | 1.86261 | 2.43632 | 2.22012 | 1.55198 | 1.01656 | 0.44883 | 0.35489 | 0.08987 | 0.00476  | -0.0001  |
| 1445                | 1.87088 | 2.4564  | 2.25442 | 1.58366 | 1.03994 | 0.46243 | 0.36137 | 0.08928 | 0.00429  | -0.00013 |
| 1450                | 1.87926 | 2.47821 | 2.29095 | 1.61534 | 1.06307 | 0.47594 | 0.36761 | 0.08864 | 0.00384  | -0.00016 |
| 1455                | 1.88775 | 2.50203 | 2.32979 | 1.64699 | 1.08592 | 0.48935 | 0.37359 | 0.08797 | 0.00338  | -0.0002  |
| 1460                | 1.89633 | 2.52791 | 2.37059 | 1.67854 | 1.10846 | 0.50267 | 0.37931 | 0.08724 | 0.00294  | -0.00023 |
| 1465                | 1.90498 | 2.55575 | 2.41275 | 1.70994 | 1.13066 | 0.51587 | 0.38474 | 0.08647 | 0.0025   | -0.00027 |
| 1470                | 1.9137  | 2.58528 | 2.45552 | 1.74115 | 1.1525  | 0.52897 | 0.38989 | 0.08565 | 0.00207  | -0.00031 |
| 1475                | 1.92247 | 2.61583 | 2.49765 | 1.77211 | 1.17394 | 0.54196 | 0.39473 | 0.08478 | 0.00164  | -0.00036 |
| 1480                | 1.93128 | 2.64682 | 2.53822 | 1.80277 | 1.19496 | 0.55482 | 0.39926 | 0.08386 | 0.00122  | -0.00041 |
| 1485                | 1.9401  | 2.67749 | 2.57631 | 1.83306 | 1.21553 | 0.56756 | 0.40347 | 0.08288 | 0.00081  | -0.00046 |
| 1490                | 1.94894 | 2.70719 | 2.61131 | 1.86296 | 1.23562 | 0.58015 | 0.40734 | 0.08184 | 0.0004   | -0.00051 |
| 1495                | 1.95779 | 2.73518 | 2.64271 | 1.89239 | 1.2552  | 0.59258 | 0.41088 | 0.08076 | 0        | -0.00057 |
| 1500                | 1.96663 | 2.76107 | 2.67053 | 1.92133 | 1.27426 | 0.60481 | 0.4141  | 0.07962 | -0.0004  | -0.00063 |
| 1505                | 1.97546 | 2.78466 | 2.6951  | 1.94971 | 1.29278 | 0.61681 | 0.41699 | 0.07844 | -0.0008  | -0.00069 |
| 1510                | 1.98427 | 2.80574 | 2.71662 | 1.9775  | 1.31074 | 0.62856 | 0.41955 | 0.07722 | -0.00119 | -0.00076 |
| 1515                | 1.99305 | 2.82446 | 2.73579 | 2.00463 | 1.3281  | 0.64003 | 0.42179 | 0.07595 | -0.00158 | -0.00083 |
| 1520                | 2.00181 | 2.84098 | 2.7532  | 2.03108 | 1.34486 | 0.65118 | 0.42371 | 0.07465 | -0.00196 | -0.0009  |
| 1525                | 2.01052 | 2.85555 | 2.76943 | 2.05678 | 1.36098 | 0.66199 | 0.42531 | 0.07332 | -0.00235 | -0.00098 |
| 1530                | 2.01919 | 2.86842 | 2.78501 | 2.08169 | 1.37646 | 0.67243 | 0.4266  | 0.07196 | -0.00273 | -0.00106 |
| 1535                | 2.0278  | 2.87996 | 2.80048 | 2.10576 | 1.39126 | 0.68247 | 0.42757 | 0.07057 | -0.0031  | -0.00114 |
| 1540                | 2.03635 | 2.8903  | 2.8161  | 2.12896 | 1.40537 | 0.6921  | 0.42823 | 0.06915 | -0.00348 | -0.00123 |
| 1545                | 2.04483 | 2.89977 | 2.83218 | 2.15129 | 1.41881 | 0.7013  | 0.42858 | 0.06771 | -0.00385 | -0.00132 |

Table 6: Normalized Legendre coefficients in  $K^-p \rightarrow K^-p$  (6/10)

| Momentum<br>(MeV/c) | A1/A0   | A2/A0   | A3/A0   | A4/A0   | A5/A0   | A6/A0   | A7/A0   | A8/A0   | A9/A0    | A10/A0   |
|---------------------|---------|---------|---------|---------|---------|---------|---------|---------|----------|----------|
| 1550                | 2.05324 | 2.90864 | 2.84896 | 2.17277 | 1.43157 | 0.71009 | 0.42864 | 0.06625 | -0.00422 | -0.00141 |
| 1555                | 2.06156 | 2.91713 | 2.86654 | 2.1934  | 1.44367 | 0.71845 | 0.42841 | 0.06476 | -0.00459 | -0.00151 |
| 1560                | 2.06979 | 2.92546 | 2.88488 | 2.2132  | 1.45512 | 0.7264  | 0.4279  | 0.06325 | -0.00494 | -0.00161 |
| 1565                | 2.07792 | 2.93381 | 2.90387 | 2.23216 | 1.46592 | 0.73394 | 0.42712 | 0.06171 | -0.00529 | -0.00171 |
| 1570                | 2.08595 | 2.94231 | 2.92325 | 2.25032 | 1.47609 | 0.74106 | 0.42607 | 0.06015 | -0.00563 | -0.00181 |
| 1575                | 2.09387 | 2.95113 | 2.94275 | 2.26766 | 1.48563 | 0.74777 | 0.42477 | 0.05856 | -0.00596 | -0.00191 |
| 1580                | 2.10166 | 2.96017 | 2.96173 | 2.28421 | 1.49455 | 0.75406 | 0.42322 | 0.05695 | -0.00628 | -0.00201 |
| 1585                | 2.10933 | 2.96958 | 2.97993 | 2.29998 | 1.50287 | 0.75995 | 0.42143 | 0.05532 | -0.00659 | -0.00211 |
| 1590                | 2.11686 | 2.97912 | 2.99666 | 2.31496 | 1.51058 | 0.76542 | 0.41941 | 0.05366 | -0.00689 | -0.00221 |
| 1595                | 2.12426 | 2.98872 | 3.01163 | 2.32918 | 1.5177  | 0.77048 | 0.41717 | 0.05198 | -0.00716 | -0.0023  |
| 1600                | 2.1315  | 2.99818 | 3.0245  | 2.34264 | 1.52424 | 0.77514 | 0.41471 | 0.05028 | -0.00743 | -0.0024  |
| 1605                | 2.13859 | 3.00725 | 3.03509 | 2.35536 | 1.53021 | 0.77939 | 0.41204 | 0.04855 | -0.00768 | -0.00249 |
| 1610                | 2.14551 | 3.01569 | 3.04332 | 2.36733 | 1.53561 | 0.78324 | 0.40917 | 0.0468  | -0.00791 | -0.00258 |
| 1615                | 2.15227 | 3.02325 | 3.04931 | 2.37858 | 1.54046 | 0.78668 | 0.40611 | 0.04503 | -0.00811 | -0.00267 |
| 1620                | 2.15884 | 3.02974 | 3.05324 | 2.38911 | 1.54476 | 0.78972 | 0.40287 | 0.04324 | -0.0083  | -0.00275 |
| 1625                | 2.16523 | 3.03506 | 3.0554  | 2.39893 | 1.54852 | 0.79235 | 0.39945 | 0.04142 | -0.00847 | -0.00282 |
| 1630                | 2.17143 | 3.03914 | 3.05609 | 2.40805 | 1.55175 | 0.79459 | 0.39587 | 0.03958 | -0.00862 | -0.0029  |
| 1635                | 2.17743 | 3.04206 | 3.05566 | 2.41649 | 1.55446 | 0.79642 | 0.39212 | 0.03772 | -0.00874 | -0.00296 |
| 1640                | 2.18323 | 3.0438  | 3.05428 | 2.42425 | 1.55667 | 0.79786 | 0.38823 | 0.03583 | -0.00884 | -0.00302 |
| 1645                | 2.18883 | 3.04456 | 3.05224 | 2.43135 | 1.5584  | 0.79893 | 0.38421 | 0.03394 | -0.0089  | -0.00308 |
| 1650                | 2.19425 | 3.04449 | 3.04972 | 2.43784 | 1.55969 | 0.79964 | 0.38008 | 0.03203 | -0.00894 | -0.00312 |
| 1655                | 2.19949 | 3.04374 | 3.04683 | 2.44372 | 1.56058 | 0.80001 | 0.37586 | 0.03012 | -0.00894 | -0.00316 |
| 1660                | 2.20457 | 3.04245 | 3.04363 | 2.44904 | 1.5611  | 0.80007 | 0.37157 | 0.02822 | -0.0089  | -0.00318 |
| 1665                | 2.20949 | 3.04076 | 3.04018 | 2.4538  | 1.56127 | 0.79983 | 0.36722 | 0.02633 | -0.00882 | -0.00319 |
| 1670                | 2.21426 | 3.03876 | 3.03649 | 2.45804 | 1.56113 | 0.79931 | 0.36285 | 0.02445 | -0.00869 | -0.00319 |
| 1675                | 2.21889 | 3.03657 | 3.03256 | 2.46178 | 1.56073 | 0.79853 | 0.35847 | 0.0226  | -0.00851 | -0.00317 |
| 1680                | 2.22339 | 3.03424 | 3.02844 | 2.46505 | 1.56008 | 0.79752 | 0.35409 | 0.02078 | -0.00828 | -0.00314 |
| 1685                | 2.22778 | 3.03182 | 3.02406 | 2.46788 | 1.55922 | 0.79629 | 0.34975 | 0.019   | -0.00799 | -0.00309 |
| 1690                | 2.23204 | 3.02936 | 3.01948 | 2.47029 | 1.5582  | 0.79487 | 0.34545 | 0.01726 | -0.00764 | -0.00302 |
| 1695                | 2.2362  | 3.02689 | 3.01476 | 2.47235 | 1.55707 | 0.79332 | 0.34124 | 0.0156  | -0.00723 | -0.00294 |
| 1700                | 2.24024 | 3.02446 | 3.00998 | 2.47413 | 1.55589 | 0.79171 | 0.33714 | 0.01403 | -0.00674 | -0.00283 |
| 1705                | 2.24417 | 3.0221  | 3.00522 | 2.47568 | 1.55472 | 0.79009 | 0.33318 | 0.01259 | -0.00618 | -0.00269 |
| 1710                | 2.24799 | 3.01984 | 3.00059 | 2.47707 | 1.55362 | 0.78852 | 0.3294  | 0.01129 | -0.00554 | -0.00253 |
| 1715                | 2.2517  | 3.01771 | 2.99623 | 2.47837 | 1.55264 | 0.78708 | 0.32582 | 0.01016 | -0.00482 | -0.00234 |
| 1720                | 2.2553  | 3.01574 | 2.99226 | 2.47962 | 1.55186 | 0.78581 | 0.32248 | 0.00922 | -0.004   | -0.00212 |
| 1725                | 2.25879 | 3.01395 | 2.98884 | 2.48091 | 1.55133 | 0.78478 | 0.31941 | 0.00851 | -0.00308 | -0.00186 |
| 1730                | 2.26217 | 3.01237 | 2.98611 | 2.48228 | 1.55111 | 0.78405 | 0.31663 | 0.00804 | -0.00207 | -0.00158 |
| 1735                | 2.26543 | 3.01101 | 2.98419 | 2.48381 | 1.55125 | 0.78368 | 0.31418 | 0.00784 | -0.00095 | -0.00125 |
| 1740                | 2.2686  | 3.00988 | 2.98319 | 2.48555 | 1.55181 | 0.78373 | 0.31209 | 0.00793 | 0.00028  | -0.00089 |
| 1745                | 2.27167 | 3.00897 | 2.98323 | 2.48753 | 1.55279 | 0.7842  | 0.31036 | 0.00833 | 0.00164  | -0.00048 |
| 1750                | 2.27466 | 3.00828 | 2.98436 | 2.48976 | 1.5542  | 0.78513 | 0.309   | 0.00904 | 0.00312  | -4E-05   |
| 1755                | 2.27759 | 3.00777 | 2.9866  | 2.49229 | 1.55605 | 0.78653 | 0.30801 | 0.01008 | 0.00473  | 0.00046  |
| 1760                | 2.28046 | 3.00743 | 2.98993 | 2.49512 | 1.55834 | 0.78842 | 0.30742 | 0.01146 | 0.00649  | 0.00101  |
| 1765                | 2.28329 | 3.00722 | 2.99427 | 2.49831 | 1.56109 | 0.7908  | 0.30721 | 0.0132  | 0.0084   | 0.00161  |

Table 7: Normalized Legendre coefficients in  $K^-p \rightarrow K^-p$  (7/10)

| Momentum<br>(MeV/c) | A1/A0   | A2/A0   | A3/A0   | A4/A0   | A5/A0   | A6/A0   | A7/A0   | A8/A0   | A9/A0   | A10/A0  |
|---------------------|---------|---------|---------|---------|---------|---------|---------|---------|---------|---------|
| 1770                | 2.2861  | 3.00712 | 2.99948 | 2.50185 | 1.56429 | 0.79371 | 0.30741 | 0.0153  | 0.01047 | 0.00226 |
| 1775                | 2.28889 | 3.00709 | 3.00539 | 2.5058  | 1.56796 | 0.79716 | 0.30802 | 0.01778 | 0.0127  | 0.00297 |
| 1780                | 2.29169 | 3.1971  | 3.01177 | 2.51016 | 1.5721  | 0.80117 | 0.30905 | 0.02065 | 0.01511 | 0.00375 |
| 1785                | 2.2945  | 3.00713 | 3.01836 | 2.51497 | 1.57672 | 0.80575 | 0.3105  | 0.02392 | 0.01769 | 0.00458 |
| 1790                | 2.29733 | 3.00727 | 3.02501 | 2.52024 | 1.58182 | 0.81092 | 0.31238 | 0.0276  | 0.02047 | 0.00549 |
| 1795                | 2.30019 | 3.00743 | 3.03129 | 2.52598 | 1.58741 | 0.81667 | 0.3147  | 0.03168 | 0.02343 | 0.00646 |
| 1800                | 2.30308 | 3.00769 | 3.03701 | 2.53218 | 1.5935  | 0.82299 | 0.31748 | 0.03616 | 0.02657 | 0.0075  |
| 1805                | 2.30599 | 3.1981  | 3.04192 | 2.53883 | 1.60008 | 0.82989 | 0.3207  | 0.04101 | 0.0299  | 0.00861 |
| 1810                | 2.30894 | 3.00875 | 3.04579 | 2.54593 | 1.60716 | 0.83734 | 0.3244  | 0.04625 | 0.03341 | 0.00979 |
| 1815                | 2.31191 | 3.00975 | 3.04841 | 2.55348 | 1.61474 | 0.84535 | 0.32856 | 0.05185 | 0.0371  | 0.01104 |
| 1820                | 2.31492 | 3.01122 | 3.04963 | 2.56148 | 1.62284 | 0.85391 | 0.3332  | 0.05781 | 0.04098 | 0.01236 |
| 1825                | 2.31795 | 3.01333 | 3.04935 | 2.56991 | 1.63144 | 0.86302 | 0.33833 | 0.06413 | 0.04503 | 0.01375 |
| 1830                | 2.32102 | 3.01624 | 3.04762 | 2.57878 | 1.64056 | 0.87266 | 0.34395 | 0.07078 | 0.04926 | 0.01521 |
| 1835                | 2.32413 | 3.02014 | 3.04457 | 2.58808 | 1.6502  | 0.88283 | 0.35007 | 0.07777 | 0.05367 | 0.01675 |
| 1840                | 2.32727 | 3.02528 | 3.04081 | 2.59781 | 1.66037 | 0.89353 | 0.35671 | 0.08509 | 0.05826 | 0.01836 |
| 1845                | 2.33044 | 3.03168 | 3.03673 | 2.60797 | 1.67106 | 0.90475 | 0.36386 | 0.09272 | 0.06301 | 0.02005 |
| 1850                | 2.33366 | 3.03949 | 3.03328 | 2.61854 | 1.68229 | 0.91647 | 0.37154 | 0.10066 | 0.06795 | 0.02181 |
| 1855                | 2.33691 | 3.04874 | 3.03143 | 2.62953 | 1.69405 | 0.9287  | 0.37975 | 0.1089  | 0.07305 | 0.02365 |
| 1860                | 2.3402  | 3.0594  | 3.03217 | 2.64094 | 1.70635 | 0.94143 | 0.3885  | 0.11743 | 0.07833 | 0.02557 |
| 1865                | 2.34353 | 3.07137 | 3.03635 | 2.65275 | 1.71919 | 0.95466 | 0.3978  | 0.12624 | 0.08378 | 0.02756 |
| 1870                | 2.3469  | 3.08454 | 3.04459 | 2.66497 | 1.73259 | 0.96837 | 0.40765 | 0.13533 | 0.0894  | 0.02963 |
| 1875                | 2.35032 | 3.09878 | 3.05724 | 2.67759 | 1.74653 | 0.98256 | 0.41807 | 0.14468 | 0.09518 | 0.03179 |
| 1880                | 2.35378 | 3.11396 | 3.07431 | 2.69061 | 1.76103 | 0.99722 | 0.42906 | 0.15429 | 0.10114 | 0.03402 |
| 1885                | 2.35728 | 3.12996 | 3.09565 | 2.70402 | 1.77609 | 1.01235 | 0.44063 | 0.16415 | 0.10726 | 0.03633 |
| 1890                | 2.36083 | 3.1466  | 3.12083 | 2.71781 | 1.7917  | 1.02793 | 0.45277 | 0.17425 | 0.11354 | 0.03872 |
| 1895                | 2.3644  | 3.16367 | 3.14918 | 2.73195 | 1.80781 | 1.04392 | 0.46544 | 0.18455 | 0.11996 | 0.04119 |
| 1900                | 2.36801 | 3.181   | 3.18008 | 2.74642 | 1.82439 | 1.06029 | 0.4786  | 0.19504 | 0.1265  | 0.04371 |
| 1905                | 2.37163 | 3.19834 | 3.21275 | 2.76118 | 1.84138 | 1.07698 | 0.4922  | 0.20568 | 0.13315 | 0.0463  |
| 1910                | 2.37525 | 3.2154  | 3.24639 | 2.77619 | 1.85874 | 1.09395 | 0.50619 | 0.21644 | 0.13988 | 0.04894 |
| 1915                | 2.37887 | 3.23188 | 3.28016 | 2.79144 | 1.87643 | 1.11116 | 0.52052 | 0.2273  | 0.14668 | 0.05162 |
| 1920                | 2.38247 | 3.24747 | 3.31324 | 2.80688 | 1.89439 | 1.12858 | 0.53516 | 0.23822 | 0.15352 | 0.05433 |
| 1925                | 2.38605 | 3.26188 | 3.34488 | 2.82248 | 1.91258 | 1.14615 | 0.55006 | 0.24919 | 0.16039 | 0.05707 |
| 1930                | 2.3896  | 3.27487 | 3.37443 | 2.83822 | 1.93096 | 1.16384 | 0.56516 | 0.26017 | 0.16726 | 0.05983 |
| 1935                | 2.3931  | 3.28629 | 3.40141 | 2.85406 | 1.94947 | 1.18161 | 0.58043 | 0.27113 | 0.17413 | 0.0626  |
| 1940                | 2.39655 | 3.29596 | 3.42532 | 2.86997 | 1.96808 | 1.1994  | 0.59582 | 0.28205 | 0.18096 | 0.06538 |
| 1945                | 2.39994 | 3.30388 | 3.44597 | 2.88593 | 1.98673 | 1.21718 | 0.61129 | 0.2929  | 0.18774 | 0.06815 |
| 1950                | 2.40326 | 3.31012 | 3.46328 | 2.90189 | 2.00539 | 1.23491 | 0.62678 | 0.30364 | 0.19445 | 0.07092 |
| 1955                | 2.4065  | 3.31482 | 3.47731 | 2.91783 | 2.02399 | 1.25255 | 0.64225 | 0.31426 | 0.20108 | 0.07366 |
| 1960                | 2.40965 | 3.31816 | 3.48822 | 2.93371 | 2.04251 | 1.27005 | 0.65766 | 0.32472 | 0.20759 | 0.07638 |
| 1965                | 2.41269 | 3.32044 | 3.49632 | 2.94951 | 2.06089 | 1.28736 | 0.67296 | 0.335   | 0.21398 | 0.07907 |
| 1970                | 2.41563 | 3.32179 | 3.50179 | 2.96519 | 2.07908 | 1.30446 | 0.68811 | 0.34507 | 0.22022 | 0.08172 |
| 1975                | 2.41845 | 3.32254 | 3.50506 | 2.98073 | 2.09704 | 1.32129 | 0.70305 | 0.35489 | 0.22629 | 0.08432 |
| 1980                | 2.42114 | 3.32293 | 3.50649 | 2.99609 | 2.11473 | 1.33781 | 0.71775 | 0.36445 | 0.23218 | 0.08686 |
| 1985                | 2.42369 | 3.32318 | 3.50645 | 3.01123 | 2.13209 | 1.35398 | 0.73216 | 0.3737  | 0.23786 | 0.08934 |

Table 8: Normalized Legendre coefficients in  $K^-p \rightarrow K^-p$  (8/10)



| Momentum<br>(MeV/c) | A1/A0   | A2/A0   | A3/A0   | A4/A0   | A5/A0   | A6/A0   | A7/A0   | A8/A0   | A9/A0   | A10/A0  |
|---------------------|---------|---------|---------|---------|---------|---------|---------|---------|---------|---------|
| 1990                | 2.4261  | 3.32346 | 3.50529 | 3.02615 | 2.1491  | 1.36979 | 0.74625 | 0.38265 | 0.24332 | 0.09175 |
| 1995                | 2.42837 | 3.3239  | 3.50335 | 3.04085 | 2.16577 | 1.38523 | 0.76001 | 0.3913  | 0.24858 | 0.0941  |
| 2000                | 2.43052 | 3.3246  | 3.50095 | 3.05532 | 2.18212 | 1.40032 | 0.77347 | 0.39966 | 0.25362 | 0.09637 |
| 2005                | 2.43254 | 3.32561 | 3.49838 | 3.0696  | 2.19817 | 1.4151  | 0.78662 | 0.40776 | 0.25847 | 0.09857 |
| 2010                | 2.43445 | 3.32696 | 3.49592 | 3.08368 | 2.21393 | 1.42957 | 0.79948 | 0.41561 | 0.26313 | 0.10071 |
| 2015                | 2.43626 | 3.32865 | 3.49379 | 3.09757 | 2.22941 | 1.44376 | 0.81205 | 0.42322 | 0.2676  | 0.10277 |
| 2020                | 2.43797 | 3.33067 | 3.4922  | 3.11129 | 2.24465 | 1.45768 | 0.82434 | 0.43061 | 0.2719  | 0.10477 |
| 2025                | 2.43959 | 3.33296 | 3.49131 | 3.12484 | 2.25964 | 1.47135 | 0.83637 | 0.4378  | 0.27602 | 0.10669 |
| 2030                | 2.44113 | 3.3355  | 3.49125 | 3.13823 | 2.27442 | 1.48479 | 0.84813 | 0.4448  | 0.27998 | 0.10855 |
| 2035                | 2.4426  | 3.33826 | 3.49211 | 3.15148 | 2.28899 | 1.49802 | 0.85963 | 0.45163 | 0.28378 | 0.11033 |
| 2040                | 2.444   | 3.34111 | 3.49372 | 3.16458 | 2.30338 | 1.51106 | 0.87089 | 0.45831 | 0.28743 | 0.11205 |
| 2045                | 2.44535 | 3.34405 | 3.49616 | 3.17756 | 2.31759 | 1.52392 | 0.88191 | 0.46485 | 0.29094 | 0.11369 |
| 2050                | 2.44665 | 3.34702 | 3.49935 | 3.19042 | 2.33166 | 1.53664 | 0.8927  | 0.47126 | 0.29431 | 0.11527 |
| 2055                | 2.44791 | 3.34996 | 3.50318 | 3.20317 | 2.34559 | 1.54921 | 0.90327 | 0.47758 | 0.29755 | 0.11678 |
| 2060                | 2.44914 | 3.35283 | 3.50751 | 3.21581 | 2.3594  | 1.56167 | 0.91363 | 0.4838  | 0.30066 | 0.11821 |
| 2065                | 2.45034 | 3.35558 | 3.51224 | 3.22837 | 2.37312 | 1.57403 | 0.92377 | 0.48995 | 0.30366 | 0.11957 |
| 2070                | 2.45152 | 3.35816 | 3.51725 | 3.24084 | 2.38675 | 1.58631 | 0.93373 | 0.49604 | 0.30655 | 0.12087 |
| 2075                | 2.4527  | 3.36053 | 3.52245 | 3.25325 | 2.40031 | 1.59853 | 0.94349 | 0.50209 | 0.30933 | 0.12209 |
| 2080                | 2.45388 | 3.36265 | 3.52782 | 3.26559 | 2.41382 | 1.61071 | 0.95306 | 0.50811 | 0.31202 | 0.12324 |
| 2085                | 2.45506 | 3.36448 | 3.53335 | 3.27788 | 2.4273  | 1.62286 | 0.96247 | 0.51413 | 0.31462 | 0.12433 |
| 2090                | 2.45626 | 3.36599 | 3.53911 | 3.29012 | 2.44076 | 1.63501 | 0.97171 | 0.52015 | 0.31713 | 0.12534 |
| 2095                | 2.45747 | 3.36713 | 3.54518 | 3.30232 | 2.4542  | 1.64714 | 0.98078 | 0.52617 | 0.31957 | 0.12627 |
| 2100                | 2.4587  | 3.36785 | 3.5517  | 3.31448 | 2.46763 | 1.65927 | 0.98971 | 0.53219 | 0.32192 | 0.12714 |
| 2105                | 2.45995 | 3.3681  | 3.55882 | 3.32661 | 2.48105 | 1.67138 | 0.99848 | 0.5382  | 0.32419 | 0.12793 |
| 2110                | 2.46121 | 3.36785 | 3.56668 | 3.3387  | 2.49446 | 1.68349 | 1.1971  | 0.5442  | 0.32639 | 0.12864 |
| 2115                | 2.46248 | 3.36709 | 3.57531 | 3.35077 | 2.50787 | 1.69558 | 1.01559 | 0.55019 | 0.32851 | 0.12928 |
| 2120                | 2.46378 | 3.36582 | 3.58467 | 3.3628  | 2.52126 | 1.70766 | 1.02394 | 0.55616 | 0.33056 | 0.12983 |
| 2125                | 2.4651  | 3.36413 | 3.59451 | 3.37482 | 2.53466 | 1.71973 | 1.03217 | 0.56211 | 0.33254 | 0.13031 |
| 2130                | 2.46643 | 3.36214 | 3.60448 | 3.38682 | 2.54806 | 1.73178 | 1.04027 | 0.56805 | 0.33445 | 0.1307  |
| 2135                | 2.46779 | 3.36001 | 3.61413 | 3.39879 | 2.56146 | 1.74382 | 1.04825 | 0.57395 | 0.33629 | 0.13101 |
| 2140                | 2.46917 | 3.35797 | 3.62309 | 3.41076 | 2.57486 | 1.75585 | 1.05612 | 0.57983 | 0.33807 | 0.13124 |
| 2145                | 2.47056 | 3.35605 | 3.63094 | 3.42271 | 2.58827 | 1.76786 | 1.06388 | 0.58568 | 0.33978 | 0.13138 |
| 2150                | 2.47199 | 3.35441 | 3.63757 | 3.43466 | 2.60169 | 1.77986 | 1.07154 | 0.59149 | 0.34143 | 0.13143 |
| 2155                | 2.47343 | 3.3531  | 3.64301 | 3.4466  | 2.61512 | 1.79184 | 1.0791  | 0.59726 | 0.34301 | 0.1314  |
| 2160                | 2.4749  | 3.35214 | 3.64737 | 3.45854 | 2.62857 | 1.8038  | 1.08657 | 0.60299 | 0.34454 | 0.13127 |
| 2165                | 2.47639 | 3.35154 | 3.65085 | 3.47048 | 2.64203 | 1.81575 | 1.09396 | 0.60868 | 0.34602 | 0.13106 |
| 2170                | 2.47791 | 3.3513  | 3.65368 | 3.48243 | 2.65551 | 1.82768 | 1.10126 | 0.61432 | 0.34743 | 0.13075 |
| 2175                | 2.47945 | 3.35147 | 3.65608 | 3.49439 | 2.66901 | 1.83959 | 1.10849 | 0.61991 | 0.3488  | 0.13035 |
| 2180                | 2.48102 | 3.35223 | 3.65849 | 3.50635 | 2.68254 | 1.85148 | 1.11565 | 0.62544 | 0.35011 | 0.12985 |
| 2185                | 2.48262 | 3.35353 | 3.66096 | 3.51833 | 2.69609 | 1.86335 | 1.12274 | 0.63092 | 0.35137 | 0.12925 |
| 2190                | 2.48425 | 3.35566 | 3.66378 | 3.53033 | 2.70967 | 1.8752  | 1.12977 | 0.63634 | 0.35259 | 0.12856 |
| 2195                | 2.4859  | 3.3589  | 3.66741 | 3.54235 | 2.72328 | 1.88704 | 1.13675 | 0.64169 | 0.35375 | 0.12777 |
| 2200                | 2.48758 | 3.36365 | 3.6723  | 3.55439 | 2.73693 | 1.89885 | 1.14368 | 0.64697 | 0.35488 | 0.12688 |
| 2205                | 2.4893  | 3.3704  | 3.67895 | 3.56646 | 2.7506  | 1.91064 | 1.15057 | 0.65219 | 0.35596 | 0.12589 |

Table 9: Normalized Legendre coefficients in  $K^-p \rightarrow K^-p$  (9/10)

| Momentum<br>(MeV/c) | A1/A0   | A2/A0   | A3/A0   | A4/A0   | A5/A0   | A6/A0   | A7/A0   | A8/A0   | A9/A0   | A10/A0  |
|---------------------|---------|---------|---------|---------|---------|---------|---------|---------|---------|---------|
| 2210                | 2.49104 | 3.37963 | 3.68794 | 3.57856 | 2.76432 | 1.9224  | 1.15742 | 0.65733 | 0.357   | 0.12479 |
| 2215                | 2.49282 | 3.39172 | 3.69969 | 3.59069 | 2.77807 | 1.93415 | 1.16424 | 0.6624  | 0.358   | 0.1236  |
| 2220                | 2.49463 | 3.40674 | 3.7144  | 3.60285 | 2.79187 | 1.94587 | 1.17103 | 0.66738 | 0.35896 | 0.12229 |
| 2225                | 2.49647 | 3.42421 | 3.73174 | 3.61506 | 2.80571 | 1.95756 | 1.17779 | 0.67228 | 0.35989 | 0.12088 |
| 2230                | 2.49835 | 3.44326 | 3.75104 | 3.62731 | 2.8196  | 1.96923 | 1.18454 | 0.6771  | 0.36078 | 0.11936 |
| 2235                | 2.50025 | 3.46231 | 3.77088 | 3.6396  | 2.83354 | 1.98088 | 1.19128 | 0.68183 | 0.36165 | 0.11773 |
| 2240                | 2.5022  | 3.48011 | 3.78998 | 3.65194 | 2.84753 | 1.9925  | 1.19802 | 0.68646 | 0.36248 | 0.11598 |
| 2245                | 2.50418 | 3.49581 | 3.80762 | 3.66433 | 2.86157 | 2.1941  | 1.20475 | 0.691   | 0.36328 | 0.11413 |
| 2250                | 2.5062  | 3.50913 | 3.82344 | 3.67678 | 2.87567 | 2.01566 | 1.21149 | 0.69544 | 0.36406 | 0.11216 |
| 2255                | 2.50825 | 3.52022 | 3.83754 | 3.68929 | 2.88983 | 2.0272  | 1.21823 | 0.69977 | 0.36481 | 0.11008 |
| 2260                | 2.51034 | 3.52949 | 3.85027 | 3.70185 | 2.90405 | 2.03872 | 1.225   | 0.704   | 0.36554 | 0.10788 |
| 2265                | 2.51247 | 3.53741 | 3.86203 | 3.71448 | 2.91833 | 2.0502  | 1.23178 | 0.70812 | 0.36624 | 0.10556 |
| 2270                | 2.51464 | 3.54443 | 3.87322 | 3.72718 | 2.93268 | 2.06165 | 1.23859 | 0.71213 | 0.36693 | 0.10313 |
| 2275                | 2.51685 | 3.5509  | 3.88415 | 3.73994 | 2.94709 | 2.07308 | 1.24543 | 0.71603 | 0.3676  | 0.10057 |
| 2280                | 2.5191  | 3.55707 | 3.89503 | 3.75278 | 2.96158 | 2.08447 | 1.25231 | 0.71981 | 0.36826 | 0.09789 |
| 2285                | 2.52139 | 3.56312 | 3.90596 | 3.7657  | 2.97614 | 2.09584 | 1.25923 | 0.72346 | 0.3689  | 0.09509 |
| 2290                | 2.52372 | 3.56913 | 3.91699 | 3.77869 | 2.99077 | 2.10717 | 1.26619 | 0.72699 | 0.36952 | 0.09217 |
| 2295                | 2.52609 | 3.57517 | 3.92809 | 3.79175 | 3.00546 | 2.11846 | 1.27319 | 0.73041 | 0.37014 | 0.08914 |
| 2300                | 2.5285  | 3.58122 | 3.93914 | 3.80486 | 3.0202  | 2.12972 | 1.28021 | 0.73371 | 0.37074 | 0.08599 |
| 2305                | 2.53093 | 3.58725 | 3.95002 | 3.81803 | 3.03497 | 2.14093 | 1.28726 | 0.73689 | 0.37132 | 0.08276 |
| 2310                | 2.5334  | 3.5932  | 3.96055 | 3.83123 | 3.04978 | 2.15209 | 1.29431 | 0.73998 | 0.37189 | 0.07943 |
| 2315                | 2.53589 | 3.599   | 3.97054 | 3.84446 | 3.06461 | 2.16319 | 1.30137 | 0.74296 | 0.37245 | 0.07603 |
| 2320                | 2.5384  | 3.60457 | 3.97979 | 3.85771 | 3.07944 | 2.17424 | 1.30842 | 0.74584 | 0.37299 | 0.07255 |
| 2325                | 2.54093 | 3.60985 | 3.98817 | 3.87097 | 3.09426 | 2.18523 | 1.31545 | 0.74863 | 0.37351 | 0.06901 |
| 2330                | 2.54348 | 3.61467 | 3.99541 | 3.88423 | 3.10907 | 2.19615 | 1.32246 | 0.75133 | 0.37402 | 0.06542 |
| 2335                | 2.54603 | 3.61904 | 4.00148 | 3.89749 | 3.12385 | 2.20701 | 1.32944 | 0.75395 | 0.3745  | 0.06178 |
| 2340                | 2.5486  | 3.6229  | 4.00632 | 3.91072 | 3.1386  | 2.21778 | 1.33638 | 0.75649 | 0.37498 | 0.0581  |
| 2345                | 2.55117 | 3.62622 | 4.00994 | 3.92392 | 3.15329 | 2.22848 | 1.34326 | 0.75895 | 0.37543 | 0.0544  |
| 2350                | 2.55375 | 3.62901 | 4.01239 | 3.93709 | 3.16793 | 2.2391  | 1.35009 | 0.76134 | 0.37586 | 0.05068 |
| 2355                | 2.55632 | 3.6313  | 4.01379 | 3.9502  | 3.1825  | 2.24963 | 1.35684 | 0.76366 | 0.37628 | 0.04694 |
| 2360                | 2.5589  | 3.6331  | 4.01428 | 3.96326 | 3.19698 | 2.26006 | 1.36353 | 0.76592 | 0.37668 | 0.0432  |
| 2365                | 2.56146 | 3.63449 | 4.01403 | 3.97626 | 3.21137 | 2.2704  | 1.37012 | 0.76813 | 0.37705 | 0.03947 |
| 2370                | 2.56401 | 3.63552 | 4.0132  | 3.98917 | 3.22566 | 2.28065 | 1.37663 | 0.77027 | 0.37741 | 0.03576 |
| 2375                | 2.56655 | 3.63624 | 4.01196 | 4.002   | 3.23983 | 2.29079 | 1.38303 | 0.77237 | 0.37774 | 0.03206 |

Table 10: Normalized Legendre coefficients in  $K^-p \rightarrow K^-p$  (10/10)

| Momentum<br>(MeV/c) | A1/A0    | A2/A0    | A3/A0    | A4/A0    | A5/A0    | A6/A0    | A7/A0 | A8/A0 |
|---------------------|----------|----------|----------|----------|----------|----------|-------|-------|
| 235                 | -0.30755 | 0        | -0.04859 | -0.01348 | -9e-05   | 5e-05    | 0     | 0     |
| 240                 | -0.3041  | 0        | -0.03549 | -0.01096 | -8e-05   | 5e-05    | 0     | 0     |
| 245                 | -0.30451 | 0        | -0.02232 | -0.00843 | -8e-05   | 4e-05    | 0     | 0     |
| 250                 | -0.31028 | 0        | -0.00899 | -0.00585 | -7e-05   | 4e-05    | 0     | 0     |
| 255                 | -0.32259 | 0        | 0.00462  | -0.00319 | -6e-05   | 4e-05    | 0     | 0     |
| 260                 | -0.34185 | 0        | 0.01859  | -0.00041 | -5e-05   | 3e-05    | 0     | 0     |
| 265                 | -0.36746 | 0        | 0.03305  | 0.00251  | -4e-05   | 3e-05    | 0     | 0     |
| 270                 | -0.39766 | 0        | 0.04809  | 0.00563  | -3e-05   | 2e-05    | 0     | 0     |
| 275                 | -0.42975 | 0        | 0.0638   | 0.00898  | -2e-05   | 2e-05    | 0     | 0     |
| 280                 | -0.46069 | 1e-05    | 0.08023  | 0.0126   | 0        | 1e-05    | 0     | 0     |
| 285                 | -0.48736 | 5e-05    | 0.0973   | 0.0165   | 1e-05    | 0        | 0     | 0     |
| 290                 | -0.50729 | 2e-04    | 0.11487  | 0.02069  | 4e-05    | -1e-05   | 0     | 0     |
| 295                 | -0.51855 | 0.00063  | 0.13282  | 0.02519  | 6e-05    | -3e-05   | 0     | 0     |
| 300                 | -0.52024 | 0.00134  | 0.15096  | 0.02998  | 9e-05    | -4e-05   | 0     | 0     |
| 305                 | -0.51207 | 0.00124  | 0.16892  | 0.03503  | 0.00013  | -6e-05   | 0     | 0     |
| 310                 | -0.49468 | -0.002   | 0.18618  | 0.04031  | 0.00016  | -9e-05   | 0     | 0     |
| 315                 | -0.46892 | -0.00933 | 0.20212  | 0.04568  | 0.00021  | -0.00011 | 0     | 0     |
| 320                 | -0.43609 | -0.01586 | 0.21604  | 0.05101  | 0.00026  | -0.00014 | 0     | 0     |
| 325                 | -0.3973  | -0.01303 | 0.22726  | 0.05617  | 0.00031  | -0.00017 | 0     | 0     |
| 330                 | -0.35379 | 0.00167  | 0.23511  | 0.06107  | 0.00037  | -0.00021 | 0     | 0     |
| 335                 | -0.3067  | 0.0219   | 0.23911  | 0.06576  | 0.00044  | -0.00024 | 0     | 0     |
| 340                 | -0.25739 | 0.04678  | 0.23878  | 0.07033  | 5e-04    | -0.00028 | 0     | 0     |
| 345                 | -0.20755 | 0.09094  | 0.23367  | 0.07488  | 0.00057  | -0.00032 | 0     | 0     |
| 350                 | -0.15908 | 0.17482  | 0.22334  | 0.0795   | 0.00064  | -0.00037 | 0     | 0     |
| 355                 | -0.11446 | 0.30682  | 0.20753  | 0.08421  | 0.00071  | -0.00041 | 0     | 0     |
| 360                 | -0.07625 | 0.48075  | 0.1861   | 0.08906  | 0.00078  | -0.00045 | 0     | 0     |
| 365                 | -0.04747 | 0.68345  | 0.1593   | 0.09421  | 0.00083  | -0.00049 | 0     | 0     |
| 370                 | -0.03064 | 0.90388  | 0.1275   | 0.09983  | 0.00088  | -0.00052 | 0     | 0     |
| 375                 | -0.02812 | 1.13397  | 0.09104  | 0.10608  | 0.00091  | -0.00054 | 0     | 0     |
| 380                 | -0.04087 | 1.3636   | 0.05039  | 0.11311  | 0.00092  | -0.00056 | 0     | 0     |
| 385                 | -0.06879 | 1.57657  | 0.00644  | 0.12093  | 9e-04    | -0.00056 | 0     | 0     |
| 390                 | -0.10972 | 1.75346  | -0.03978 | 0.1295   | 0.00085  | -0.00054 | 0     | 0     |
| 395                 | -0.16022 | 1.87981  | -0.08707 | 0.13859  | 0.00076  | -5e-04   | 0     | 0     |
| 400                 | -0.21553 | 1.9509   | -0.1342  | 0.14795  | 0.00063  | -0.00043 | 0     | 0     |
| 405                 | -0.27043 | 1.97287  | -0.17995 | 0.15732  | 0.00043  | -0.00034 | 0     | 0     |
| 410                 | -0.32009 | 1.95458  | -0.22323 | 0.16643  | 0.00017  | -2e-04   | 0     | 0     |
| 415                 | -0.36095 | 1.89945  | -0.26354 | 0.1749   | -0.00016 | -2e-05   | 0     | 0     |
| 420                 | -0.3912  | 1.80489  | -0.30052 | 0.18232  | -0.00058 | 2e-04    | 0     | 0     |
| 425                 | -0.4106  | 1.68228  | -0.3338  | 0.18828  | -0.0011  | 0.00048  | 0     | 0     |
| 430                 | -0.42021 | 1.56358  | -0.36315 | 0.19246  | -0.00172 | 0.00082  | 0     | 0     |
| 435                 | -0.42128 | 1.47378  | -0.38888 | 0.19478  | -0.00244 | 0.00123  | 0     | 0     |
| 440                 | -0.415   | 1.42688  | -0.41138 | 0.19524  | -0.00329 | 0.0017   | 0     | 0     |
| 445                 | -0.40201 | 1.39998  | -0.43103 | 0.19376  | -0.00425 | 0.00225  | 0     | 0     |
| 450                 | -0.38247 | 1.36801  | -0.44826 | 0.19036  | -0.00534 | 0.00286  | 0     | 0     |
| 455                 | -0.35589 | 1.33185  | -0.46368 | 0.18542  | -0.00653 | 0.00355  | 0     | 0     |

Table 11: Normalized Legendre coefficients in  $K^- p \rightarrow \bar{K}^0 n$  (1/5)

| Momentum<br>(MeV/c) | A1/A0    | A2/A0   | A3/A0    | A4/A0   | A5/A0    | A6/A0   | A7/A0 | A8/A0 |
|---------------------|----------|---------|----------|---------|----------|---------|-------|-------|
| 460                 | -0.3216  | 1.29215 | -0.47787 | 0.17941 | -0.00782 | 0.0043  | 0     | 0     |
| 465                 | -0.27917 | 1.2499  | -0.49102 | 0.1727  | -0.00918 | 0.0051  | 0     | 0     |
| 470                 | -0.22973 | 1.20597 | -0.50321 | 0.16567 | -0.0106  | 0.00594 | 0     | 0     |
| 475                 | -0.17713 | 1.16167 | -0.5145  | 0.15865 | -0.01204 | 0.00682 | 0     | 0     |
| 480                 | -0.12841 | 1.11813 | -0.52493 | 0.15196 | -0.01349 | 0.00771 | 0     | 0     |
| 485                 | -0.09149 | 1.07666 | -0.53436 | 0.14575 | -0.01489 | 0.0086  | 0     | 0     |
| 490                 | -0.07028 | 1.03839 | -0.5426  | 0.14013 | -0.01618 | 0.00944 | 0     | 0     |
| 495                 | -0.06296 | 1.00433 | -0.54947 | 0.13518 | -0.0173  | 0.01021 | 0     | 0     |
| 500                 | -0.06366 | 0.97503 | -0.55477 | 0.13101 | -0.01819 | 0.01087 | 0     | 0     |
| 505                 | -0.06664 | 0.95085 | -0.55833 | 0.12773 | -0.0188  | 0.0114  | 0     | 0     |
| 510                 | -0.06771 | 0.93169 | -0.55996 | 0.12544 | -0.01906 | 0.01175 | 0     | 0     |
| 515                 | -0.06476 | 0.91724 | -0.55947 | 0.12423 | -0.01891 | 0.01191 | 0     | 0     |
| 520                 | -0.05705 | 0.90697 | -0.55703 | 0.12437 | -0.01831 | 0.01186 | 0     | 0     |
| 525                 | -0.04488 | 0.90021 | -0.55318 | 0.12594 | -0.01736 | 0.01179 | 0     | 0     |
| 530                 | -0.02927 | 0.8963  | -0.54843 | 0.12893 | -0.01624 | 0.01196 | 0     | 0     |
| 535                 | -0.01183 | 0.8945  | -0.5433  | 0.13334 | -0.01512 | 0.0126  | 0     | 0     |
| 540                 | 0.00596  | 0.89424 | -0.53831 | 0.13906 | -0.01414 | 0.01394 | 0     | 0     |
| 545                 | 0.02306  | 0.89492 | -0.5339  | 0.1458  | -0.0134  | 0.01611 | 0     | 0     |
| 550                 | 0.039    | 0.89617 | -0.53048 | 0.15329 | -0.01298 | 0.01915 | 0     | 0     |
| 555                 | 0.05391  | 0.89758 | -0.52847 | 0.16125 | -0.01294 | 0.02316 | 0     | 0     |
| 560                 | 0.06806  | 0.89897 | -0.52824 | 0.16947 | -0.01334 | 0.02816 | 0     | 0     |
| 565                 | 0.08166  | 0.90012 | -0.52974 | 0.17794 | -0.01416 | 0.03398 | 0     | 0     |
| 570                 | 0.09478  | 0.90105 | -0.53283 | 0.18651 | -0.01529 | 0.0403  | 0     | 0     |
| 575                 | 0.10746  | 0.9017  | -0.53736 | 0.19494 | -0.01659 | 0.04682 | 0     | 0     |
| 580                 | 0.11985  | 0.90216 | -0.54318 | 0.20297 | -0.01795 | 0.05322 | 0     | 0     |
| 585                 | 0.13218  | 0.90248 | -0.55002 | 0.21039 | -0.01909 | 0.05908 | 0     | 0     |
| 590                 | 0.14481  | 0.90282 | -0.55752 | 0.21698 | -0.01964 | 0.06395 | 0     | 0     |
| 595                 | 0.15769  | 0.90328 | -0.56531 | 0.22255 | -0.01921 | 0.06734 | 0     | 0     |
| 600                 | 0.17046  | 0.90397 | -0.57302 | 0.2269  | -0.01743 | 0.0688  | 0     | 0     |
| 605                 | 0.18205  | 0.90496 | -0.58026 | 0.23009 | -0.01427 | 0.06815 | 0     | 0     |
| 610                 | 0.19103  | 0.90635 | -0.58673 | 0.23229 | -0.00999 | 0.06549 | 0     | 0     |
| 615                 | 0.19589  | 0.90814 | -0.59209 | 0.2337  | -0.00486 | 0.06093 | 0     | 0     |
| 620                 | 0.19545  | 0.91035 | -0.59603 | 0.2345  | 0.00083  | 0.05457 | 0     | 0     |
| 625                 | 0.18873  | 0.91297 | -0.59864 | 0.23485 | 0.00685  | 0.04682 | 0     | 0     |
| 630                 | 0.17514  | 0.91598 | -0.60046 | 0.2349  | 0.01298  | 0.03844 | 0     | 0     |
| 635                 | 0.15461  | 0.91935 | -0.60188 | 0.23486 | 0.0191   | 0.03017 | 0     | 0     |
| 640                 | 0.12791  | 0.92305 | -0.60283 | 0.23506 | 0.0253   | 0.02263 | 0     | 0     |
| 645                 | 0.09694  | 0.92707 | -0.60322 | 0.23576 | 0.03151  | 0.01633 | 0     | 0     |
| 650                 | 0.06435  | 0.9314  | -0.60304 | 0.23717 | 0.03758  | 0.01172 | 0     | 0     |
| 655                 | 0.03278  | 0.93603 | -0.60224 | 0.23951 | 0.04331  | 0.00924 | 0     | 0     |
| 660                 | 0.00403  | 0.94096 | -0.60081 | 0.24298 | 0.04854  | 0.00932 | 0     | 0     |
| 665                 | -0.02138 | 0.9462  | -0.59882 | 0.24774 | 0.05304  | 0.01201 | 0     | 0     |
| 670                 | -0.04399 | 0.95174 | -0.59638 | 0.25384 | 0.05655  | 0.01685 | 0     | 0     |
| 675                 | -0.06489 | 0.95757 | -0.59359 | 0.26128 | 0.05879  | 0.02333 | 0     | 0     |

Table 12: Normalized Legendre coefficients in  $K^-p \rightarrow \bar{K}^0 n$  (2/5)

| Momentum<br>(MeV/c) | A1/A0    | A2/A0   | A3/A0    | A4/A0   | A5/A0    | A6/A0    | A7/A0   | A8/A0 |
|---------------------|----------|---------|----------|---------|----------|----------|---------|-------|
| 680                 | -0.08497 | 0.96367 | -0.59053 | 0.27011 | 0.05955  | 0.03096  | -1e-05  | 0     |
| 685                 | -0.10471 | 0.97    | -0.58712 | 0.2802  | 0.0589   | 0.03927  | -1e-05  | 0     |
| 690                 | -0.12371 | 0.97649 | -0.58315 | 0.29136 | 0.05721  | 0.0478   | -1e-05  | 0     |
| 695                 | -0.14097 | 0.98305 | -0.57828 | 0.3031  | 0.05487  | 0.05603  | -1e-05  | 0     |
| 700                 | -0.15469 | 0.98957 | -0.57209 | 0.31472 | 0.05231  | 0.06337  | -1e-05  | 0     |
| 705                 | -0.16271 | 0.99591 | -0.56443 | 0.3256  | 0.04979  | 0.06932  | -1e-05  | 0     |
| 710                 | -0.16255 | 1.00194 | -0.55574 | 0.33535 | 0.04732  | 0.07359  | -2e-05  | 0     |
| 715                 | -0.15199 | 1.00752 | -0.54657 | 0.34363 | 0.04488  | 0.07591  | -2e-05  | 0     |
| 720                 | -0.12951 | 1.01251 | -0.53743 | 0.3499  | 0.04245  | 0.07587  | -2e-05  | 0     |
| 725                 | -0.09529 | 1.0168  | -0.52879 | 0.35376 | 0.03995  | 0.07327  | -2e-05  | 0     |
| 730                 | -0.05159 | 1.0203  | -0.5212  | 0.35562 | 0.03722  | 0.06853  | -2e-05  | 0     |
| 735                 | -0.00245 | 1.02293 | -0.51519 | 0.35595 | 0.0341   | 0.06213  | -2e-05  | 0     |
| 740                 | 0.04772  | 1.02468 | -0.51129 | 0.35522 | 0.03044  | 0.05455  | -2e-05  | 0     |
| 745                 | 0.09584  | 1.02553 | -0.51005 | 0.35387 | 0.02597  | 0.04627  | -2e-05  | 0     |
| 750                 | 0.14086  | 1.02552 | -0.51202 | 0.35229 | 0.02027  | 0.03776  | -1e-05  | 0     |
| 755                 | 0.18338  | 1.02466 | -0.51778 | 0.35084 | 0.01302  | 0.02948  | -1e-05  | 0     |
| 760                 | 0.22444  | 1.023   | -0.52787 | 0.34965 | 0.00409  | 0.02179  | 0       | 0     |
| 765                 | 0.2645   | 1.0206  | -0.54268 | 0.34874 | -0.00656 | 0.01494  | 1e-05   | 0     |
| 770                 | 0.30276  | 1.01748 | -0.56211 | 0.34808 | -0.01882 | 0.00896  | 2e-05   | 0     |
| 775                 | 0.33729  | 1.01369 | -0.58582 | 0.34762 | -0.03243 | 0.00376  | 4e-05   | 0     |
| 780                 | 0.36532  | 1.00926 | -0.61343 | 0.34741 | -0.04713 | -8e-04   | 6e-05   | 0     |
| 785                 | 0.38445  | 1.00421 | -0.64453 | 0.34758 | -0.06254 | -0.00496 | 8e-05   | 0     |
| 790                 | 0.39323  | 0.99857 | -0.67869 | 0.34828 | -0.07831 | -0.00897 | 0.00011 | 0     |
| 795                 | 0.39129  | 0.99243 | -0.71549 | 0.34967 | -0.09409 | -0.01306 | 0.00014 | 0     |
| 800                 | 0.37889  | 0.98587 | -0.75456 | 0.35269 | -0.10967 | -0.01765 | 0.00017 | 0     |
| 805                 | 0.35624  | 0.97903 | -0.79561 | 0.35848 | -0.12507 | -0.023   | 0.00021 | 0     |
| 810                 | 0.32292  | 0.97211 | -0.83834 | 0.36717 | -0.14022 | -0.02894 | 0.00025 | 0     |
| 815                 | 0.27791  | 0.96533 | -0.88246 | 0.37885 | -0.15509 | -0.03525 | 0.00029 | 0     |
| 820                 | 0.22029  | 0.95894 | -0.92768 | 0.39359 | -0.16961 | -0.04173 | 0.00034 | 0     |
| 825                 | 0.15048  | 0.9532  | -0.9737  | 0.41145 | -0.18373 | -0.04817 | 0.00039 | 0     |
| 830                 | 0.07108  | 0.94826 | -1.02023 | 0.43252 | -0.1974  | -0.05435 | 0.00044 | 0     |
| 835                 | -0.0136  | 0.94426 | -1.06697 | 0.45687 | -0.21057 | -0.06007 | 0.00049 | 0     |
| 840                 | -0.09855 | 0.94118 | -1.11361 | 0.48455 | -0.22318 | -0.06513 | 0.00054 | 0     |
| 845                 | -0.17951 | 0.9389  | -1.15976 | 0.51525 | -0.23515 | -0.06938 | 0.00059 | 0     |
| 850                 | -0.25366 | 0.93727 | -1.20484 | 0.54811 | -0.24638 | -0.07279 | 0.00064 | 0     |
| 855                 | -0.31965 | 0.93606 | -1.24827 | 0.58227 | -0.25672 | -0.07535 | 0.00069 | 0     |
| 860                 | -0.37707 | 0.93506 | -1.28948 | 0.61685 | -0.26608 | -0.07701 | 0.00072 | 0     |
| 865                 | -0.42612 | 0.93404 | -1.3279  | 0.651   | -0.27433 | -0.07778 | 0.00075 | 0     |
| 870                 | -0.46711 | 0.93281 | -1.36298 | 0.68418 | -0.28136 | -0.0779  | 0.00077 | 0     |
| 875                 | -0.50042 | 0.93129 | -1.39424 | 0.7161  | -0.28708 | -0.07783 | 0.00078 | 0     |
| 880                 | -0.52649 | 0.92936 | -1.42118 | 0.74648 | -0.29139 | -0.07803 | 0.00076 | 0     |
| 885                 | -0.54572 | 0.92699 | -1.44339 | 0.77492 | -0.29417 | -0.07883 | 0.00072 | 0     |
| 890                 | -0.55824 | 0.92417 | -1.46054 | 0.801   | -0.29529 | -0.08047 | 0.00065 | 0     |
| 895                 | -0.56399 | 0.92098 | -1.47259 | 0.82492 | -0.29497 | -0.08289 | 0.00054 | 0     |
| 900                 | -0.56271 | 0.91754 | -1.47975 | 0.84731 | -0.29367 | -0.08579 | 0.00039 | 0     |

Table 13: Normalized Legendre coefficients in  $K^- p \rightarrow \bar{K}^0 n$  (3/5)

| Momentum<br>(MeV/c) | A1/A0    | A2/A0   | A3/A0    | A4/A0   | A5/A0    | A6/A0    | A7/A0    | A8/A0    |
|---------------------|----------|---------|----------|---------|----------|----------|----------|----------|
| 905                 | -0.55466 | 0.91396 | -1.48218 | 0.86857 | -0.29166 | -0.08892 | 0.00018  | 0        |
| 910                 | -0.54086 | 0.91044 | -1.48007 | 0.88907 | -0.28921 | -0.09206 | -8e-05   | 0        |
| 915                 | -0.52332 | 0.90717 | -1.47358 | 0.90921 | -0.28662 | -0.09496 | -0.00042 | 0        |
| 920                 | -0.5045  | 0.90438 | -1.46288 | 0.92935 | -0.28415 | -0.09741 | -0.00084 | 0        |
| 925                 | -0.48654 | 0.9023  | -1.4482  | 0.94975 | -0.28214 | -0.09924 | -0.00135 | 0        |
| 930                 | -0.47053 | 0.90114 | -1.42984 | 0.97058 | -0.281   | -0.10034 | -0.00195 | 0        |
| 935                 | -0.45659 | 0.90112 | -1.40806 | 0.99201 | -0.2811  | -0.10059 | -0.00266 | 0        |
| 940                 | -0.44423 | 0.90246 | -1.38314 | 1.01421 | -0.28285 | -0.09988 | -0.00348 | 0        |
| 945                 | -0.43287 | 0.90525 | -1.35536 | 1.0371  | -0.28653 | -0.09816 | -0.00441 | 0        |
| 950                 | -0.42193 | 0.90965 | -1.32498 | 1.06041 | -0.29239 | -0.09538 | -0.00544 | 0        |
| 955                 | -0.41093 | 0.91577 | -1.29226 | 1.08389 | -0.30066 | -0.09153 | -0.00659 | 0        |
| 960                 | -0.39924 | 0.92369 | -1.25746 | 1.10725 | -0.31158 | -0.08656 | -0.00783 | 0        |
| 965                 | -0.38604 | 0.93346 | -1.22095 | 1.13008 | -0.32524 | -0.08039 | -0.00918 | 0        |
| 970                 | -0.37027 | 0.94514 | -1.18303 | 1.15197 | -0.34144 | -0.07311 | -0.01058 | 0        |
| 975                 | -0.35077 | 0.95876 | -1.14385 | 1.17271 | -0.35991 | -0.06496 | -0.01199 | 0        |
| 980                 | -0.32717 | 0.97435 | -1.10358 | 1.19206 | -0.38038 | -0.05616 | -0.01336 | 0        |
| 985                 | -0.3004  | 0.99188 | -1.0624  | 1.20979 | -0.40261 | -0.04696 | -0.01464 | 0        |
| 990                 | -0.27312 | 1.01135 | -1.02046 | 1.2257  | -0.42632 | -0.03758 | -0.01578 | 0        |
| 995                 | -0.24834 | 1.03272 | -0.97795 | 1.23954 | -0.45126 | -0.02826 | -0.01674 | 0        |
| 1000                | -0.22769 | 1.0559  | -0.93501 | 1.2511  | -0.47716 | -0.01922 | -0.01745 | 0        |
| 1005                | -0.21032 | 1.0808  | -0.89184 | 1.26017 | -0.50377 | -0.01069 | -0.01787 | 0        |
| 1010                | -0.19369 | 1.10728 | -0.84866 | 1.26669 | -0.53095 | -0.00261 | -0.0179  | 0        |
| 1015                | -0.17436 | 1.13513 | -0.80576 | 1.27066 | -0.55859 | 0.00512  | -0.01742 | 0        |
| 1020                | -0.1494  | 1.16411 | -0.7634  | 1.27208 | -0.58657 | 0.01264  | -0.01633 | 0        |
| 1025                | -0.11749 | 1.19391 | -0.72184 | 1.27097 | -0.61479 | 0.02007  | -0.01451 | 0        |
| 1030                | -0.081   | 1.22417 | -0.68137 | 1.26732 | -0.64314 | 0.02755  | -0.01185 | 0        |
| 1035                | -0.04533 | 1.25445 | -0.64225 | 1.26114 | -0.6715  | 0.0352   | -0.00824 | 0        |
| 1040                | -0.01646 | 1.28424 | -0.60476 | 1.25244 | -0.69977 | 0.04316  | -0.00356 | 0        |
| 1045                | 0.00361  | 1.31304 | -0.56915 | 1.24121 | -0.72785 | 0.05154  | 0.00231  | 0        |
| 1050                | 0.01552  | 1.34024 | -0.53567 | 1.22751 | -0.75561 | 0.06047  | 0.0094   | 0        |
| 1055                | 0.02103  | 1.36529 | -0.50435 | 1.21159 | -0.78295 | 0.07001  | 0.01752  | 0        |
| 1060                | 0.02215  | 1.38771 | -0.47519 | 1.19376 | -0.80975 | 0.08022  | 0.02639  | 0        |
| 1065                | 0.02047  | 1.40712 | -0.4482  | 1.1743  | -0.83589 | 0.09116  | 0.03575  | 0        |
| 1070                | 0.01735  | 1.4233  | -0.42337 | 1.15353 | -0.86126 | 0.10289  | 0.04532  | 0        |
| 1075                | 0.0137   | 1.43585 | -0.40071 | 1.13173 | -0.88574 | 0.11546  | 0.05485  | 0        |
| 1080                | 0.00983  | 1.44489 | -0.38022 | 1.10922 | -0.90921 | 0.12892  | 0.06405  | 0        |
| 1085                | 0.00516  | 1.45066 | -0.3619  | 1.08628 | -0.93157 | 0.14335  | 0.07265  | 0        |
| 1090                | -0.00091 | 1.45292 | -0.34574 | 1.0632  | -0.95272 | 0.15877  | 0.08044  | 0        |
| 1095                | -0.00921 | 1.4522  | -0.33171 | 1.04013 | -0.97273 | 0.17517  | 0.08734  | 0        |
| 1100                | -0.01996 | 1.44884 | -0.31977 | 1.01722 | -0.99171 | 0.19252  | 0.09332  | -2e-05   |
| 1105                | -0.03239 | 1.44326 | -0.30987 | 0.99459 | -1.00975 | 0.2108   | 0.09835  | -4e-05   |
| 1110                | -0.0447  | 1.43582 | -0.30197 | 0.97238 | -1.02695 | 0.22997  | 0.1024   | -6e-05   |
| 1115                | -0.05508 | 1.42673 | -0.29604 | 0.95074 | -1.0434  | 0.25     | 0.10545  | -9e-05   |
| 1120                | -0.06264 | 1.41667 | -0.29202 | 0.92979 | -1.05922 | 0.27085  | 0.10746  | -0.00015 |
| 1125                | -0.06741 | 1.40585 | -0.28988 | 0.90967 | -1.0745  | 0.29251  | 0.10841  | -0.00023 |
| 1130                | -0.06996 | 1.39476 | -0.28958 | 0.89052 | -1.08934 | 0.31494  | 0.10826  | -0.00036 |

Table 14: Normalized Legendre coefficients in  $K^- p \rightarrow \bar{K}^0 n$  (4/5)

| Momentum<br>(MeV/c) | A1/A0    | A2/A0   | A3/A0    | A4/A0   | A5/A0    | A6/A0   | A7/A0    | A8/A0    |
|---------------------|----------|---------|----------|---------|----------|---------|----------|----------|
| 1135                | -0.07105 | 1.38376 | -0.29107 | 0.87247 | -1.10383 | 0.3381  | 0.107    | -0.00054 |
| 1140                | -0.0711  | 1.3732  | -0.29431 | 0.85567 | -1.11808 | 0.36197 | 0.10458  | -0.00087 |
| 1145                | -0.07085 | 1.36335 | -0.29927 | 0.84024 | -1.13219 | 0.38652 | 0.10099  | -0.00128 |
| 1150                | -0.07116 | 1.35452 | -0.30589 | 0.82632 | -1.14626 | 0.41172 | 0.09619  | -0.00185 |
| 1155                | -0.07304 | 1.34687 | -0.31414 | 0.81405 | -1.16038 | 0.43753 | 0.09015  | -0.00263 |
| 1160                | -0.07771 | 1.34061 | -0.32397 | 0.80356 | -1.17466 | 0.46393 | 0.08284  | -0.00367 |
| 1165                | -0.08664 | 1.3359  | -0.33535 | 0.79499 | -1.18919 | 0.49089 | 0.07424  | -0.00506 |
| 1170                | -0.10173 | 1.33284 | -0.34823 | 0.78841 | -1.20404 | 0.51834 | 0.06434  | -0.00686 |
| 1175                | -0.12509 | 1.33145 | -0.36258 | 0.78356 | -1.21914 | 0.54614 | 0.05318  | -0.00925 |
| 1180                | -0.15682 | 1.33177 | -0.37838 | 0.78014 | -1.23438 | 0.57409 | 0.04086  | -0.0122  |
| 1185                | -0.19464 | 1.33374 | -0.39559 | 0.77782 | -1.24965 | 0.60201 | 0.02744  | -0.01586 |
| 1190                | -0.23352 | 1.33727 | -0.41419 | 0.7763  | -1.26484 | 0.62972 | 0.01301  | -0.02035 |
| 1195                | -0.26876 | 1.34221 | -0.43415 | 0.77525 | -1.27985 | 0.65702 | -0.00237 | -0.02577 |
| 1200                | -0.299   | 1.34841 | -0.45544 | 0.77437 | -1.29457 | 0.68375 | -0.01862 | -0.0322  |
| 1205                | -0.32631 | 1.35562 | -0.47804 | 0.77332 | -1.30888 | 0.7097  | -0.03565 | -0.03976 |
| 1210                | -0.35505 | 1.36358 | -0.50188 | 0.77186 | -1.32269 | 0.73474 | -0.05339 | -0.04851 |
| 1215                | -0.38961 | 1.372   | -0.52686 | 0.7699  | -1.33587 | 0.75888 | -0.07178 | -0.0585  |
| 1220                | -0.43176 | 1.38055 | -0.55282 | 0.76744 | -1.3483  | 0.78219 | -0.09072 | -0.06977 |
| 1225                | -0.47936 | 1.38889 | -0.57962 | 0.76446 | -1.35986 | 0.80471 | -0.11016 | -0.08229 |
| 1230                | -0.52635 | 1.39666 | -0.60711 | 0.76094 | -1.37043 | 0.82652 | -0.13    | -0.09604 |
| 1235                | -0.56649 | 1.40351 | -0.63516 | 0.75687 | -1.37988 | 0.84766 | -0.15019 | -0.11094 |
| 1240                | -0.59709 | 1.40914 | -0.66361 | 0.75222 | -1.3881  | 0.86819 | -0.17064 | -0.12681 |
| 1245                | -0.61879 | 1.41323 | -0.69232 | 0.74699 | -1.39497 | 0.88817 | -0.19128 | -0.14349 |
| 1250                | -0.63452 | 1.41555 | -0.72116 | 0.74115 | -1.40036 | 0.90767 | -0.21203 | -0.16074 |
| 1255                | -0.6472  | 1.4159  | -0.74996 | 0.73469 | -1.40415 | 0.92673 | -0.23283 | -0.17827 |
| 1260                | -0.65841 | 1.4142  | -0.77859 | 0.7276  | -1.40622 | 0.94542 | -0.25358 | -0.19575 |
| 1265                | -0.66819 | 1.41043 | -0.80691 | 0.71985 | -1.40646 | 0.96379 | -0.27423 | -0.21283 |
| 1270                | -0.67506 | 1.40465 | -0.83476 | 0.71143 | -1.40474 | 0.9819  | -0.29469 | -0.22916 |
| 1275                | -0.67695 | 1.39703 | -0.86202 | 0.70233 | -1.40093 | 0.99981 | -0.3149  | -0.24439 |
| 1280                | -0.67215 | 1.38781 | -0.88852 | 0.69252 | -1.39492 | 1.01758 | -0.33477 | -0.25814 |
| 1285                | -0.65883 | 1.37728 | -0.91412 | 0.68199 | -1.38659 | 1.03527 | -0.35423 | -0.27016 |
| 1290                | -0.63639 | 1.36579 | -0.93873 | 0.67076 | -1.37587 | 1.05293 | -0.37323 | -0.28021 |
| 1295                | -0.60463 | 1.35371 | -0.96237 | 0.65893 | -1.3629  | 1.07059 | -0.3918  | -0.28812 |
| 1300                | -0.56527 | 1.34141 | -0.98514 | 0.64665 | -1.34787 | 1.08829 | -0.41    | -0.29382 |
| 1305                | -0.52229 | 1.32923 | -1.0071  | 0.63407 | -1.33099 | 1.10606 | -0.4279  | -0.29727 |
| 1310                | -0.4806  | 1.31751 | -1.02834 | 0.62132 | -1.31244 | 1.12394 | -0.44553 | -0.29853 |
| 1315                | -0.44384 | 1.3065  | -1.04893 | 0.60855 | -1.29241 | 1.14195 | -0.46298 | -0.29776 |
| 1320                | -0.41298 | 1.29641 | -1.06896 | 0.5959  | -1.27111 | 1.16013 | -0.48028 | -0.29505 |
| 1325                | -0.38708 | 1.28739 | -1.0885  | 0.58352 | -1.24873 | 1.17852 | -0.4975  | -0.29066 |
| 1330                | -0.36429 | 1.27952 | -1.10764 | 0.57154 | -1.22546 | 1.19714 | -0.5147  | -0.28485 |
| 1335                | -0.34347 | 1.27284 | -1.12645 | 0.56012 | -1.2015  | 1.21602 | -0.53193 | -0.27787 |
| 1340                | -0.32464 | 1.26732 | -1.14501 | 0.54939 | -1.17704 | 1.23521 | -0.54926 | -0.26998 |
| 1345                | -0.30854 | 1.2629  | -1.1634  | 0.5395  | -1.15228 | 1.25472 | -0.56673 | -0.26145 |
| 1350                | -0.29584 | 1.25949 | -1.18169 | 0.53059 | -1.1274  | 1.27461 | -0.58441 | -0.2525  |
| 1355                | -0.28655 | 1.25697 | -1.19998 | 0.52281 | -1.10262 | 1.29488 | -0.60235 | -0.2434  |

Table 15: Normalized Legendre coefficients in  $K^- p \rightarrow \bar{K}^0 n$  (5/5)

| Momentum<br>(MeV/c) | A1/A0   | A2/A0   | A3/A0   | A4/A0    | A5/A0    | A6/A0    | A7/A0 |
|---------------------|---------|---------|---------|----------|----------|----------|-------|
| 435                 | 1.29381 | 0.87668 | 0.24531 | 0.00844  | -0.0067  | 4e-05    | 0     |
| 440                 | 1.28561 | 0.87491 | 0.24024 | 0.00529  | -0.00609 | 3e-05    | 0     |
| 445                 | 1.27743 | 0.87315 | 0.23522 | 0.00212  | -0.00547 | 3e-05    | 0     |
| 450                 | 1.26928 | 0.87139 | 0.2303  | -0.00105 | -0.00485 | 2e-05    | 0     |
| 455                 | 1.2612  | 0.86965 | 0.22553 | -0.00424 | -0.0042  | 1e-05    | 0     |
| 460                 | 1.25317 | 0.86792 | 0.22099 | -0.00745 | -0.00354 | 0        | 0     |
| 465                 | 1.24512 | 0.86623 | 0.21678 | -0.01069 | -0.00284 | 0        | 0     |
| 470                 | 1.23692 | 0.86461 | 0.21304 | -0.01397 | -0.00211 | -1e-05   | 0     |
| 475                 | 1.22848 | 0.86311 | 0.20991 | -0.01729 | -0.00132 | -2e-05   | 0     |
| 480                 | 1.21967 | 0.86172 | 0.20749 | -0.02066 | -0.00048 | -3e-05   | 0     |
| 485                 | 1.21035 | 0.86044 | 0.20577 | -0.02407 | 0.00044  | -3e-05   | 0     |
| 490                 | 1.2004  | 0.85923 | 0.20473 | -0.02748 | 0.00143  | -4e-05   | 0     |
| 495                 | 1.18967 | 0.85804 | 0.20434 | -0.03087 | 0.00251  | -5e-05   | 0     |
| 500                 | 1.17802 | 0.85684 | 0.20455 | -0.03423 | 0.00369  | -6e-05   | 0     |
| 505                 | 1.16533 | 0.8556  | 0.20535 | -0.03753 | 0.00497  | -7e-05   | 0     |
| 510                 | 1.15145 | 0.85427 | 0.20669 | -0.04075 | 0.00637  | -8e-05   | 0     |
| 515                 | 1.13624 | 0.85282 | 0.20855 | -0.04386 | 0.0079   | -9e-05   | 0     |
| 520                 | 1.11972 | 0.85121 | 0.21086 | -0.0468  | 0.00955  | -1e-04   | 0     |
| 525                 | 1.10208 | 0.84953 | 0.21379 | -0.04947 | 0.01133  | -0.00011 | 0     |
| 530                 | 1.0835  | 0.84789 | 0.21759 | -0.05178 | 0.01323  | -0.00012 | 0     |
| 535                 | 1.06417 | 0.84639 | 0.2225  | -0.05361 | 0.01525  | -0.00013 | 0     |
| 540                 | 1.04423 | 0.8451  | 0.22862 | -0.05493 | 0.01738  | -0.00014 | 0     |
| 545                 | 1.02374 | 0.844   | 0.23576 | -0.05583 | 0.0196   | -0.00015 | 0     |
| 550                 | 1.00274 | 0.84308 | 0.2437  | -0.05642 | 0.02189  | -0.00016 | 0     |
| 555                 | 0.98125 | 0.8423  | 0.25219 | -0.05681 | 0.02423  | -0.00017 | 0     |
| 560                 | 0.95932 | 0.84165 | 0.26101 | -0.0571  | 0.02659  | -0.00017 | 0     |
| 565                 | 0.93696 | 0.84108 | 0.26988 | -0.05743 | 0.02895  | -0.00018 | 0     |
| 570                 | 0.91408 | 0.84053 | 0.27837 | -0.05801 | 0.03126  | -0.00018 | 0     |
| 575                 | 0.89056 | 0.83994 | 0.28602 | -0.05907 | 0.03345  | -0.00018 | 0     |
| 580                 | 0.86629 | 0.8393  | 0.29249 | -0.06069 | 0.03543  | -0.00017 | 0     |
| 585                 | 0.84122 | 0.83869 | 0.29765 | -0.06277 | 0.0371   | -0.00016 | 0     |
| 590                 | 0.81531 | 0.83818 | 0.30154 | -0.06516 | 0.03842  | -0.00015 | 0     |
| 595                 | 0.78853 | 0.83781 | 0.30425 | -0.06771 | 0.03943  | -0.00012 | 0     |
| 600                 | 0.76086 | 0.83762 | 0.30587 | -0.07025 | 0.04015  | -9e-05   | 1e-05 |
| 605                 | 0.73242 | 0.83777 | 0.30661 | -0.07259 | 0.0406   | -6e-05   | 1e-05 |
| 610                 | 0.7034  | 0.8385  | 0.30673 | -0.07453 | 0.04081  | -1e-05   | 1e-05 |
| 615                 | 0.67402 | 0.84003 | 0.3065  | -0.07588 | 0.0408   | 5e-05    | 1e-05 |
| 620                 | 0.6445  | 0.8426  | 0.30618 | -0.07642 | 0.0406   | 0.00012  | 1e-05 |
| 625                 | 0.61503 | 0.84637 | 0.30581 | -0.07599 | 0.04021  | 2e-04    | 2e-05 |
| 630                 | 0.5858  | 0.85147 | 0.30525 | -0.07444 | 0.03962  | 3e-04    | 2e-05 |
| 635                 | 0.557   | 0.85801 | 0.30443 | -0.07169 | 0.03881  | 0.00041  | 2e-05 |
| 640                 | 0.5289  | 0.86611 | 0.30346 | -0.06786 | 0.03772  | 0.00053  | 3e-05 |
| 645                 | 0.50176 | 0.87586 | 0.30245 | -0.06312 | 0.03626  | 0.00068  | 3e-05 |
| 650                 | 0.47582 | 0.8874  | 0.30153 | -0.05762 | 0.03438  | 0.00084  | 3e-05 |
| 655                 | 0.45135 | 0.90083 | 0.30082 | -0.05148 | 0.03201  | 0.00101  | 4e-05 |

Table 16: Normalized Legendre coefficients in  $\overline{K}N \rightarrow \Lambda\pi$  (1/7)



| Momentum<br>(MeV/c) | A1/A0    | A2/A0   | A3/A0   | A4/A0    | A5/A0   | A6/A0    | A7/A0    |
|---------------------|----------|---------|---------|----------|---------|----------|----------|
| 660                 | 0.42865  | 0.91629 | 0.30054 | -0.0447  | 0.0292  | 0.0012   | 4e-05    |
| 665                 | 0.40794  | 0.93393 | 0.30079 | -0.03707 | 0.02606 | 0.00141  | 4e-05    |
| 670                 | 0.38927  | 0.95387 | 0.30149 | -0.0283  | 0.02276 | 0.00163  | 5e-05    |
| 675                 | 0.37268  | 0.97623 | 0.30251 | -0.01806 | 0.01946 | 0.00187  | 5e-05    |
| 680                 | 0.35818  | 1.0011  | 0.30373 | -0.00607 | 0.01635 | 0.0021   | 5e-05    |
| 685                 | 0.34574  | 1.02858 | 0.30527 | 0.00796  | 0.0136  | 0.00234  | 5e-05    |
| 690                 | 0.33527  | 1.05871 | 0.30741 | 0.02426  | 0.01138 | 0.00257  | 5e-05    |
| 695                 | 0.32658  | 1.09138 | 0.31026 | 0.04292  | 0.00982 | 0.0028   | 5e-05    |
| 700                 | 0.31939  | 1.12634 | 0.31382 | 0.06382  | 0.00895 | 0.003    | 5e-05    |
| 705                 | 0.31344  | 1.16334 | 0.31815 | 0.08676  | 0.00879 | 0.00317  | 4e-05    |
| 710                 | 0.3086   | 1.20215 | 0.32345 | 0.11138  | 0.00935 | 0.00328  | 4e-05    |
| 715                 | 0.30471  | 1.24255 | 0.32994 | 0.13731  | 0.01061 | 0.00334  | 3e-05    |
| 720                 | 0.30161  | 1.28419 | 0.33773 | 0.16421  | 0.01265 | 0.00332  | 2e-05    |
| 725                 | 0.29909  | 1.32659 | 0.34682 | 0.19187  | 0.01564 | 0.0032   | 0        |
| 730                 | 0.29695  | 1.36945 | 0.35725 | 0.22005  | 0.01956 | 0.00296  | -2e-05   |
| 735                 | 0.29502  | 1.41255 | 0.36915 | 0.24854  | 0.0243  | 0.00258  | -4e-05   |
| 740                 | 0.29311  | 1.45571 | 0.38262 | 0.27709  | 0.02974 | 0.00202  | -7e-05   |
| 745                 | 0.29109  | 1.49871 | 0.39781 | 0.3055   | 0.03575 | 0.00127  | -0.00011 |
| 750                 | 0.28898  | 1.54138 | 0.41503 | 0.33366  | 0.0422  | 0.00029  | -0.00015 |
| 755                 | 0.28683  | 1.58345 | 0.43457 | 0.36147  | 0.04894 | -0.00094 | -0.00019 |
| 760                 | 0.28451  | 1.6243  | 0.45625 | 0.38871  | 0.05591 | -0.00244 | -0.00025 |
| 765                 | 0.28175  | 1.66337 | 0.47979 | 0.41518  | 0.06308 | -0.00425 | -0.00031 |
| 770                 | 0.27835  | 1.70025 | 0.50482 | 0.44067  | 0.07042 | -0.00639 | -0.00037 |
| 775                 | 0.27417  | 1.73456 | 0.53095 | 0.46502  | 0.07785 | -0.00889 | -0.00044 |
| 780                 | 0.26902  | 1.76599 | 0.55773 | 0.48808  | 0.08531 | -0.01176 | -0.00052 |
| 785                 | 0.26276  | 1.79435 | 0.58464 | 0.50969  | 0.09264 | -0.01503 | -6e-04   |
| 790                 | 0.2552   | 1.81947 | 0.61114 | 0.52972  | 0.09971 | -0.0187  | -0.00068 |
| 795                 | 0.24617  | 1.84117 | 0.6367  | 0.54802  | 0.10638 | -0.02279 | -0.00077 |
| 800                 | 0.23554  | 1.85933 | 0.66076 | 0.56451  | 0.11244 | -0.0273  | -0.00086 |
| 805                 | 0.22322  | 1.87397 | 0.68275 | 0.57917  | 0.11765 | -0.03222 | -0.00095 |
| 810                 | 0.20914  | 1.8851  | 0.70209 | 0.592    | 0.12173 | -0.03752 | -0.00104 |
| 815                 | 0.1932   | 1.89272 | 0.7182  | 0.60299  | 0.12443 | -0.04319 | -0.00113 |
| 820                 | 0.17533  | 1.89686 | 0.73052 | 0.61214  | 0.1255  | -0.04922 | -0.00121 |
| 825                 | 0.15565  | 1.89756 | 0.73887 | 0.61947  | 0.12491 | -0.05557 | -0.00128 |
| 830                 | 0.13439  | 1.89493 | 0.74336 | 0.62504  | 0.12283 | -0.06219 | -0.00134 |
| 835                 | 0.11178  | 1.88905 | 0.74408 | 0.62889  | 0.11942 | -0.06905 | -0.00139 |
| 840                 | 0.08807  | 1.88001 | 0.74115 | 0.63106  | 0.11484 | -0.07609 | -0.00143 |
| 845                 | 0.0635   | 1.86791 | 0.73467 | 0.63161  | 0.10925 | -0.08327 | -0.00144 |
| 850                 | 0.03831  | 1.85283 | 0.72475 | 0.63058  | 0.10282 | -0.09055 | -0.00144 |
| 855                 | 0.01278  | 1.83488 | 0.7116  | 0.62802  | 0.09574 | -0.09784 | -0.00142 |
| 860                 | -0.01274 | 1.81419 | 0.69565 | 0.624    | 0.0883  | -0.105   | -0.00136 |
| 865                 | -0.03789 | 1.79087 | 0.67736 | 0.61858  | 0.08079 | -0.11186 | -0.00127 |
| 870                 | -0.06232 | 1.76507 | 0.65719 | 0.61182  | 0.07351 | -0.11824 | -0.00115 |
| 875                 | -0.08566 | 1.73691 | 0.63561 | 0.60379  | 0.06676 | -0.12399 | -0.00099 |

Table 17: Normalized Legendre coefficients in  $\bar{K}N \rightarrow \Lambda\pi$  (2/7)

| Momentum<br>(MeV/c) | A1/A0    | A2/A0   | A3/A0    | A4/A0    | A5/A0   | A6/A0    | A7/A0    |
|---------------------|----------|---------|----------|----------|---------|----------|----------|
| 880                 | -0.10755 | 1.70652 | 0.61308  | 0.59454  | 0.06082 | -0.12894 | -0.00077 |
| 885                 | -0.12763 | 1.67402 | 0.59005  | 0.58414  | 0.05598 | -0.13293 | -0.00051 |
| 890                 | -0.1458  | 1.63947 | 0.56679  | 0.57245  | 0.05242 | -0.13584 | -0.00019 |
| 895                 | -0.16195 | 1.60305 | 0.54339  | 0.5594   | 0.05012 | -0.13773 | 0.00019  |
| 900                 | -0.17602 | 1.56493 | 0.51984  | 0.54502  | 0.04902 | -0.13871 | 0.00064  |
| 905                 | -0.18798 | 1.52525 | 0.4961   | 0.52929  | 0.049   | -0.13888 | 0.00117  |
| 910                 | -0.19778 | 1.48414 | 0.47216  | 0.51223  | 0.04998 | -0.13838 | 0.00177  |
| 915                 | -0.20538 | 1.44176 | 0.44798  | 0.49384  | 0.05185 | -0.13732 | 0.00247  |
| 920                 | -0.21074 | 1.39824 | 0.42355  | 0.47412  | 0.05451 | -0.13581 | 0.00325  |
| 925                 | -0.21388 | 1.35383 | 0.39886  | 0.45319  | 0.05787 | -0.13396 | 0.00414  |
| 930                 | -0.21484 | 1.30892 | 0.37401  | 0.4313   | 0.06178 | -0.13183 | 0.00512  |
| 935                 | -0.21369 | 1.2639  | 0.34905  | 0.40872  | 0.06613 | -0.1295  | 0.0062   |
| 940                 | -0.2105  | 1.21913 | 0.32406  | 0.38569  | 0.07078 | -0.12704 | 0.00739  |
| 945                 | -0.20536 | 1.17491 | 0.29905  | 0.36232  | 0.07556 | -0.12458 | 0.00869  |
| 950                 | -0.19836 | 1.13145 | 0.27401  | 0.33866  | 0.08027 | -0.12224 | 0.01009  |
| 955                 | -0.18958 | 1.08898 | 0.24895  | 0.31474  | 0.08473 | -0.12018 | 0.01158  |
| 960                 | -0.17912 | 1.04775 | 0.22386  | 0.2906   | 0.08874 | -0.11852 | 0.01318  |
| 965                 | -0.16707 | 1.00794 | 0.19872  | 0.26627  | 0.09217 | -0.11741 | 0.01487  |
| 970                 | -0.15345 | 0.96965 | 0.17358  | 0.24171  | 0.09504 | -0.11702 | 0.01662  |
| 975                 | -0.1383  | 0.93292 | 0.14845  | 0.21687  | 0.09744 | -0.1175  | 0.01841  |
| 980                 | -0.12165 | 0.89782 | 0.12337  | 0.19178  | 0.09944 | -0.11883 | 0.0202   |
| 985                 | -0.10352 | 0.86439 | 0.09835  | 0.16649  | 0.10108 | -0.12091 | 0.02197  |
| 990                 | -0.08393 | 0.83266 | 0.07345  | 0.14106  | 0.1024  | -0.12362 | 0.02367  |
| 995                 | -0.06289 | 0.80271 | 0.04868  | 0.11554  | 0.10346 | -0.12687 | 0.02527  |
| 1000                | -0.04044 | 0.77456 | 0.02407  | 0.09     | 0.10431 | -0.13055 | 0.02675  |
| 1005                | -0.0166  | 0.74824 | -3e-04   | 0.06448  | 0.10496 | -0.13453 | 0.02801  |
| 1010                | 0.00852  | 0.72368 | -0.02409 | 0.03902  | 0.1053  | -0.13858 | 0.02872  |
| 1015                | 0.03479  | 0.70081 | -0.0472  | 0.01366  | 0.10528 | -0.14262 | 0.02878  |
| 1020                | 0.06212  | 0.67958 | -0.06962 | -0.01158 | 0.10492 | -0.14664 | 0.02821  |
| 1025                | 0.0904   | 0.65992 | -0.09133 | -0.03664 | 0.10421 | -0.15064 | 0.02703  |
| 1030                | 0.11951  | 0.64179 | -0.11234 | -0.0615  | 0.10315 | -0.15461 | 0.02526  |
| 1035                | 0.14935  | 0.62513 | -0.13261 | -0.08611 | 0.10174 | -0.15854 | 0.02291  |
| 1040                | 0.1798   | 0.60989 | -0.15215 | -0.11044 | 0.09999 | -0.16241 | 0.02     |
| 1045                | 0.21078  | 0.59602 | -0.17094 | -0.13445 | 0.0979  | -0.16622 | 0.01656  |
| 1050                | 0.24215  | 0.58346 | -0.18897 | -0.15811 | 0.09547 | -0.16996 | 0.01259  |
| 1055                | 0.27383  | 0.57216 | -0.20623 | -0.18137 | 0.0927  | -0.17363 | 0.00812  |
| 1060                | 0.30569  | 0.56207 | -0.2227  | -0.20421 | 0.08959 | -0.1772  | 0.00316  |
| 1065                | 0.33764  | 0.55313 | -0.23838 | -0.22657 | 0.08615 | -0.18068 | -0.00227 |
| 1070                | 0.36956  | 0.54529 | -0.25326 | -0.24843 | 0.08237 | -0.18405 | -0.00815 |
| 1075                | 0.40134  | 0.53849 | -0.26732 | -0.26974 | 0.07826 | -0.1873  | -0.01447 |
| 1080                | 0.43288  | 0.53269 | -0.28055 | -0.29047 | 0.07382 | -0.19043 | -0.02119 |
| 1085                | 0.46407  | 0.52783 | -0.29295 | -0.31059 | 0.06905 | -0.19342 | -0.02832 |
| 1090                | 0.49481  | 0.52386 | -0.30452 | -0.33004 | 0.06396 | -0.19627 | -0.03582 |
| 1095                | 0.52503  | 0.52073 | -0.31538 | -0.34881 | 0.05856 | -0.1989  | -0.04359 |

Table 18: Normalized Legendre coefficients in  $\bar{K}N \rightarrow \Lambda\pi$  (3/7)

| Momentum<br>(MeV/c) | A1/A0   | A2/A0   | A3/A0    | A4/A0    | A5/A0    | A6/A0    | A7/A0    |
|---------------------|---------|---------|----------|----------|----------|----------|----------|
| 1100                | 0.55465 | 0.51841 | -0.3257  | -0.36683 | 0.05286  | -0.20125 | -0.05154 |
| 1105                | 0.58361 | 0.51686 | -0.3356  | -0.38409 | 0.0469   | -0.20327 | -0.05957 |
| 1110                | 0.61184 | 0.51604 | -0.34525 | -0.40052 | 0.04068  | -0.20488 | -0.06757 |
| 1115                | 0.63927 | 0.5159  | -0.35478 | -0.4161  | 0.03422  | -0.20602 | -0.07545 |
| 1120                | 0.66583 | 0.51641 | -0.36435 | -0.43079 | 0.02755  | -0.20662 | -0.08311 |
| 1125                | 0.69146 | 0.51753 | -0.37411 | -0.44454 | 0.02068  | -0.20662 | -0.09043 |
| 1130                | 0.71609 | 0.51922 | -0.38418 | -0.45732 | 0.01364  | -0.20594 | -0.09736 |
| 1135                | 0.73967 | 0.5214  | -0.3946  | -0.46913 | 0.00649  | -0.20451 | -0.10389 |
| 1140                | 0.76215 | 0.52403 | -0.40542 | -0.47994 | -0.00069 | -0.20222 | -0.11009 |
| 1145                | 0.78348 | 0.52703 | -0.41665 | -0.48977 | -0.00782 | -0.19898 | -0.11598 |
| 1150                | 0.80362 | 0.53033 | -0.42833 | -0.49859 | -0.01484 | -0.19469 | -0.1216  |
| 1155                | 0.82251 | 0.53388 | -0.44048 | -0.50642 | -0.02166 | -0.18927 | -0.12701 |
| 1160                | 0.8401  | 0.53761 | -0.45313 | -0.51323 | -0.02821 | -0.18261 | -0.13223 |
| 1165                | 0.85635 | 0.54144 | -0.46631 | -0.51903 | -0.03442 | -0.17462 | -0.13732 |
| 1170                | 0.87122 | 0.54533 | -0.48004 | -0.52382 | -0.04023 | -0.16525 | -0.14231 |
| 1175                | 0.88472 | 0.54924 | -0.49427 | -0.52765 | -0.0457  | -0.15454 | -0.1472  |
| 1180                | 0.89689 | 0.55314 | -0.50896 | -0.5306  | -0.0509  | -0.1426  | -0.15202 |
| 1185                | 0.90774 | 0.55701 | -0.52406 | -0.53273 | -0.05591 | -0.12951 | -0.15675 |
| 1190                | 0.91731 | 0.56082 | -0.53952 | -0.53411 | -0.06079 | -0.11537 | -0.16142 |
| 1195                | 0.92561 | 0.56455 | -0.55528 | -0.53481 | -0.06563 | -0.10027 | -0.16601 |
| 1200                | 0.93269 | 0.56816 | -0.57129 | -0.53488 | -0.07049 | -0.08429 | -0.17056 |
| 1205                | 0.93856 | 0.57163 | -0.58751 | -0.53441 | -0.07546 | -0.06754 | -0.17505 |
| 1210                | 0.94325 | 0.57494 | -0.60389 | -0.53345 | -0.0806  | -0.0501  | -0.17949 |
| 1215                | 0.94679 | 0.57806 | -0.62037 | -0.53208 | -0.086   | -0.03207 | -0.1839  |
| 1220                | 0.94921 | 0.58096 | -0.6369  | -0.53036 | -0.09172 | -0.01354 | -0.18827 |
| 1225                | 0.95052 | 0.58361 | -0.65343 | -0.52836 | -0.09784 | 0.00541  | -0.19262 |
| 1230                | 0.95077 | 0.58599 | -0.66992 | -0.52614 | -0.10444 | 0.02468  | -0.19694 |
| 1235                | 0.94997 | 0.58808 | -0.68631 | -0.52378 | -0.11159 | 0.04417  | -0.20126 |
| 1240                | 0.94816 | 0.58984 | -0.70255 | -0.52133 | -0.11936 | 0.06379  | -0.20557 |
| 1245                | 0.94535 | 0.59125 | -0.71859 | -0.51888 | -0.12783 | 0.08346  | -0.20987 |
| 1250                | 0.94157 | 0.59229 | -0.73437 | -0.51648 | -0.13706 | 0.10305  | -0.21416 |
| 1255                | 0.93683 | 0.59293 | -0.74976 | -0.51419 | -0.1471  | 0.12231  | -0.21828 |
| 1260                | 0.93113 | 0.59315 | -0.76463 | -0.51207 | -0.15797 | 0.14096  | -0.22206 |
| 1265                | 0.92447 | 0.59294 | -0.77883 | -0.51019 | -0.1697  | 0.15872  | -0.22534 |
| 1270                | 0.91689 | 0.59232 | -0.79218 | -0.50845 | -0.18223 | 0.17547  | -0.22804 |
| 1275                | 0.90848 | 0.5914  | -0.80445 | -0.5066  | -0.19545 | 0.19131  | -0.23018 |
| 1280                | 0.89933 | 0.59026 | -0.81539 | -0.50438 | -0.20919 | 0.20634  | -0.2318  |
| 1285                | 0.88952 | 0.58902 | -0.82477 | -0.50151 | -0.22331 | 0.22066  | -0.23293 |
| 1290                | 0.87914 | 0.58776 | -0.83234 | -0.49778 | -0.23768 | 0.23437  | -0.23361 |
| 1295                | 0.86827 | 0.58655 | -0.83797 | -0.49307 | -0.25217 | 0.24756  | -0.23388 |
| 1300                | 0.85696 | 0.58546 | -0.84148 | -0.48733 | -0.26668 | 0.26028  | -0.23375 |
| 1305                | 0.8453  | 0.58454 | -0.84274 | -0.4805  | -0.2811  | 0.27262  | -0.23327 |
| 1310                | 0.83334 | 0.58385 | -0.84159 | -0.47251 | -0.29532 | 0.28466  | -0.23245 |
| 1315                | 0.82116 | 0.58345 | -0.8379  | -0.46331 | -0.30922 | 0.29645  | -0.23134 |

Table 19: Normalized Legendre coefficients in  $\bar{K}N \rightarrow \Lambda\pi$  (4/7)

| Momentum<br>(MeV/c) | A1/A0   | A2/A0   | A3/A0    | A4/A0    | A5/A0    | A6/A0   | A7/A0    |
|---------------------|---------|---------|----------|----------|----------|---------|----------|
| 1320                | 0.80881 | 0.58341 | -0.8315  | -0.45284 | -0.32269 | 0.30807 | -0.22995 |
| 1325                | 0.79636 | 0.58376 | -0.82231 | -0.44106 | -0.33567 | 0.31957 | -0.22833 |
| 1330                | 0.78383 | 0.58452 | -0.81043 | -0.42806 | -0.34819 | 0.33087 | -0.22653 |
| 1335                | 0.77121 | 0.58565 | -0.79603 | -0.41395 | -0.36036 | 0.34185 | -0.22459 |
| 1340                | 0.75852 | 0.58715 | -0.77928 | -0.39886 | -0.37227 | 0.3524  | -0.22258 |
| 1345                | 0.74577 | 0.589   | -0.76033 | -0.38289 | -0.38399 | 0.36242 | -0.22055 |
| 1350                | 0.73295 | 0.59118 | -0.73935 | -0.36617 | -0.39563 | 0.37178 | -0.21857 |
| 1355                | 0.72008 | 0.59368 | -0.71651 | -0.3488  | -0.40726 | 0.38039 | -0.21667 |
| 1360                | 0.70715 | 0.59646 | -0.69194 | -0.3309  | -0.41893 | 0.38818 | -0.2149  |
| 1365                | 0.6941  | 0.59943 | -0.66566 | -0.31253 | -0.43043 | 0.39531 | -0.21314 |
| 1370                | 0.68084 | 0.60248 | -0.63764 | -0.29373 | -0.44151 | 0.40198 | -0.21126 |
| 1375                | 0.66737 | 0.60553 | -0.60795 | -0.27456 | -0.45201 | 0.40833 | -0.20918 |
| 1380                | 0.65371 | 0.60856 | -0.57672 | -0.25501 | -0.46189 | 0.41438 | -0.2069  |
| 1385                | 0.63991 | 0.61158 | -0.5441  | -0.2351  | -0.47112 | 0.42015 | -0.20442 |
| 1390                | 0.62603 | 0.61456 | -0.51023 | -0.21484 | -0.47966 | 0.42567 | -0.20173 |
| 1395                | 0.6121  | 0.6175  | -0.47525 | -0.19424 | -0.48749 | 0.43095 | -0.19884 |
| 1400                | 0.59816 | 0.62039 | -0.43932 | -0.17332 | -0.49457 | 0.43601 | -0.19575 |
| 1405                | 0.58428 | 0.62321 | -0.40257 | -0.15208 | -0.50088 | 0.44087 | -0.19246 |
| 1410                | 0.57048 | 0.62596 | -0.36515 | -0.13053 | -0.50637 | 0.44556 | -0.18897 |
| 1415                | 0.55682 | 0.62862 | -0.32721 | -0.1087  | -0.51102 | 0.4501  | -0.18528 |
| 1420                | 0.54335 | 0.63118 | -0.28889 | -0.08658 | -0.5148  | 0.4545  | -0.18139 |
| 1425                | 0.5301  | 0.63363 | -0.25033 | -0.06419 | -0.51767 | 0.45878 | -0.1773  |
| 1430                | 0.51712 | 0.63597 | -0.21167 | -0.04154 | -0.5196  | 0.46298 | -0.173   |
| 1435                | 0.50446 | 0.63817 | -0.17307 | -0.01864 | -0.52057 | 0.4671  | -0.16851 |
| 1440                | 0.49217 | 0.64024 | -0.13467 | 0.0045   | -0.52053 | 0.47116 | -0.16382 |
| 1445                | 0.48028 | 0.64215 | -0.09661 | 0.02786  | -0.51946 | 0.4752  | -0.15892 |
| 1450                | 0.46885 | 0.64391 | -0.05904 | 0.05144  | -0.51733 | 0.47922 | -0.15383 |
| 1455                | 0.45792 | 0.64548 | -0.02209 | 0.07522  | -0.51411 | 0.48325 | -0.14854 |
| 1460                | 0.44754 | 0.64688 | 0.01408  | 0.09919  | -0.50975 | 0.48732 | -0.14305 |
| 1465                | 0.43774 | 0.64808 | 0.04933  | 0.12335  | -0.50424 | 0.49143 | -0.13736 |
| 1470                | 0.42855 | 0.64906 | 0.08361  | 0.14764  | -0.49758 | 0.49559 | -0.13154 |
| 1475                | 0.41997 | 0.6498  | 0.11691  | 0.17201  | -0.4898  | 0.49979 | -0.12566 |
| 1480                | 0.41199 | 0.65025 | 0.14924  | 0.19638  | -0.48094 | 0.50402 | -0.11983 |
| 1485                | 0.4046  | 0.65039 | 0.1806   | 0.2207   | -0.47103 | 0.50827 | -0.11413 |
| 1490                | 0.39781 | 0.65018 | 0.211    | 0.2449   | -0.4601  | 0.51253 | -0.10866 |
| 1495                | 0.39161 | 0.6496  | 0.24043  | 0.26892  | -0.44819 | 0.51679 | -0.10352 |
| 1500                | 0.38599 | 0.64862 | 0.26889  | 0.29269  | -0.43534 | 0.52104 | -0.09879 |
| 1505                | 0.38096 | 0.64719 | 0.2964   | 0.31615  | -0.42158 | 0.52526 | -0.09457 |
| 1510                | 0.37651 | 0.6453  | 0.32295  | 0.33923  | -0.40693 | 0.52944 | -0.09095 |
| 1515                | 0.37264 | 0.6429  | 0.34854  | 0.36186  | -0.39144 | 0.53359 | -0.08803 |
| 1520                | 0.36933 | 0.63998 | 0.37315  | 0.38401  | -0.37512 | 0.53773 | -0.08583 |
| 1525                | 0.36653 | 0.63654 | 0.39667  | 0.40564  | -0.35794 | 0.54203 | -0.08422 |
| 1530                | 0.3642  | 0.63257 | 0.41901  | 0.42676  | -0.33984 | 0.54668 | -0.08304 |

Table 20: Normalized Legendre coefficients in  $\bar{K}N \rightarrow \Lambda\pi$  (5/7)

| Momentum<br>(MeV/c) | A1/A0   | A2/A0   | A3/A0   | A4/A0   | A5/A0    | A6/A0   | A7/A0    |
|---------------------|---------|---------|---------|---------|----------|---------|----------|
| 1535                | 0.36228 | 0.62809 | 0.44005 | 0.44733 | -0.3208  | 0.55185 | -0.08216 |
| 1540                | 0.36072 | 0.62309 | 0.45968 | 0.46736 | -0.30076 | 0.55773 | -0.08141 |
| 1545                | 0.35948 | 0.61757 | 0.47781 | 0.48683 | -0.27969 | 0.5645  | -0.08065 |
| 1550                | 0.35851 | 0.61154 | 0.49434 | 0.50572 | -0.25756 | 0.57231 | -0.07974 |
| 1555                | 0.35781 | 0.60502 | 0.50929 | 0.52405 | -0.23439 | 0.58116 | -0.07861 |
| 1560                | 0.35738 | 0.59804 | 0.52273 | 0.54186 | -0.21023 | 0.59098 | -0.07724 |
| 1565                | 0.35725 | 0.59063 | 0.53473 | 0.55915 | -0.18514 | 0.60169 | -0.07558 |
| 1570                | 0.35742 | 0.58282 | 0.54538 | 0.57597 | -0.15918 | 0.61322 | -0.07362 |
| 1575                | 0.35792 | 0.57463 | 0.55473 | 0.59234 | -0.13239 | 0.62549 | -0.07132 |
| 1580                | 0.35874 | 0.5661  | 0.56287 | 0.60828 | -0.10484 | 0.63843 | -0.06864 |
| 1585                | 0.35991 | 0.55725 | 0.56986 | 0.62383 | -0.07657 | 0.65196 | -0.06557 |
| 1590                | 0.36144 | 0.54811 | 0.57578 | 0.63899 | -0.04764 | 0.66601 | -0.06206 |
| 1595                | 0.36335 | 0.53871 | 0.5807  | 0.65382 | -0.0181  | 0.6805  | -0.05809 |
| 1600                | 0.36564 | 0.52909 | 0.5847  | 0.66832 | 0.01199  | 0.69536 | -0.05363 |
| 1605                | 0.36833 | 0.51926 | 0.58783 | 0.68253 | 0.04258  | 0.7105  | -0.04864 |
| 1610                | 0.37143 | 0.50926 | 0.59019 | 0.69647 | 0.07361  | 0.72586 | -0.0431  |
| 1615                | 0.37496 | 0.49911 | 0.59183 | 0.71017 | 0.10503  | 0.74137 | -0.03697 |
| 1620                | 0.37894 | 0.48885 | 0.59284 | 0.72365 | 0.13679  | 0.75693 | -0.03023 |
| 1625                | 0.38336 | 0.47851 | 0.59329 | 0.73695 | 0.16883  | 0.77249 | -0.02284 |
| 1630                | 0.38826 | 0.46811 | 0.59324 | 0.75008 | 0.2011   | 0.78797 | -0.01477 |
| 1635                | 0.39363 | 0.45767 | 0.59277 | 0.76308 | 0.23354  | 0.80328 | -0.00599 |
| 1640                | 0.39951 | 0.44724 | 0.59195 | 0.77597 | 0.26611  | 0.81836 | 0.00352  |
| 1645                | 0.40588 | 0.43684 | 0.59086 | 0.78878 | 0.29874  | 0.83312 | 0.01381  |
| 1650                | 0.41278 | 0.4265  | 0.58956 | 0.80153 | 0.33138  | 0.84751 | 0.0249   |
| 1655                | 0.42022 | 0.41624 | 0.58813 | 0.81425 | 0.36397  | 0.86143 | 0.03681  |
| 1660                | 0.4282  | 0.40614 | 0.58665 | 0.82695 | 0.39646  | 0.87483 | 0.04954  |
| 1665                | 0.43672 | 0.39632 | 0.58517 | 0.83966 | 0.42876  | 0.88768 | 0.06298  |
| 1670                | 0.44579 | 0.38689 | 0.58378 | 0.85238 | 0.46079  | 0.89994 | 0.07703  |
| 1675                | 0.45542 | 0.37799 | 0.58253 | 0.86511 | 0.49245  | 0.91158 | 0.09161  |
| 1680                | 0.46559 | 0.36972 | 0.5815  | 0.87787 | 0.52367  | 0.92256 | 0.1066   |
| 1685                | 0.47631 | 0.36223 | 0.58075 | 0.89067 | 0.55437  | 0.93285 | 0.12193  |
| 1690                | 0.48759 | 0.35562 | 0.58036 | 0.90351 | 0.58446  | 0.94242 | 0.13748  |
| 1695                | 0.49943 | 0.35002 | 0.58039 | 0.91642 | 0.61386  | 0.95122 | 0.15316  |
| 1700                | 0.51182 | 0.34555 | 0.58092 | 0.92938 | 0.64248  | 0.95923 | 0.16887  |
| 1705                | 0.52478 | 0.34234 | 0.58201 | 0.94243 | 0.67025  | 0.96642 | 0.18453  |
| 1710                | 0.5383  | 0.34049 | 0.58374 | 0.95556 | 0.69713  | 0.97277 | 0.20007  |
| 1715                | 0.55239 | 0.34002 | 0.58616 | 0.96883 | 0.72336  | 0.97841 | 0.21569  |
| 1720                | 0.56707 | 0.34092 | 0.58936 | 0.98229 | 0.74924  | 0.98349 | 0.23159  |
| 1725                | 0.58235 | 0.34319 | 0.59342 | 0.99599 | 0.77504  | 0.98814 | 0.24802  |
| 1730                | 0.59825 | 0.34683 | 0.59839 | 1.00998 | 0.80106  | 0.99252 | 0.26518  |
| 1735                | 0.61478 | 0.35185 | 0.60435 | 1.02432 | 0.82759  | 0.99678 | 0.28332  |
| 1740                | 0.63195 | 0.35823 | 0.61138 | 1.03905 | 0.85493  | 1.00106 | 0.30266  |
| 1745                | 0.64977 | 0.36598 | 0.61954 | 1.05422 | 0.88333  | 1.00549 | 0.32339  |

Table 21: Normalized Legendre coefficients in  $\bar{K}N \rightarrow \Lambda\pi$  (6/7)

| Momentum<br>(MeV/c) | A1/A0   | A2/A0   | A3/A0   | A4/A0   | A5/A0   | A6/A0   | A7/A0   |
|---------------------|---------|---------|---------|---------|---------|---------|---------|
| 1750                | 0.66822 | 0.37504 | 0.6288  | 1.06985 | 0.91282 | 1.01013 | 0.34556 |
| 1755                | 0.68725 | 0.38533 | 0.6391  | 1.08592 | 0.94333 | 1.01496 | 0.36913 |
| 1760                | 0.70685 | 0.39679 | 0.65037 | 1.10245 | 0.9748  | 1.01998 | 0.39406 |
| 1765                | 0.72695 | 0.40934 | 0.66257 | 1.11943 | 1.00714 | 1.02519 | 0.42031 |
| 1770                | 0.74754 | 0.42291 | 0.67563 | 1.13684 | 1.0403  | 1.03058 | 0.44784 |
| 1775                | 0.76857 | 0.43743 | 0.68947 | 1.15471 | 1.07419 | 1.03615 | 0.47661 |
| 1780                | 0.79    | 0.45282 | 0.70406 | 1.17301 | 1.10875 | 1.04191 | 0.50658 |
| 1785                | 0.81179 | 0.46902 | 0.71931 | 1.19174 | 1.14391 | 1.04784 | 0.53771 |
| 1790                | 0.83392 | 0.48594 | 0.73518 | 1.21092 | 1.17959 | 1.05394 | 0.56997 |
| 1795                | 0.85634 | 0.50352 | 0.75159 | 1.23052 | 1.21573 | 1.06022 | 0.60332 |
| 1800                | 0.87901 | 0.52169 | 0.76849 | 1.25055 | 1.25225 | 1.06666 | 0.63771 |
| 1805                | 0.9019  | 0.54038 | 0.78582 | 1.27101 | 1.28908 | 1.07326 | 0.6731  |
| 1810                | 0.92496 | 0.5595  | 0.80351 | 1.2919  | 1.32615 | 1.08003 | 0.70946 |
| 1815                | 0.94817 | 0.57899 | 0.82151 | 1.31321 | 1.36339 | 1.08695 | 0.74675 |
| 1820                | 0.97149 | 0.59878 | 0.83975 | 1.33493 | 1.40073 | 1.09403 | 0.78493 |
| 1825                | 0.99487 | 0.61879 | 0.85816 | 1.35707 | 1.4381  | 1.10125 | 0.82396 |
| 1830                | 1.01828 | 0.63895 | 0.8767  | 1.37963 | 1.47543 | 1.10863 | 0.86381 |
| 1835                | 1.04168 | 0.65919 | 0.89529 | 1.4026  | 1.51264 | 1.11616 | 0.90442 |
| 1840                | 1.06504 | 0.67943 | 0.91388 | 1.42598 | 1.54966 | 1.12382 | 0.94576 |
| 1845                | 1.08832 | 0.69962 | 0.93241 | 1.44973 | 1.58645 | 1.13162 | 0.98775 |

Table 22: Normalized Legendre coefficients in  $\overline{K}N \rightarrow \Lambda\pi$  (7/7)

| Momentum<br>(MeV/c) | A1/A0    | A2/A0   | A3/A0    | A4/A0    | A5/A0    | A6/A0    | A7/A0 | A8/A0 |
|---------------------|----------|---------|----------|----------|----------|----------|-------|-------|
| 435                 | 0.20268  | 0.89605 | 0.00315  | -0.02043 | 0.00013  | 1e-05    | 0     | 0     |
| 440                 | 0.2116   | 0.91169 | 0.00737  | -0.02297 | 2e-04    | 0        | 0     | 0     |
| 445                 | 0.21976  | 0.92725 | 0.01151  | -0.02554 | 0.00027  | -1e-05   | 0     | 0     |
| 450                 | 0.22691  | 0.94264 | 0.01546  | -0.02817 | 0.00033  | -2e-05   | 0     | 0     |
| 455                 | 0.23293  | 0.95777 | 0.0191   | -0.03089 | 4e-04    | -3e-05   | 0     | 0     |
| 460                 | 0.23762  | 0.97259 | 0.02233  | -0.03372 | 0.00046  | -4e-05   | 0     | 0     |
| 465                 | 0.24084  | 0.98722 | 0.025    | -0.03662 | 0.00053  | -5e-05   | 0     | 0     |
| 470                 | 0.24244  | 1.00183 | 0.02695  | -0.0395  | 0.00059  | -6e-05   | 0     | 0     |
| 475                 | 0.24243  | 1.0166  | 0.02804  | -0.0423  | 0.00065  | -7e-05   | 0     | 0     |
| 480                 | 0.2408   | 1.03171 | 0.0281   | -0.04494 | 0.00071  | -8e-05   | 0     | 0     |
| 485                 | 0.23759  | 1.04732 | 0.02704  | -0.04728 | 0.00076  | -8e-05   | 0     | 0     |
| 490                 | 0.23289  | 1.06364 | 0.02475  | -0.04917 | 0.00081  | -9e-05   | 0     | 0     |
| 495                 | 0.22693  | 1.08085 | 0.02112  | -0.05045 | 0.00086  | -1e-04   | 0     | 0     |
| 500                 | 0.21985  | 1.0991  | 0.01607  | -0.05099 | 0.00089  | -0.00011 | 0     | 0     |
| 505                 | 0.21186  | 1.11838 | 0.00962  | -0.05067 | 0.00092  | -0.00012 | 0     | 0     |
| 510                 | 0.20311  | 1.13865 | 0.0018   | -0.04938 | 0.00094  | -0.00012 | 0     | 0     |
| 515                 | 0.19378  | 1.15987 | -0.00734 | -0.04703 | 0.00095  | -0.00013 | 0     | 0     |
| 520                 | 0.18394  | 1.18199 | -0.01776 | -0.04353 | 0.00094  | -0.00013 | 0     | 0     |
| 525                 | 0.17362  | 1.20497 | -0.02941 | -0.03891 | 0.00092  | -0.00014 | 0     | 0     |
| 530                 | 0.16277  | 1.22874 | -0.04223 | -0.03321 | 0.00088  | -0.00014 | 1e-05 | 0     |
| 535                 | 0.15135  | 1.25326 | -0.05615 | -0.02646 | 0.00082  | -0.00014 | 1e-05 | 0     |
| 540                 | 0.13922  | 1.2785  | -0.07107 | -0.01873 | 0.00073  | -0.00014 | 1e-05 | 0     |
| 545                 | 0.12624  | 1.30447 | -0.08684 | -0.01017 | 0.00061  | -0.00013 | 1e-05 | 0     |
| 550                 | 0.1123   | 1.3312  | -0.10326 | -0.00094 | 0.00047  | -0.00012 | 1e-05 | 0     |
| 555                 | 0.09727  | 1.35871 | -0.12015 | 0.00879  | 0.00029  | -0.00011 | 1e-05 | 0     |
| 560                 | 0.08117  | 1.38699 | -0.13734 | 0.01891  | 7e-05    | -9e-05   | 1e-05 | 0     |
| 565                 | 0.064    | 1.41599 | -0.15466 | 0.02935  | -0.00019 | -7e-05   | 2e-05 | 0     |
| 570                 | 0.0459   | 1.44562 | -0.17197 | 0.04009  | -5e-04   | -5e-05   | 2e-05 | 0     |
| 575                 | 0.02704  | 1.47583 | -0.18911 | 0.05108  | -0.00085 | -2e-05   | 2e-05 | 0     |
| 580                 | 0.00769  | 1.50654 | -0.20595 | 0.06228  | -0.00126 | 2e-05    | 2e-05 | 0     |
| 585                 | -0.01183 | 1.53766 | -0.22246 | 0.07364  | -0.00172 | 6e-05    | 2e-05 | 0     |
| 590                 | -0.03118 | 1.56911 | -0.23858 | 0.08511  | -0.00224 | 0.00011  | 2e-05 | 0     |
| 595                 | -0.05002 | 1.60083 | -0.25425 | 0.09665  | -0.00282 | 0.00016  | 3e-05 | 0     |
| 600                 | -0.06802 | 1.63271 | -0.26943 | 0.10821  | -0.00346 | 0.00023  | 3e-05 | 0     |
| 605                 | -0.08492 | 1.66463 | -0.28414 | 0.1197   | -0.00417 | 3e-04    | 3e-05 | 0     |
| 610                 | -0.10045 | 1.69641 | -0.29846 | 0.131    | -0.00494 | 0.00038  | 3e-05 | 0     |
| 615                 | -0.11445 | 1.72786 | -0.31248 | 0.14199  | -0.00578 | 0.00047  | 3e-05 | 0     |
| 620                 | -0.12685 | 1.75882 | -0.32626 | 0.15255  | -0.00669 | 0.00057  | 3e-05 | 0     |
| 625                 | -0.13761 | 1.78907 | -0.3398  | 0.16263  | -0.00766 | 0.00068  | 3e-05 | 0     |
| 630                 | -0.14665 | 1.81843 | -0.353   | 0.17219  | -0.00869 | 8e-04    | 3e-05 | 0     |
| 635                 | -0.15404 | 1.84667 | -0.36578 | 0.18122  | -0.00977 | 0.00093  | 3e-05 | 0     |
| 640                 | -0.15984 | 1.8736  | -0.37806 | 0.18969  | -0.0109  | 0.00107  | 3e-05 | 0     |
| 645                 | -0.1641  | 1.89903 | -0.38974 | 0.19753  | -0.01207 | 0.00121  | 3e-05 | 0     |
| 650                 | -0.1668  | 1.92283 | -0.40077 | 0.20457  | -0.01326 | 0.00137  | 3e-05 | 0     |
| 655                 | -0.16802 | 1.94484 | -0.41108 | 0.2107   | -0.01447 | 0.00153  | 3e-05 | 0     |

Table 23: Normalized Legendre coefficients in  $K^-p \rightarrow \Sigma^- \pi^+$  (1/7)

| Momentum<br>(MeV/c) | A1/A0    | A2/A0   | A3/A0    | A4/A0    | A5/A0    | A6/A0    | A7/A0    | A8/A0    |
|---------------------|----------|---------|----------|----------|----------|----------|----------|----------|
| 660                 | -0.16778 | 1.96491 | -0.4206  | 0.21575  | -0.01567 | 0.0017   | 2e-05    | 0        |
| 665                 | -0.16609 | 1.98295 | -0.42932 | 0.21971  | -0.01684 | 0.00187  | 2e-05    | 1e-05    |
| 670                 | -0.16293 | 1.99895 | -0.4373  | 0.22266  | -0.01797 | 0.00204  | 1e-05    | 1e-05    |
| 675                 | -0.15835 | 2.01289 | -0.4446  | 0.2247   | -0.01902 | 0.00221  | 0        | 1e-05    |
| 680                 | -0.15235 | 2.02475 | -0.45128 | 0.22593  | -0.01997 | 0.00238  | -1e-05   | 1e-05    |
| 685                 | -0.14502 | 2.03452 | -0.45737 | 0.22638  | -0.02077 | 0.00255  | -2e-05   | 1e-05    |
| 690                 | -0.1364  | 2.04219 | -0.46282 | 0.22601  | -0.02139 | 0.0027   | -3e-05   | 1e-05    |
| 695                 | -0.12665 | 2.04773 | -0.46761 | 0.22477  | -0.02178 | 0.00284  | -4e-05   | 1e-05    |
| 700                 | -0.11594 | 2.05112 | -0.47172 | 0.22263  | -0.0219  | 0.00296  | -6e-05   | 1e-05    |
| 705                 | -0.10451 | 2.05233 | -0.47513 | 0.21958  | -0.0217  | 0.00305  | -8e-05   | 1e-05    |
| 710                 | -0.09257 | 2.05134 | -0.47789 | 0.21563  | -0.02111 | 0.00311  | -1e-04   | 1e-05    |
| 715                 | -0.08045 | 2.0481  | -0.48004 | 0.21082  | -0.02008 | 0.00314  | -0.00012 | 1e-05    |
| 720                 | -0.06841 | 2.04258 | -0.48164 | 0.20519  | -0.01853 | 0.00312  | -0.00015 | 1e-05    |
| 725                 | -0.05677 | 2.03476 | -0.4827  | 0.19876  | -0.01641 | 0.00305  | -0.00018 | 1e-05    |
| 730                 | -0.04577 | 2.02468 | -0.48321 | 0.19159  | -0.01364 | 0.00292  | -0.00021 | 1e-05    |
| 735                 | -0.03567 | 2.01241 | -0.48312 | 0.18371  | -0.01013 | 0.00271  | -0.00024 | 1e-05    |
| 740                 | -0.02666 | 1.99799 | -0.4824  | 0.17518  | -0.0058  | 0.00243  | -0.00028 | 1e-05    |
| 745                 | -0.01887 | 1.98148 | -0.48101 | 0.16603  | -0.00058 | 0.00205  | -0.00031 | 1e-05    |
| 750                 | -0.01239 | 1.96293 | -0.47891 | 0.15626  | 0.00561  | 0.00157  | -0.00035 | 1e-05    |
| 755                 | -0.00733 | 1.9424  | -0.47608 | 0.14587  | 0.01287  | 0.00098  | -0.00039 | 1e-05    |
| 760                 | -0.00369 | 1.91993 | -0.47246 | 0.13483  | 0.02128  | 0.00026  | -0.00043 | 0        |
| 765                 | -0.0015  | 1.8956  | -0.46801 | 0.12316  | 0.03091  | -0.00059 | -0.00048 | 0        |
| 770                 | -0.00083 | 1.86947 | -0.46257 | 0.1109   | 0.04184  | -0.0016  | -0.00052 | 0        |
| 775                 | -0.00169 | 1.84167 | -0.45593 | 0.09812  | 0.05414  | -0.00277 | -0.00056 | 0        |
| 780                 | -0.0042  | 1.81233 | -0.44791 | 0.0849   | 0.06785  | -0.0041  | -0.00061 | -1e-05   |
| 785                 | -0.0085  | 1.78162 | -0.43841 | 0.07136  | 0.08299  | -0.00562 | -0.00065 | -1e-05   |
| 790                 | -0.0149  | 1.74974 | -0.4273  | 0.05758  | 0.09958  | -0.00733 | -0.00068 | -2e-05   |
| 795                 | -0.02359 | 1.71687 | -0.41448 | 0.04365  | 0.11765  | -0.00925 | -0.00072 | -2e-05   |
| 800                 | -0.03492 | 1.68318 | -0.3999  | 0.02967  | 0.13718  | -0.01137 | -0.00074 | -3e-05   |
| 805                 | -0.04918 | 1.64882 | -0.38363 | 0.01571  | 0.15809  | -0.0137  | -0.00076 | -4e-05   |
| 810                 | -0.06654 | 1.61392 | -0.36573 | 0.00182  | 0.18032  | -0.01625 | -0.00077 | -4e-05   |
| 815                 | -0.08712 | 1.57864 | -0.34628 | -0.01193 | 0.20379  | -0.01901 | -0.00077 | -5e-05   |
| 820                 | -0.11012 | 1.54311 | -0.32533 | -0.02547 | 0.22841  | -0.02199 | -0.00075 | -6e-05   |
| 825                 | -0.13493 | 1.50749 | -0.30295 | -0.03874 | 0.25413  | -0.02519 | -0.00072 | -7e-05   |
| 830                 | -0.16027 | 1.47191 | -0.2792  | -0.05167 | 0.28087  | -0.02861 | -0.00068 | -8e-05   |
| 835                 | -0.18509 | 1.43652 | -0.25416 | -0.0642  | 0.30854  | -0.03226 | -0.00061 | -9e-05   |
| 840                 | -0.20852 | 1.40147 | -0.22789 | -0.07626 | 0.33709  | -0.03613 | -0.00053 | -1e-04   |
| 845                 | -0.23013 | 1.3669  | -0.20046 | -0.08779 | 0.36642  | -0.04024 | -0.00042 | -0.00012 |
| 850                 | -0.2499  | 1.33295 | -0.17192 | -0.09871 | 0.39647  | -0.04458 | -3e-04   | -0.00013 |
| 855                 | -0.26818 | 1.29977 | -0.14236 | -0.10898 | 0.42717  | -0.04916 | -0.00014 | -0.00015 |
| 860                 | -0.2854  | 1.2675  | -0.11182 | -0.11851 | 0.45844  | -0.05397 | 4e-05    | -0.00016 |
| 865                 | -0.30205 | 1.23628 | -0.08039 | -0.12725 | 0.4902   | -0.05903 | 0.00025  | -0.00018 |
| 870                 | -0.31869 | 1.20621 | -0.0481  | -0.13519 | 0.52231  | -0.06438 | 0.00049  | -2e-04   |
| 875                 | -0.33574 | 1.17732 | -0.01498 | -0.14236 | 0.5546   | -0.07012 | 0.00076  | -0.00021 |

Table 24: Normalized Legendre coefficients in  $K^-p \rightarrow \Sigma^- \pi^+$  (2/7)



| Momentum<br>(MeV/c) | A1/A0    | A2/A0   | A3/A0   | A4/A0    | A5/A0   | A6/A0    | A7/A0    | A8/A0    |
|---------------------|----------|---------|---------|----------|---------|----------|----------|----------|
| 880                 | -0.35356 | 1.14966 | 0.01893 | -0.14877 | 0.58687 | -0.07634 | 0.00107  | -0.00023 |
| 885                 | -0.37245 | 1.12329 | 0.05362 | -0.15447 | 0.61893 | -0.08312 | 0.00141  | -0.00025 |
| 890                 | -0.3926  | 1.09818 | 0.08898 | -0.15955 | 0.65061 | -0.09049 | 0.00179  | -0.00027 |
| 895                 | -0.41404 | 1.07429 | 0.12481 | -0.16417 | 0.68173 | -0.09828 | 0.00221  | -0.00029 |
| 900                 | -0.43679 | 1.05155 | 0.16084 | -0.16846 | 0.7122  | -0.10616 | 0.00266  | -0.00031 |
| 905                 | -0.46071 | 1.02994 | 0.1968  | -0.17253 | 0.74193 | -0.11383 | 0.00314  | -0.00033 |
| 910                 | -0.4856  | 1.00944 | 0.23246 | -0.17643 | 0.77089 | -0.12104 | 0.00366  | -0.00034 |
| 915                 | -0.51107 | 0.99007 | 0.26757 | -0.18017 | 0.79911 | -0.12764 | 0.00421  | -0.00035 |
| 920                 | -0.53674 | 0.97186 | 0.3019  | -0.18373 | 0.8266  | -0.13347 | 0.00478  | -0.00036 |
| 925                 | -0.56217 | 0.95486 | 0.33525 | -0.18707 | 0.85342 | -0.13846 | 0.00537  | -0.00036 |
| 930                 | -0.58681 | 0.9392  | 0.36744 | -0.19012 | 0.87966 | -0.14268 | 0.00598  | -0.00036 |
| 935                 | -0.61023 | 0.92501 | 0.39833 | -0.1928  | 0.9054  | -0.14621 | 0.00659  | -0.00035 |
| 940                 | -0.63197 | 0.91241 | 0.42775 | -0.19502 | 0.93074 | -0.14913 | 0.0072   | -0.00034 |
| 945                 | -0.65175 | 0.90149 | 0.45562 | -0.19679 | 0.95586 | -0.15152 | 0.0078   | -0.00031 |
| 950                 | -0.66926 | 0.89231 | 0.4819  | -0.19816 | 0.98094 | -0.15347 | 0.00838  | -0.00027 |
| 955                 | -0.68439 | 0.88494 | 0.50655 | -0.19918 | 1.00619 | -0.15508 | 0.00891  | -0.00022 |
| 960                 | -0.69707 | 0.87945 | 0.52952 | -0.19989 | 1.03181 | -0.15642 | 0.00939  | -0.00016 |
| 965                 | -0.70731 | 0.87589 | 0.55076 | -0.20033 | 1.05793 | -0.15758 | 0.0098   | -8e-05   |
| 970                 | -0.71516 | 0.87419 | 0.5703  | -0.20045 | 1.08454 | -0.15852 | 0.01012  | 2e-05    |
| 975                 | -0.7207  | 0.87429 | 0.58813 | -0.20021 | 1.11152 | -0.1592  | 0.01032  | 0.00013  |
| 980                 | -0.72394 | 0.87607 | 0.60419 | -0.1995  | 1.13868 | -0.1595  | 0.01035  | 0.00027  |
| 985                 | -0.72503 | 0.87939 | 0.61843 | -0.19819 | 1.16573 | -0.15928 | 0.01018  | 0.00043  |
| 990                 | -0.72394 | 0.88412 | 0.63075 | -0.19616 | 1.1924  | -0.15842 | 0.00978  | 0.00061  |
| 995                 | -0.72067 | 0.89012 | 0.64109 | -0.19327 | 1.21844 | -0.15676 | 0.0091   | 0.00081  |
| 1000                | -0.71516 | 0.89727 | 0.64936 | -0.1894  | 1.24357 | -0.15418 | 0.0081   | 0.00105  |
| 1005                | -0.70731 | 0.90541 | 0.6555  | -0.18445 | 1.26753 | -0.15055 | 0.00676  | 0.00131  |
| 1010                | -0.697   | 0.91431 | 0.65947 | -0.17846 | 1.29013 | -0.1459  | 0.00501  | 0.00161  |
| 1015                | -0.68411 | 0.92376 | 0.66132 | -0.17145 | 1.31127 | -0.14023 | 0.00282  | 0.00193  |
| 1020                | -0.66835 | 0.93356 | 0.66107 | -0.16347 | 1.3309  | -0.13354 | 0.00014  | 0.00228  |
| 1025                | -0.64976 | 0.94348 | 0.65877 | -0.15451 | 1.34895 | -0.12582 | -0.0031  | 0.00266  |
| 1030                | -0.62823 | 0.95334 | 0.65446 | -0.14459 | 1.36535 | -0.11708 | -0.00694 | 0.00307  |
| 1035                | -0.6038  | 0.96292 | 0.64817 | -0.13375 | 1.38003 | -0.10731 | -0.01143 | 0.00351  |
| 1040                | -0.57654 | 0.97201 | 0.63996 | -0.12199 | 1.39292 | -0.0965  | -0.01662 | 0.00397  |
| 1045                | -0.54672 | 0.9804  | 0.62985 | -0.10933 | 1.40396 | -0.08465 | -0.02256 | 0.00446  |
| 1050                | -0.51475 | 0.98795 | 0.61792 | -0.09577 | 1.41311 | -0.07177 | -0.02927 | 0.00498  |
| 1055                | -0.48114 | 0.99462 | 0.60434 | -0.08128 | 1.42048 | -0.05788 | -0.03657 | 0.00552  |
| 1060                | -0.44627 | 1.00047 | 0.58928 | -0.06579 | 1.42621 | -0.04301 | -0.04426 | 0.00608  |
| 1065                | -0.41097 | 1.00553 | 0.57295 | -0.04925 | 1.43042 | -0.02719 | -0.05212 | 0.00665  |
| 1070                | -0.37567 | 1.00983 | 0.55554 | -0.03158 | 1.43327 | -0.01044 | -0.05994 | 0.00724  |
| 1075                | -0.34091 | 1.01341 | 0.53725 | -0.01274 | 1.43488 | 0.00719  | -0.06751 | 0.00782  |
| 1080                | -0.30701 | 1.0163  | 0.51825 | 0.00733  | 1.4354  | 0.02567  | -0.07463 | 0.00841  |
| 1085                | -0.27413 | 1.01854 | 0.49874 | 0.0287   | 1.43496 | 0.04499  | -0.08107 | 0.009    |
| 1090                | -0.2425  | 1.02016 | 0.47892 | 0.0514   | 1.4337  | 0.06511  | -0.08666 | 0.00957  |

Table 25: Normalized Legendre coefficients in  $K^-p \rightarrow \Sigma^- \pi^+$  (3/7)

| Momentum<br>(MeV/c) | A1/A0    | A2/A0   | A3/A0   | A4/A0   | A5/A0   | A6/A0   | A7/A0    | A8/A0    |
|---------------------|----------|---------|---------|---------|---------|---------|----------|----------|
| 1095                | -0.21201 | 1.02123 | 0.45893 | 0.0754  | 1.43171 | 0.08607 | -0.09129 | 0.01013  |
| 1100                | -0.18239 | 1.02178 | 0.43894 | 0.10065 | 1.4291  | 0.10791 | -0.09489 | 0.01066  |
| 1105                | -0.15367 | 1.02189 | 0.41909 | 0.12708 | 1.42598 | 0.13065 | -0.09738 | 0.01114  |
| 1110                | -0.1254  | 1.02159 | 0.39954 | 0.15464 | 1.42243 | 0.15435 | -0.09869 | 0.01156  |
| 1115                | -0.09757 | 1.02096 | 0.38043 | 0.18328 | 1.41856 | 0.17903 | -0.09875 | 0.01192  |
| 1120                | -0.06982 | 1.02003 | 0.36193 | 0.21294 | 1.41446 | 0.20473 | -0.09748 | 0.0122   |
| 1125                | -0.04213 | 1.01887 | 0.34419 | 0.24357 | 1.41025 | 0.23151 | -0.0948  | 0.01238  |
| 1130                | -0.0142  | 1.01753 | 0.32732 | 0.27509 | 1.40599 | 0.25935 | -0.09067 | 0.01246  |
| 1135                | 0.01406  | 1.01605 | 0.31137 | 0.30741 | 1.40167 | 0.28815 | -0.08514 | 0.01242  |
| 1140                | 0.04282  | 1.01449 | 0.29633 | 0.3404  | 1.39724 | 0.31776 | -0.07828 | 0.01222  |
| 1145                | 0.0719   | 1.0129  | 0.28221 | 0.37395 | 1.39267 | 0.34804 | -0.07016 | 0.01185  |
| 1150                | 0.10146  | 1.01132 | 0.26901 | 0.40794 | 1.3879  | 0.37885 | -0.06087 | 0.01128  |
| 1155                | 0.13127  | 1.00979 | 0.25673 | 0.44225 | 1.38291 | 0.41003 | -0.05049 | 0.0105   |
| 1160                | 0.1612   | 1.00837 | 0.24537 | 0.47676 | 1.37764 | 0.44145 | -0.03908 | 0.00947  |
| 1165                | 0.19131  | 1.00711 | 0.23494 | 0.51136 | 1.37206 | 0.47296 | -0.02672 | 0.00818  |
| 1170                | 0.22156  | 1.00605 | 0.22546 | 0.54595 | 1.36612 | 0.5044  | -0.01351 | 0.0066   |
| 1175                | 0.25183  | 1.00528 | 0.21695 | 0.58048 | 1.35981 | 0.53559 | 0.00041  | 0.00471  |
| 1180                | 0.28191  | 1.00489 | 0.20947 | 0.61496 | 1.35311 | 0.56633 | 0.01488  | 0.00247  |
| 1185                | 0.31173  | 1.00498 | 0.20307 | 0.64937 | 1.34598 | 0.59642 | 0.02974  | -0.00015 |
| 1190                | 0.34118  | 1.00562 | 0.1978  | 0.68368 | 1.33842 | 0.62566 | 0.04483  | -0.00318 |
| 1195                | 0.37021  | 1.0069  | 0.1937  | 0.71789 | 1.33041 | 0.65385 | 0.05998  | -0.00664 |
| 1200                | 0.39843  | 1.00892 | 0.19083 | 0.75199 | 1.32192 | 0.6808  | 0.07505  | -0.01057 |
| 1205                | 0.42584  | 1.01177 | 0.18923 | 0.78595 | 1.31293 | 0.7063  | 0.08986  | -0.015   |
| 1210                | 0.45231  | 1.01553 | 0.18896 | 0.81978 | 1.30344 | 0.7302  | 0.10428  | -0.01995 |
| 1215                | 0.47765  | 1.02033 | 0.19014 | 0.85355 | 1.29349 | 0.7525  | 0.11823  | -0.02545 |
| 1220                | 0.50177  | 1.02629 | 0.19287 | 0.88735 | 1.28312 | 0.77325 | 0.13164  | -0.03151 |
| 1225                | 0.52457  | 1.03352 | 0.19729 | 0.92127 | 1.27241 | 0.79248 | 0.14447  | -0.03814 |
| 1230                | 0.54599  | 1.04214 | 0.2035  | 0.95541 | 1.26139 | 0.81024 | 0.15665  | -0.04537 |
| 1235                | 0.56609  | 1.05228 | 0.21163 | 0.98984 | 1.25012 | 0.82657 | 0.16812  | -0.05321 |
| 1240                | 0.5847   | 1.06406 | 0.2218  | 1.02465 | 1.23865 | 0.84152 | 0.17883  | -0.06168 |
| 1245                | 0.60195  | 1.07759 | 0.23413 | 1.05995 | 1.22704 | 0.85513 | 0.18872  | -0.07079 |
| 1250                | 0.61786  | 1.09296 | 0.24867 | 1.09575 | 1.21531 | 0.86741 | 0.19769  | -0.08061 |
| 1255                | 0.63245  | 1.11008 | 0.26523 | 1.13191 | 1.20336 | 0.87829 | 0.20553  | -0.09138 |
| 1260                | 0.64572  | 1.1288  | 0.28356 | 1.16821 | 1.19107 | 0.88763 | 0.21202  | -0.10339 |
| 1265                | 0.65767  | 1.14902 | 0.30341 | 1.20443 | 1.1783  | 0.89534 | 0.2169   | -0.11694 |
| 1270                | 0.6683   | 1.17065 | 0.32457 | 1.24045 | 1.16511 | 0.90145 | 0.22018  | -0.13214 |
| 1275                | 0.67758  | 1.19375 | 0.34687 | 1.27626 | 1.15175 | 0.90623 | 0.22212  | -0.14893 |
| 1280                | 0.68536  | 1.21833 | 0.37014 | 1.31188 | 1.1385  | 0.90994 | 0.22304  | -0.16725 |
| 1285                | 0.69167  | 1.24444 | 0.39422 | 1.34729 | 1.12563 | 0.91284 | 0.22321  | -0.187   |
| 1290                | 0.69645  | 1.27212 | 0.41894 | 1.38249 | 1.11339 | 0.91518 | 0.22293  | -0.20808 |
| 1295                | 0.69969  | 1.30139 | 0.44417 | 1.41745 | 1.10188 | 0.91705 | 0.22235  | -0.23029 |
| 1300                | 0.70139  | 1.33231 | 0.46975 | 1.45211 | 1.09119 | 0.91853 | 0.22163  | -0.25337 |
| 1305                | 0.70159  | 1.36489 | 0.49554 | 1.48643 | 1.0814  | 0.91967 | 0.22091  | -0.27708 |
| 1310                | 0.70037  | 1.39918 | 0.52138 | 1.52037 | 1.07258 | 0.92056 | 0.22033  | -0.30119 |
| 1315                | 0.69788  | 1.43522 | 0.54714 | 1.55387 | 1.06482 | 0.92125 | 0.22005  | -0.32545 |

Table 26: Normalized Legendre coefficients in  $K^-p \rightarrow \Sigma^- \pi^+$  (4/7)

| Momentum<br>(MeV/c) | A1/A0   | A2/A0   | A3/A0   | A4/A0   | A5/A0   | A6/A0   | A7/A0   | A8/A0    |
|---------------------|---------|---------|---------|---------|---------|---------|---------|----------|
| 1320                | 0.69426 | 1.47301 | 0.57267 | 1.5869  | 1.05819 | 0.92182 | 0.22018 | -0.34964 |
| 1325                | 0.68978 | 1.51246 | 0.59789 | 1.61947 | 1.05272 | 0.92232 | 0.22064 | -0.37368 |
| 1330                | 0.68469 | 1.55333 | 0.62279 | 1.65156 | 1.04837 | 0.92281 | 0.22135 | -0.39738 |
| 1335                | 0.6793  | 1.59543 | 0.64739 | 1.68314 | 1.04513 | 0.92337 | 0.22227 | -0.4205  |
| 1340                | 0.67393 | 1.63853 | 0.67168 | 1.71418 | 1.04298 | 0.92406 | 0.22335 | -0.44283 |
| 1345                | 0.66891 | 1.68242 | 0.69567 | 1.74465 | 1.04188 | 0.92496 | 0.22454 | -0.46412 |
| 1350                | 0.66455 | 1.72688 | 0.71937 | 1.77453 | 1.04181 | 0.92613 | 0.22578 | -0.48416 |
| 1355                | 0.66117 | 1.7717  | 0.74277 | 1.80377 | 1.04274 | 0.92764 | 0.22704 | -0.50271 |
| 1360                | 0.65897 | 1.81664 | 0.76591 | 1.83233 | 1.04468 | 0.92957 | 0.2283  | -0.51949 |
| 1365                | 0.65815 | 1.86145 | 0.78889 | 1.86002 | 1.0477  | 0.93203 | 0.2298  | -0.53402 |
| 1370                | 0.65879 | 1.90585 | 0.81186 | 1.88663 | 1.05191 | 0.93512 | 0.23178 | -0.54579 |
| 1375                | 0.66083 | 1.94962 | 0.8348  | 1.91201 | 1.05725 | 0.93889 | 0.23444 | -0.55462 |
| 1380                | 0.66406 | 1.9926  | 0.85756 | 1.93612 | 1.06349 | 0.94336 | 0.23782 | -0.56076 |
| 1385                | 0.66812 | 2.03463 | 0.87996 | 1.95888 | 1.07037 | 0.94852 | 0.24197 | -0.56449 |
| 1390                | 0.67247 | 2.07556 | 0.90183 | 1.98025 | 1.07762 | 0.95437 | 0.24693 | -0.5661  |
| 1395                | 0.67646 | 2.11524 | 0.92297 | 2.00017 | 1.08501 | 0.9609  | 0.25275 | -0.56588 |
| 1400                | 0.67917 | 2.15351 | 0.94322 | 2.01858 | 1.09227 | 0.96812 | 0.25948 | -0.56411 |
| 1405                | 0.67999 | 2.19022 | 0.96239 | 2.03543 | 1.09914 | 0.97601 | 0.26715 | -0.56106 |
| 1410                | 0.67813 | 2.2252  | 0.98032 | 2.05066 | 1.10537 | 0.98459 | 0.27582 | -0.55704 |
| 1415                | 0.67307 | 2.25832 | 0.99681 | 2.06423 | 1.11071 | 0.99384 | 0.28552 | -0.55231 |
| 1420                | 0.66456 | 2.28945 | 1.01176 | 2.07609 | 1.11496 | 1.00374 | 0.29628 | -0.54712 |
| 1425                | 0.65267 | 2.31863 | 1.02525 | 2.08636 | 1.11811 | 1.01425 | 0.30798 | -0.54148 |
| 1430                | 0.6378  | 2.34595 | 1.03744 | 2.09517 | 1.12022 | 1.02527 | 0.32046 | -0.53535 |
| 1435                | 0.62062 | 2.37149 | 1.04848 | 2.10265 | 1.12135 | 1.03672 | 0.33357 | -0.52871 |
| 1440                | 0.60209 | 2.39534 | 1.05852 | 2.10894 | 1.12156 | 1.04854 | 0.34718 | -0.52152 |
| 1445                | 0.5832  | 2.41757 | 1.06772 | 2.11416 | 1.1209  | 1.06063 | 0.36112 | -0.51375 |
| 1450                | 0.56496 | 2.43828 | 1.07622 | 2.11846 | 1.11943 | 1.07293 | 0.37526 | -0.50535 |
| 1455                | 0.54826 | 2.45754 | 1.08418 | 2.12197 | 1.1172  | 1.08535 | 0.38943 | -0.49631 |
| 1460                | 0.53374 | 2.47544 | 1.09175 | 2.12481 | 1.11428 | 1.09782 | 0.40349 | -0.48658 |
| 1465                | 0.52181 | 2.49206 | 1.09908 | 2.12713 | 1.11072 | 1.11025 | 0.41731 | -0.47614 |
| 1470                | 0.51254 | 2.50744 | 1.10619 | 2.12895 | 1.10663 | 1.12251 | 0.4309  | -0.46499 |
| 1475                | 0.50575 | 2.52157 | 1.11304 | 2.13027 | 1.10217 | 1.13444 | 0.44441 | -0.4532  |
| 1480                | 0.50085 | 2.53446 | 1.11958 | 2.13104 | 1.09748 | 1.14586 | 0.45799 | -0.44082 |
| 1485                | 0.49715 | 2.5461  | 1.12576 | 2.13126 | 1.09271 | 1.15662 | 0.47178 | -0.4279  |
| 1490                | 0.49385 | 2.55652 | 1.13152 | 2.13089 | 1.08803 | 1.16654 | 0.48593 | -0.4145  |
| 1495                | 0.49019 | 2.56569 | 1.13682 | 2.12991 | 1.08357 | 1.17545 | 0.50059 | -0.40067 |
| 1500                | 0.48551 | 2.57364 | 1.14159 | 2.1283  | 1.07949 | 1.1832  | 0.51591 | -0.38647 |
| 1505                | 0.47939 | 2.58035 | 1.14579 | 2.12603 | 1.07594 | 1.18959 | 0.53203 | -0.37195 |
| 1510                | 0.47148 | 2.58582 | 1.14937 | 2.12307 | 1.07308 | 1.19448 | 0.5491  | -0.35716 |
| 1515                | 0.46175 | 2.59007 | 1.15228 | 2.11941 | 1.07105 | 1.1977  | 0.56728 | -0.34216 |
| 1520                | 0.45033 | 2.59313 | 1.15453 | 2.11509 | 1.06998 | 1.19914 | 0.58667 | -0.32702 |
| 1525                | 0.43753 | 2.5951  | 1.15631 | 2.11032 | 1.06994 | 1.19888 | 0.60734 | -0.31178 |
| 1530                | 0.42376 | 2.59609 | 1.15782 | 2.10533 | 1.071   | 1.19702 | 0.62932 | -0.29653 |
| 1535                | 0.40952 | 2.59624 | 1.15926 | 2.10037 | 1.07322 | 1.19365 | 0.65266 | -0.28133 |

Table 27: Normalized Legendre coefficients in  $K^-p \rightarrow \Sigma^- \pi^+$  (5/7)

| Momentum<br>(MeV/c) | A1/A0   | A2/A0   | A3/A0   | A4/A0   | A5/A0   | A6/A0   | A7/A0   | A8/A0    |
|---------------------|---------|---------|---------|---------|---------|---------|---------|----------|
| 1540                | 0.39543 | 2.59565 | 1.16083 | 2.09565 | 1.07667 | 1.18887 | 0.6774  | -0.26624 |
| 1545                | 0.38215 | 2.59444 | 1.16275 | 2.09142 | 1.08141 | 1.18276 | 0.7036  | -0.25134 |
| 1550                | 0.37039 | 2.59273 | 1.1652  | 2.08789 | 1.08751 | 1.17544 | 0.73127 | -0.2367  |
| 1555                | 0.36091 | 2.59062 | 1.16833 | 2.08526 | 1.09503 | 1.16716 | 0.76032 | -0.22237 |
| 1560                | 0.35456 | 2.58822 | 1.17224 | 2.08366 | 1.10406 | 1.15822 | 0.79059 | -0.20842 |
| 1565                | 0.35177 | 2.58562 | 1.17705 | 2.08327 | 1.11465 | 1.14894 | 0.82195 | -0.19492 |
| 1570                | 0.35337 | 2.58293 | 1.18288 | 2.08422 | 1.1269  | 1.13961 | 0.85423 | -0.18192 |
| 1575                | 0.35961 | 2.58025 | 1.18983 | 2.08669 | 1.14085 | 1.13056 | 0.88728 | -0.1695  |
| 1580                | 0.37063 | 2.57768 | 1.19803 | 2.09082 | 1.1566  | 1.12209 | 0.92096 | -0.1577  |
| 1585                | 0.3863  | 2.57533 | 1.20758 | 2.09678 | 1.17421 | 1.1145  | 0.95511 | -0.1466  |
| 1590                | 0.40627 | 2.57329 | 1.2186  | 2.10471 | 1.19376 | 1.10811 | 0.98957 | -0.13626 |
| 1595                | 0.43008 | 2.57166 | 1.2312  | 2.11477 | 1.21531 | 1.10322 | 1.0242  | -0.12673 |
| 1600                | 0.45695 | 2.57056 | 1.2455  | 2.12712 | 1.23895 | 1.10014 | 1.05885 | -0.11809 |
| 1605                | 0.48626 | 2.57007 | 1.2616  | 2.14191 | 1.26474 | 1.09918 | 1.09336 | -0.1104  |
| 1610                | 0.51735 | 2.57029 | 1.27959 | 2.15926 | 1.29271 | 1.1006  | 1.12758 | -0.1037  |
| 1615                | 0.54962 | 2.57116 | 1.2992  | 2.17896 | 1.3226  | 1.10434 | 1.16131 | -0.09794 |
| 1620                | 0.58245 | 2.57256 | 1.32004 | 2.20065 | 1.35402 | 1.11019 | 1.19434 | -0.09302 |
| 1625                | 0.61536 | 2.5744  | 1.34172 | 2.224   | 1.38657 | 1.11794 | 1.22646 | -0.08883 |
| 1630                | 0.64786 | 2.57654 | 1.36383 | 2.24863 | 1.41985 | 1.12739 | 1.25746 | -0.08529 |
| 1635                | 0.67945 | 2.57889 | 1.38599 | 2.27422 | 1.45346 | 1.13832 | 1.28713 | -0.08227 |
| 1640                | 0.70969 | 2.58132 | 1.40779 | 2.30039 | 1.48701 | 1.15051 | 1.31525 | -0.07969 |
| 1645                | 0.73811 | 2.58373 | 1.42884 | 2.32681 | 1.52009 | 1.16377 | 1.34161 | -0.07744 |
| 1650                | 0.7643  | 2.58599 | 1.44873 | 2.35312 | 1.55232 | 1.17789 | 1.36601 | -0.07541 |
| 1655                | 0.78784 | 2.58801 | 1.46709 | 2.37897 | 1.58329 | 1.19264 | 1.38822 | -0.07352 |
| 1660                | 0.80845 | 2.58964 | 1.4836  | 2.40404 | 1.61266 | 1.20785 | 1.40808 | -0.07166 |
| 1665                | 0.8259  | 2.59072 | 1.49807 | 2.42802 | 1.64013 | 1.22332 | 1.42543 | -0.06977 |
| 1670                | 0.84003 | 2.5911  | 1.51034 | 2.45063 | 1.6654  | 1.2389  | 1.44012 | -0.06776 |
| 1675                | 0.85087 | 2.59061 | 1.52021 | 2.47156 | 1.68818 | 1.25439 | 1.45202 | -0.06558 |
| 1680                | 0.85853 | 2.58908 | 1.52752 | 2.49054 | 1.7082  | 1.26964 | 1.46098 | -0.06314 |
| 1685                | 0.86321 | 2.58636 | 1.53208 | 2.50725 | 1.72514 | 1.28447 | 1.46686 | -0.06037 |
| 1690                | 0.86521 | 2.58228 | 1.53373 | 2.52141 | 1.73872 | 1.29869 | 1.4695  | -0.05719 |
| 1695                | 0.86497 | 2.57669 | 1.53227 | 2.53272 | 1.74866 | 1.31215 | 1.46878 | -0.05354 |
| 1700                | 0.86261 | 2.56941 | 1.52753 | 2.54089 | 1.75465 | 1.32465 | 1.46453 | -0.04935 |
| 1705                | 0.85865 | 2.5603  | 1.51934 | 2.54562 | 1.7564  | 1.33604 | 1.45663 | -0.04453 |
| 1710                | 0.85338 | 2.54921 | 1.50758 | 2.54666 | 1.75368 | 1.34611 | 1.44499 | -0.03906 |
| 1715                | 0.84709 | 2.53615 | 1.49237 | 2.54388 | 1.74639 | 1.35461 | 1.42984 | -0.03313 |
| 1720                | 0.83998 | 2.52115 | 1.4739  | 2.5372  | 1.73451 | 1.36127 | 1.41148 | -0.02693 |
| 1725                | 0.83223 | 2.50424 | 1.45236 | 2.52653 | 1.718   | 1.36581 | 1.3902  | -0.02071 |
| 1730                | 0.82398 | 2.48546 | 1.42794 | 2.51179 | 1.69681 | 1.36795 | 1.36629 | -0.01468 |
| 1735                | 0.81532 | 2.46484 | 1.40083 | 2.49289 | 1.67092 | 1.36742 | 1.34005 | -0.00906 |
| 1740                | 0.80635 | 2.4424  | 1.37121 | 2.46973 | 1.6403  | 1.36394 | 1.31177 | -0.00407 |
| 1745                | 0.79717 | 2.4182  | 1.33927 | 2.44227 | 1.60491 | 1.35727 | 1.28174 | 8e-05    |
| 1750                | 0.78787 | 2.39228 | 1.30516 | 2.41059 | 1.56494 | 1.34739 | 1.25012 | 0.00337  |
| 1755                | 0.77864 | 2.36474 | 1.26903 | 2.37487 | 1.52061 | 1.33437 | 1.21704 | 0.00581  |

Table 28: Normalized Legendre coefficients in  $K^-p \rightarrow \Sigma^- \pi^+$  (6/7)

| Momentum<br>(MeV/c) | A1/A0   | A2/A0   | A3/A0   | A4/A0   | A5/A0   | A6/A0   | A7/A0   | A8/A0    |
|---------------------|---------|---------|---------|---------|---------|---------|---------|----------|
| 1760                | 0.76947 | 2.33565 | 1.231   | 2.33528 | 1.47217 | 1.31829 | 1.18262 | 0.00745  |
| 1765                | 0.76063 | 2.3051  | 1.19124 | 2.29197 | 1.41987 | 1.29923 | 1.14697 | 0.00832  |
| 1770                | 0.75229 | 2.27315 | 1.14986 | 2.24514 | 1.36393 | 1.27726 | 1.11021 | 0.00845  |
| 1775                | 0.74462 | 2.23989 | 1.10702 | 2.19493 | 1.3046  | 1.25247 | 1.07248 | 0.00788  |
| 1780                | 0.73776 | 2.20541 | 1.06285 | 2.14153 | 1.24212 | 1.22492 | 1.03388 | 0.00663  |
| 1785                | 0.73178 | 2.16977 | 1.0175  | 2.0851  | 1.17673 | 1.1947  | 0.99455 | 0.00475  |
| 1790                | 0.72674 | 2.13307 | 0.9711  | 2.02582 | 1.10867 | 1.16189 | 0.95459 | 0.00226  |
| 1795                | 0.7226  | 2.09537 | 0.9238  | 1.96385 | 1.03819 | 1.12655 | 0.91414 | -0.00079 |
| 1800                | 0.7193  | 2.05676 | 0.87573 | 1.89936 | 0.96551 | 1.08878 | 0.8733  | -0.00439 |
| 1805                | 0.71674 | 2.01732 | 0.82704 | 1.83253 | 0.89088 | 1.04864 | 0.83221 | -0.00849 |
| 1810                | 0.71485 | 1.97712 | 0.77787 | 1.76351 | 0.81455 | 1.00621 | 0.79099 | -0.01305 |
| 1815                | 0.7135  | 1.93625 | 0.72835 | 1.69249 | 0.73675 | 0.96158 | 0.74975 | -0.01806 |
| 1820                | 0.71257 | 1.89479 | 0.67863 | 1.61963 | 0.65772 | 0.91481 | 0.70861 | -0.02347 |
| 1825                | 0.71198 | 1.85282 | 0.62885 | 1.5451  | 0.5777  | 0.86598 | 0.66769 | -0.02924 |
| 1830                | 0.71165 | 1.81041 | 0.57915 | 1.46907 | 0.49694 | 0.81518 | 0.62713 | -0.03536 |
| 1835                | 0.7115  | 1.76765 | 0.52966 | 1.39172 | 0.41567 | 0.76248 | 0.58703 | -0.04177 |
| 1840                | 0.71149 | 1.72461 | 0.48053 | 1.3132  | 0.33413 | 0.70795 | 0.54752 | -0.04846 |
| 1845                | 0.71158 | 1.68139 | 0.43186 | 1.23376 | 0.25256 | 0.65182 | 0.50865 | -0.05537 |

Table 29: Normalized Legendre coefficients in  $K^-p \rightarrow \Sigma^- \pi^+$  (7/7)

| Momentum<br>(MeV/c) | A1/A0    | A2/A0   | A3/A0    | A4/A0    | A5/A0 | A6/A0 | A7/A0 | A8/A0 |
|---------------------|----------|---------|----------|----------|-------|-------|-------|-------|
| 435                 | 0.01082  | 1.10989 | 0.01663  | -0.00335 | 0     | 0     | 0     | 0     |
| 440                 | -0.01888 | 1.07693 | -0.00805 | -0.01206 | 0     | 0     | 0     | 0     |
| 445                 | -0.04853 | 1.04408 | -0.03276 | -0.02075 | 0     | 0     | 0     | 0     |
| 450                 | -0.07803 | 1.01152 | -0.0575  | -0.02944 | 0     | 0     | 0     | 0     |
| 455                 | -0.10733 | 0.97938 | -0.0823  | -0.03809 | 0     | 0     | 0     | 0     |
| 460                 | -0.13633 | 0.9478  | -0.10716 | -0.0467  | 0     | 0     | 0     | 0     |
| 465                 | -0.16491 | 0.91681 | -0.13197 | -0.0552  | 0     | 0     | 0     | 0     |
| 470                 | -0.19294 | 0.88642 | -0.15661 | -0.06351 | 0     | 0     | 0     | 0     |
| 475                 | -0.2203  | 0.85665 | -0.18094 | -0.07154 | 0     | 0     | 0     | 0     |
| 480                 | -0.24683 | 0.82754 | -0.20479 | -0.07921 | 0     | 0     | 0     | 0     |
| 485                 | -0.27226 | 0.79925 | -0.22775 | -0.08632 | 0     | 0     | 0     | 0     |
| 490                 | -0.29631 | 0.77198 | -0.24937 | -0.09267 | 0     | 0     | 0     | 0     |
| 495                 | -0.31868 | 0.74592 | -0.26919 | -0.09804 | 0     | 0     | 0     | 0     |
| 500                 | -0.33912 | 0.72125 | -0.28682 | -0.10221 | 0     | 0     | 0     | 0     |
| 505                 | -0.35756 | 0.69815 | -0.30212 | -0.10482 | 0     | 0     | 0     | 0     |
| 510                 | -0.37395 | 0.67677 | -0.31501 | -0.10547 | 0     | 0     | 0     | 0     |
| 515                 | -0.38825 | 0.65729 | -0.32543 | -0.10379 | 0     | 0     | 0     | 0     |
| 520                 | -0.40045 | 0.63982 | -0.33324 | -0.09964 | 0     | 0     | 0     | 0     |
| 525                 | -0.41054 | 0.62436 | -0.33823 | -0.09347 | 0     | 0     | 0     | 0     |
| 530                 | -0.41855 | 0.61093 | -0.34015 | -0.0858  | 0     | 0     | 0     | 0     |
| 535                 | -0.42447 | 0.59951 | -0.33876 | -0.07716 | 0     | 0     | 0     | 0     |
| 540                 | -0.42842 | 0.59011 | -0.33407 | -0.06792 | 0     | 0     | 0     | 0     |
| 545                 | -0.43073 | 0.5827  | -0.32663 | -0.05813 | 0     | 0     | 0     | 0     |
| 550                 | -0.43174 | 0.57727 | -0.31706 | -0.04781 | 0     | 0     | 0     | 0     |
| 555                 | -0.4318  | 0.57379 | -0.30599 | -0.03697 | 0     | 0     | 0     | 0     |
| 560                 | -0.43126 | 0.57219 | -0.29405 | -0.0257  | 0     | 0     | 0     | 0     |
| 565                 | -0.43044 | 0.57227 | -0.28185 | -0.01436 | 0     | 0     | 0     | 0     |
| 570                 | -0.4298  | 0.57397 | -0.26991 | -0.00328 | 0     | 0     | 0     | 0     |
| 575                 | -0.42982 | 0.57729 | -0.25874 | 0.0072   | 0     | 0     | 0     | 0     |
| 580                 | -0.4308  | 0.58214 | -0.24872 | 0.01687  | 0     | 0     | 0     | 0     |
| 585                 | -0.4328  | 0.58835 | -0.2401  | 0.02571  | 0     | 0     | 0     | 0     |
| 590                 | -0.43612 | 0.59583 | -0.23321 | 0.03376  | 0     | 0     | 0     | 0     |
| 595                 | -0.44115 | 0.6045  | -0.22839 | 0.04108  | 0     | 0     | 0     | 0     |
| 600                 | -0.4482  | 0.61432 | -0.22597 | 0.04772  | 0     | 0     | 0     | 0     |
| 605                 | -0.45692 | 0.62534 | -0.22614 | 0.0535   | 0     | 0     | 0     | 0     |
| 610                 | -0.46673 | 0.63752 | -0.22906 | 0.05801  | 0     | 0     | 0     | 0     |
| 615                 | -0.47702 | 0.65085 | -0.23489 | 0.06082  | 0     | 0     | 0     | 0     |
| 620                 | -0.48723 | 0.66531 | -0.24375 | 0.06153  | 0     | 0     | 0     | 0     |
| 625                 | -0.4968  | 0.68072 | -0.25539 | 0.06011  | 0     | 0     | 0     | 0     |
| 630                 | -0.50526 | 0.69682 | -0.26923 | 0.05678  | 0     | 0     | 0     | 0     |
| 635                 | -0.51223 | 0.71341 | -0.28474 | 0.05178  | 0     | 0     | 0     | 0     |
| 640                 | -0.51759 | 0.73044 | -0.30159 | 0.04536  | 0     | 0     | 0     | 0     |
| 645                 | -0.52116 | 0.74789 | -0.31929 | 0.0379   | 0     | 0     | 0     | 0     |
| 650                 | -0.52267 | 0.76582 | -0.33727 | 0.02987  | 0     | 0     | 0     | 0     |
| 655                 | -0.52186 | 0.78423 | -0.35493 | 0.02172  | 0     | 0     | 0     | 0     |

Table 30: Normalized Legendre coefficients in  $K^-p \rightarrow \Sigma^0\pi^0$  (1/2)

| Momentum<br>(MeV/c) | A1/A0    | A2/A0   | A3/A0    | A4/A0    | A5/A0 | A6/A0 | A7/A0 | A8/A0 |
|---------------------|----------|---------|----------|----------|-------|-------|-------|-------|
| 660                 | -0.51846 | 0.80318 | -0.3717  | 0.01394  | 0     | 0     | 0     | 0     |
| 665                 | -0.51218 | 0.82275 | -0.387   | 0.007    | 0     | 0     | 0     | 0     |
| 670                 | -0.50273 | 0.84317 | -0.40028 | 0.00144  | 0     | 0     | 0     | 0     |
| 675                 | -0.48982 | 0.86469 | -0.41096 | -0.0022  | 0     | 0     | 0     | 0     |
| 680                 | -0.47326 | 0.88743 | -0.41875 | -0.00347 | 0     | 0     | 0     | 0     |
| 685                 | -0.45292 | 0.91119 | -0.42381 | -0.0022  | 0     | 0     | 0     | 0     |
| 690                 | -0.42867 | 0.93557 | -0.42646 | 0.00161  | 0     | 0     | 0     | 0     |
| 695                 | -0.40062 | 0.96016 | -0.42703 | 0.00789  | 0     | 0     | 0     | 0     |
| 700                 | -0.36903 | 0.98453 | -0.42585 | 0.01652  | 0     | 0     | 0     | 0     |
| 705                 | -0.33405 | 1.00813 | -0.42325 | 0.02726  | 0     | 0     | 0     | 0     |
| 710                 | -0.29565 | 1.03016 | -0.41947 | 0.03953  | 0     | 0     | 0     | 0     |
| 715                 | -0.25378 | 1.0498  | -0.41477 | 0.05274  | 0     | 0     | 0     | 0     |
| 720                 | -0.20851 | 1.06626 | -0.40938 | 0.06618  | 0     | 0     | 0     | 0     |
| 725                 | -0.16053 | 1.07916 | -0.40351 | 0.07896  | 0     | 0     | 0     | 0     |
| 730                 | -0.11059 | 1.08856 | -0.39716 | 0.09047  | 0     | 0     | 0     | 0     |
| 735                 | -0.05947 | 1.09453 | -0.3903  | 0.10015  | 0     | 0     | 0     | 0     |
| 740                 | -0.00792 | 1.09717 | -0.38288 | 0.10747  | 0     | 0     | 0     | 0     |
| 745                 | 0.0433   | 1.09656 | -0.37485 | 0.11203  | 0     | 0     | 0     | 0     |
| 750                 | 0.09344  | 1.09277 | -0.36603 | 0.11403  | 0     | 0     | 0     | 0     |
| 755                 | 0.14178  | 1.0859  | -0.35625 | 0.11383  | 0     | 0     | 0     | 0     |
| 760                 | 0.18761  | 1.07615 | -0.34549 | 0.1117   | 0     | 0     | 0     | 0     |
| 765                 | 0.23037  | 1.06383 | -0.33392 | 0.10794  | 0     | 0     | 0     | 0     |
| 770                 | 0.26959  | 1.04936 | -0.32217 | 0.1028   | 0     | 0     | 0     | 0     |
| 775                 | 0.30481  | 1.03313 | -0.311   | 0.09648  | 0     | 0     | 0     | 0     |
| 780                 | 0.33569  | 1.0155  | -0.3011  | 0.08904  | 0     | 0     | 0     | 0     |
| 785                 | 0.36209  | 0.9969  | -0.29309 | 0.08029  | 0     | 0     | 0     | 0     |
| 790                 | 0.38386  | 0.97771 | -0.28758 | 0.07006  | 0     | 0     | 0     | 0     |
| 795                 | 0.40088  | 0.95833 | -0.28517 | 0.05815  | 0     | 0     | 0     | 0     |
| 800                 | 0.41307  | 0.93883 | -0.28627 | 0.04427  | 0     | 0     | 0     | 0     |
| 805                 | 0.42048  | 0.91889 | -0.29099 | 0.02801  | 0     | 0     | 0     | 0     |
| 810                 | 0.42339  | 0.89844 | -0.29914 | 0.0094   | 0     | 0     | 0     | 0     |
| 815                 | 0.42217  | 0.87751 | -0.31045 | -0.01136 | 0     | 0     | 0     | 0     |
| 820                 | 0.4172   | 0.85614 | -0.32463 | -0.03409 | 0     | 0     | 0     | 0     |
| 825                 | 0.40886  | 0.83439 | -0.34137 | -0.05857 | 0     | 0     | 0     | 0     |
| 830                 | 0.39754  | 0.8123  | -0.36041 | -0.08462 | 0     | 0     | 0     | 0     |
| 835                 | 0.38361  | 0.7899  | -0.38143 | -0.11203 | 0     | 0     | 0     | 0     |
| 840                 | 0.36745  | 0.76725 | -0.40416 | -0.14061 | 0     | 0     | 0     | 0     |
| 845                 | 0.34944  | 0.74439 | -0.4283  | -0.17016 | 0     | 0     | 0     | 0     |
| 850                 | 0.32996  | 0.72136 | -0.45357 | -0.20047 | 0     | 0     | 0     | 0     |
| 855                 | 0.30939  | 0.6982  | -0.47967 | -0.23135 | 0     | 0     | 0     | 0     |
| 860                 | 0.2881   | 0.67496 | -0.50631 | -0.26261 | 0     | 0     | 0     | 0     |
| 865                 | 0.26649  | 0.65168 | -0.53321 | -0.29404 | 0     | 0     | 0     | 0     |

Table 31: Normalized Legendre coefficients in  $K^-p \rightarrow \Sigma^0\pi^0$  (2/2)

| Momentum<br>(MeV/c) | A1/A0    | A2/A0   | A3/A0    | A4/A0    | A5/A0    | A6/A0    | A7/A0 | A8/A0  |
|---------------------|----------|---------|----------|----------|----------|----------|-------|--------|
| 435                 | -0.41506 | 0.51794 | -0.39061 | -0.17259 | -0.00101 | -0.00057 | 0     | 1e-05  |
| 440                 | -0.41233 | 0.48944 | -0.38429 | -0.1651  | -0.00059 | -0.00043 | 0     | 1e-05  |
| 445                 | -0.4096  | 0.46112 | -0.37795 | -0.15764 | -0.00017 | -0.00029 | 0     | 0      |
| 450                 | -0.40685 | 0.4332  | -0.37154 | -0.15026 | 0.00025  | -0.00016 | 0     | 0      |
| 455                 | -0.40408 | 0.40591 | -0.36504 | -0.14301 | 0.00067  | -2e-05   | 0     | 0      |
| 460                 | -0.40131 | 0.37946 | -0.35841 | -0.13594 | 0.00109  | 0.00012  | 0     | 0      |
| 465                 | -0.39874 | 0.35403 | -0.35162 | -0.12907 | 0.00152  | 0.00025  | 0     | 0      |
| 470                 | -0.39658 | 0.32979 | -0.34467 | -0.12244 | 0.00194  | 0.00039  | 0     | 0      |
| 475                 | -0.39505 | 0.30691 | -0.33753 | -0.11608 | 0.00237  | 0.00053  | 0     | 0      |
| 480                 | -0.3944  | 0.28554 | -0.3302  | -0.11002 | 0.00279  | 0.00067  | 0     | -1e-05 |
| 485                 | -0.39493 | 0.26577 | -0.32275 | -0.10426 | 0.00322  | 0.00081  | 0     | -1e-05 |
| 490                 | -0.39696 | 0.24765 | -0.31529 | -0.09883 | 0.00364  | 0.00095  | 0     | -1e-05 |
| 495                 | -0.4008  | 0.23126 | -0.30789 | -0.09372 | 0.00407  | 0.00109  | 0     | -1e-05 |
| 500                 | -0.40672 | 0.21665 | -0.30065 | -0.08895 | 0.00449  | 0.00124  | 0     | -1e-05 |
| 505                 | -0.41477 | 0.20379 | -0.2936  | -0.08456 | 0.00491  | 0.00138  | 0     | -1e-05 |
| 510                 | -0.42493 | 0.19264 | -0.2868  | -0.0806  | 0.00533  | 0.00152  | 0     | -1e-05 |
| 515                 | -0.4372  | 0.18316 | -0.28027 | -0.07711 | 0.00575  | 0.00167  | 0     | -2e-05 |
| 520                 | -0.45145 | 0.17527 | -0.27403 | -0.07413 | 0.00616  | 0.00181  | 0     | -2e-05 |
| 525                 | -0.46723 | 0.16882 | -0.268   | -0.07163 | 0.00656  | 0.00195  | 0     | -2e-05 |
| 530                 | -0.48408 | 0.16365 | -0.26212 | -0.06961 | 0.00696  | 0.0021   | 0     | -2e-05 |
| 535                 | -0.50152 | 0.15962 | -0.25632 | -0.06805 | 0.00734  | 0.00224  | 0     | -2e-05 |
| 540                 | -0.5191  | 0.1566  | -0.25056 | -0.06694 | 0.00772  | 0.00238  | 0     | -2e-05 |
| 545                 | -0.53644 | 0.15456 | -0.24489 | -0.06628 | 0.00807  | 0.00251  | 0     | -3e-05 |
| 550                 | -0.55315 | 0.15349 | -0.23935 | -0.06605 | 0.00841  | 0.00264  | 0     | -3e-05 |
| 555                 | -0.56883 | 0.15338 | -0.23399 | -0.06626 | 0.00872  | 0.00277  | 0     | -3e-05 |
| 560                 | -0.58327 | 0.15419 | -0.22886 | -0.0669  | 0.00901  | 0.0029   | 0     | -3e-05 |
| 565                 | -0.59663 | 0.15588 | -0.2239  | -0.06794 | 0.00927  | 0.00301  | 0     | -3e-05 |
| 570                 | -0.60911 | 0.15838 | -0.21909 | -0.06938 | 0.00949  | 0.00312  | 0     | -3e-05 |
| 575                 | -0.62091 | 0.16164 | -0.21439 | -0.07118 | 0.00967  | 0.00322  | 0     | -4e-05 |
| 580                 | -0.63222 | 0.1656  | -0.20978 | -0.07333 | 0.00981  | 0.00331  | 0     | -4e-05 |
| 585                 | -0.64322 | 0.17023 | -0.20527 | -0.07583 | 0.0099   | 0.00339  | 0     | -4e-05 |
| 590                 | -0.65408 | 0.17551 | -0.20089 | -0.07867 | 0.00993  | 0.00345  | 0     | -4e-05 |
| 595                 | -0.66499 | 0.18138 | -0.19664 | -0.08184 | 0.0099   | 0.0035   | 0     | -4e-05 |
| 600                 | -0.6761  | 0.18784 | -0.19254 | -0.08532 | 0.0098   | 0.00353  | 0     | -4e-05 |
| 605                 | -0.68744 | 0.19486 | -0.18869 | -0.08913 | 0.00962  | 0.00354  | 0     | -4e-05 |
| 610                 | -0.69895 | 0.2025  | -0.18519 | -0.09324 | 0.00936  | 0.00353  | 0     | -4e-05 |
| 615                 | -0.71054 | 0.21077 | -0.18219 | -0.09768 | 0.009    | 0.00349  | 0     | -4e-05 |
| 620                 | -0.72215 | 0.21971 | -0.17979 | -0.10242 | 0.00855  | 0.00343  | 0     | -4e-05 |
| 625                 | -0.73381 | 0.22936 | -0.17813 | -0.1075  | 0.00798  | 0.00333  | 0     | -4e-05 |
| 630                 | -0.74564 | 0.23978 | -0.17729 | -0.11293 | 0.0073   | 0.00321  | 0     | -4e-05 |
| 635                 | -0.75775 | 0.25101 | -0.17738 | -0.11874 | 0.0065   | 0.00305  | 0     | -4e-05 |
| 640                 | -0.77025 | 0.26312 | -0.17851 | -0.12496 | 0.00555  | 0.00285  | 1e-05 | -4e-05 |
| 645                 | -0.78311 | 0.27609 | -0.18077 | -0.1316  | 0.00446  | 0.00261  | 1e-05 | -4e-05 |
| 650                 | -0.79619 | 0.28987 | -0.18424 | -0.13869 | 0.00322  | 0.00232  | 1e-05 | -3e-05 |
| 655                 | -0.80933 | 0.30439 | -0.18901 | -0.14623 | 0.00181  | 0.00199  | 1e-05 | -3e-05 |

Table 32: Normalized Legendre coefficients in  $K^-p \rightarrow \Sigma^+\pi^-$  (1/7)



| Momentum<br>(MeV/c) | A1/A0    | A2/A0   | A3/A0    | A4/A0    | A5/A0    | A6/A0    | A7/A0    | A8/A0   |
|---------------------|----------|---------|----------|----------|----------|----------|----------|---------|
| 660                 | -0.8224  | 0.3196  | -0.19518 | -0.15426 | 0.00022  | 0.0016   | 2e-05    | -3e-05  |
| 665                 | -0.83513 | 0.3354  | -0.2028  | -0.16277 | -0.00156 | 0.00116  | 2e-05    | -3e-05  |
| 670                 | -0.84713 | 0.35164 | -0.21197 | -0.1718  | -0.00353 | 0.00066  | 2e-05    | -2e-05  |
| 675                 | -0.85802 | 0.36815 | -0.22273 | -0.18137 | -0.00571 | 1e-04    | 3e-05    | -2e-05  |
| 680                 | -0.86734 | 0.38479 | -0.23516 | -0.19149 | -0.00811 | -0.00053 | 3e-05    | -1e-05  |
| 685                 | -0.87414 | 0.4013  | -0.24915 | -0.2022  | -0.01074 | -0.00123 | 4e-05    | 0       |
| 690                 | -0.87701 | 0.41738 | -0.26452 | -0.2135  | -0.0136  | -0.00201 | 4e-05    | 0       |
| 695                 | -0.87457 | 0.43271 | -0.28104 | -0.22543 | -0.01672 | -0.00286 | 4e-05    | 1e-05   |
| 700                 | -0.86542 | 0.447   | -0.29851 | -0.238   | -0.02008 | -0.00379 | 4e-05    | 2e-05   |
| 705                 | -0.8484  | 0.46    | -0.31674 | -0.25122 | -0.02371 | -0.00481 | 5e-05    | 3e-05   |
| 710                 | -0.82293 | 0.47163 | -0.33558 | -0.26507 | -0.02761 | -0.00591 | 5e-05    | 4e-05   |
| 715                 | -0.7885  | 0.48183 | -0.35485 | -0.2795  | -0.03179 | -0.00711 | 4e-05    | 5e-05   |
| 720                 | -0.74459 | 0.49053 | -0.37441 | -0.29449 | -0.03625 | -0.0084  | 4e-05    | 7e-05   |
| 725                 | -0.69112 | 0.49769 | -0.39405 | -0.31    | -0.041   | -0.00979 | 3e-05    | 8e-05   |
| 730                 | -0.62899 | 0.50329 | -0.41345 | -0.32601 | -0.04604 | -0.01127 | 2e-05    | 9e-05   |
| 735                 | -0.55919 | 0.50731 | -0.43227 | -0.34248 | -0.05136 | -0.01286 | 1e-05    | 0.00011 |
| 740                 | -0.48275 | 0.50974 | -0.45017 | -0.3594  | -0.05697 | -0.01455 | -1e-05   | 0.00013 |
| 745                 | -0.40083 | 0.51061 | -0.46688 | -0.37671 | -0.06287 | -0.01634 | -3e-05   | 0.00015 |
| 750                 | -0.31522 | 0.51019 | -0.48236 | -0.39436 | -0.06905 | -0.01823 | -6e-05   | 0.00017 |
| 755                 | -0.22787 | 0.50878 | -0.49662 | -0.41225 | -0.0755  | -0.02023 | -1e-04   | 0.00019 |
| 760                 | -0.14072 | 0.5067  | -0.5097  | -0.43031 | -0.08221 | -0.02233 | -0.00014 | 0.00021 |
| 765                 | -0.05569 | 0.50425 | -0.52159 | -0.44847 | -0.08917 | -0.02453 | -0.00019 | 0.00023 |
| 770                 | 0.0256   | 0.50172 | -0.53224 | -0.46666 | -0.09637 | -0.02683 | -0.00024 | 0.00026 |
| 775                 | 0.10169  | 0.49939 | -0.54158 | -0.48485 | -0.10377 | -0.02923 | -0.00031 | 0.00028 |
| 780                 | 0.17164  | 0.49748 | -0.54958 | -0.503   | -0.11136 | -0.03171 | -0.00038 | 0.00031 |
| 785                 | 0.23528  | 0.49609 | -0.55635 | -0.52109 | -0.11908 | -0.03426 | -0.00045 | 0.00034 |
| 790                 | 0.29246  | 0.49532 | -0.56201 | -0.53909 | -0.1269  | -0.03689 | -0.00053 | 0.00037 |
| 795                 | 0.34305  | 0.49529 | -0.56666 | -0.55697 | -0.13479 | -0.03958 | -0.00061 | 4e-04   |
| 800                 | 0.38717  | 0.49602 | -0.57044 | -0.5747  | -0.14269 | -0.04231 | -0.00069 | 0.00043 |
| 805                 | 0.42531  | 0.49745 | -0.57352 | -0.59223 | -0.15055 | -0.04508 | -0.00077 | 0.00046 |
| 810                 | 0.45797  | 0.49951 | -0.57609 | -0.60951 | -0.15829 | -0.04787 | -0.00084 | 0.00049 |
| 815                 | 0.48565  | 0.50213 | -0.57833 | -0.6265  | -0.16587 | -0.05066 | -0.00089 | 0.00052 |
| 820                 | 0.50886  | 0.50523 | -0.58041 | -0.64314 | -0.17322 | -0.05344 | -0.00093 | 0.00056 |
| 825                 | 0.5281   | 0.50875 | -0.58253 | -0.65939 | -0.18027 | -0.05618 | -0.00095 | 0.00059 |
| 830                 | 0.54388  | 0.51262 | -0.58485 | -0.6752  | -0.18697 | -0.05889 | -0.00095 | 0.00062 |
| 835                 | 0.55669  | 0.51675 | -0.58757 | -0.69052 | -0.19326 | -0.06154 | -0.00091 | 0.00065 |
| 840                 | 0.56705  | 0.5211  | -0.59085 | -0.70531 | -0.19907 | -0.06411 | -0.00084 | 0.00069 |
| 845                 | 0.57545  | 0.52557 | -0.59488 | -0.71951 | -0.20435 | -0.06659 | -0.00074 | 0.00072 |
| 850                 | 0.5824   | 0.53011 | -0.59985 | -0.73309 | -0.20902 | -0.06896 | -0.00059 | 0.00075 |
| 855                 | 0.5884   | 0.53464 | -0.60592 | -0.74598 | -0.21304 | -0.07122 | -4e-04   | 0.00078 |
| 860                 | 0.59395  | 0.53909 | -0.61329 | -0.75815 | -0.21633 | -0.07334 | -0.00016 | 0.00081 |
| 865                 | 0.59954  | 0.54338 | -0.62212 | -0.76955 | -0.21885 | -0.0753  | 0.00013  | 0.00084 |
| 870                 | 0.60541  | 0.54745 | -0.63256 | -0.78013 | -0.22056 | -0.0771  | 0.00048  | 0.00087 |
| 875                 | 0.61159  | 0.55119 | -0.64468 | -0.78984 | -0.22145 | -0.07869 | 0.00089  | 9e-04   |

Table 33: Normalized Legendre coefficients in  $K^-p \rightarrow \Sigma^+\pi^-$  (2/7)

| Momentum<br>(MeV/c) | A1/A0   | A2/A0   | A3/A0    | A4/A0    | A5/A0    | A6/A0    | A7/A0    | A8/A0    |
|---------------------|---------|---------|----------|----------|----------|----------|----------|----------|
| 880                 | 0.61811 | 0.55452 | -0.65859 | -0.79866 | -0.22151 | -0.08006 | 0.00137  | 0.00093  |
| 885                 | 0.62501 | 0.55734 | -0.67437 | -0.80652 | -0.22076 | -0.08119 | 0.00192  | 0.00095  |
| 890                 | 0.63226 | 0.55962 | -0.69201 | -0.81339 | -0.21917 | -0.08204 | 0.00254  | 0.00097  |
| 895                 | 0.63991 | 0.56144 | -0.71124 | -0.81921 | -0.21677 | -0.08265 | 0.00322  | 0.00099  |
| 900                 | 0.6482  | 0.56292 | -0.73165 | -0.82391 | -0.21351 | -0.08304 | 0.00396  | 0.00101  |
| 905                 | 0.65734 | 0.56418 | -0.7528  | -0.82746 | -0.20938 | -0.08324 | 0.00472  | 0.00102  |
| 910                 | 0.66707 | 0.56537 | -0.77433 | -0.82982 | -0.20437 | -0.08329 | 0.0055   | 0.00103  |
| 915                 | 0.67677 | 0.56667 | -0.79588 | -0.83094 | -0.19849 | -0.08322 | 0.00626  | 0.00103  |
| 920                 | 0.68581 | 0.56824 | -0.81712 | -0.83079 | -0.19176 | -0.08306 | 0.00696  | 0.00102  |
| 925                 | 0.6938  | 0.57027 | -0.83765 | -0.82936 | -0.18417 | -0.08286 | 0.00755  | 0.00101  |
| 930                 | 0.70068 | 0.57295 | -0.85705 | -0.8266  | -0.17573 | -0.08266 | 0.00799  | 0.00099  |
| 935                 | 0.70637 | 0.57649 | -0.8749  | -0.8225  | -0.16642 | -0.08249 | 0.00819  | 0.00097  |
| 940                 | 0.71082 | 0.58109 | -0.89077 | -0.81703 | -0.15624 | -0.08242 | 0.00809  | 0.00093  |
| 945                 | 0.71395 | 0.58698 | -0.90423 | -0.81016 | -0.14519 | -0.08246 | 0.0076   | 0.00088  |
| 950                 | 0.71565 | 0.59441 | -0.91489 | -0.80182 | -0.13326 | -0.08261 | 0.00663  | 0.00082  |
| 955                 | 0.71583 | 0.60361 | -0.92234 | -0.79199 | -0.12046 | -0.08291 | 0.00506  | 0.00075  |
| 960                 | 0.71439 | 0.61483 | -0.92615 | -0.78061 | -0.10679 | -0.08336 | 0.0028   | 0.00067  |
| 965                 | 0.71134 | 0.62829 | -0.92599 | -0.76765 | -0.09225 | -0.08398 | -0.00027 | 0.00056  |
| 970                 | 0.70709 | 0.64411 | -0.92166 | -0.7531  | -0.07689 | -0.08479 | -0.00425 | 0.00045  |
| 975                 | 0.7021  | 0.66238 | -0.91307 | -0.73694 | -0.06076 | -0.0858  | -0.00928 | 0.00031  |
| 980                 | 0.69672 | 0.68301 | -0.90027 | -0.7192  | -0.04391 | -0.08702 | -0.01547 | 0.00016  |
| 985                 | 0.69117 | 0.70589 | -0.8834  | -0.69991 | -0.02642 | -0.08844 | -0.02292 | -1e-05   |
| 990                 | 0.68572 | 0.73088 | -0.8626  | -0.6791  | -0.00834 | -0.09004 | -0.03174 | -0.00021 |
| 995                 | 0.6806  | 0.75785 | -0.838   | -0.6568  | 0.01026  | -0.09181 | -0.04202 | -0.00043 |
| 1000                | 0.67606 | 0.78666 | -0.80974 | -0.63304 | 0.02931  | -0.09375 | -0.05388 | -0.00067 |
| 1005                | 0.67236 | 0.81718 | -0.77798 | -0.60786 | 0.04877  | -0.09583 | -0.06739 | -0.00094 |
| 1010                | 0.66984 | 0.84916 | -0.74299 | -0.5813  | 0.06857  | -0.09799 | -0.08243 | -0.00124 |
| 1015                | 0.66874 | 0.88239 | -0.70509 | -0.5534  | 0.08867  | -0.10021 | -0.09858 | -0.00156 |
| 1020                | 0.66925 | 0.91668 | -0.66453 | -0.52422 | 0.10903  | -0.10243 | -0.11538 | -0.00191 |
| 1025                | 0.67157 | 0.95184 | -0.62161 | -0.49382 | 0.12959  | -0.10462 | -0.13236 | -0.00229 |
| 1030                | 0.67589 | 0.98766 | -0.57661 | -0.46226 | 0.15032  | -0.10673 | -0.14906 | -0.00271 |
| 1035                | 0.68241 | 1.02396 | -0.52979 | -0.42958 | 0.17118  | -0.10873 | -0.165   | -0.00316 |
| 1040                | 0.69132 | 1.06053 | -0.48143 | -0.39584 | 0.1921   | -0.11057 | -0.17973 | -0.00364 |
| 1045                | 0.70281 | 1.09718 | -0.43183 | -0.36109 | 0.21306  | -0.11223 | -0.19278 | -0.00415 |
| 1050                | 0.71699 | 1.13373 | -0.38124 | -0.3254  | 0.234    | -0.11366 | -0.2038  | -0.0047  |
| 1055                | 0.73356 | 1.17007 | -0.32997 | -0.28883 | 0.25489  | -0.11484 | -0.21289 | -0.00529 |
| 1060                | 0.75214 | 1.20612 | -0.2783  | -0.25144 | 0.27572  | -0.11578 | -0.22029 | -0.00591 |
| 1065                | 0.77234 | 1.24178 | -0.22653 | -0.2133  | 0.29644  | -0.11646 | -0.22622 | -0.00657 |
| 1070                | 0.79378 | 1.27697 | -0.17493 | -0.17448 | 0.31703  | -0.11688 | -0.23091 | -0.00727 |
| 1075                | 0.81607 | 1.31159 | -0.1238  | -0.13504 | 0.33746  | -0.11701 | -0.23458 | -0.008   |
| 1080                | 0.83883 | 1.34556 | -0.07343 | -0.09504 | 0.3577   | -0.11687 | -0.23746 | -0.00877 |
| 1085                | 0.86167 | 1.37879 | -0.02411 | -0.05456 | 0.37772  | -0.11643 | -0.23978 | -0.00959 |
| 1090                | 0.88422 | 1.41119 | 0.02389  | -0.01366 | 0.39751  | -0.11569 | -0.24169 | -0.01044 |
| 1095                | 0.90616 | 1.44276 | 0.07039  | 0.02762  | 0.41704  | -0.11467 | -0.24307 | -0.01132 |

Table 34: Normalized Legendre coefficients in  $K^-p \rightarrow \Sigma^+\pi^-$  (3/7)

| Momentum<br>(MeV/c) | A1/A0   | A2/A0   | A3/A0   | A4/A0   | A5/A0   | A6/A0    | A7/A0    | A8/A0    |
|---------------------|---------|---------|---------|---------|---------|----------|----------|----------|
| 1100                | 0.92718 | 1.47349 | 0.11521 | 0.06924 | 0.43632 | -0.11339 | -0.24371 | -0.01225 |
| 1105                | 0.94696 | 1.50338 | 0.15818 | 0.11115 | 0.45534 | -0.11187 | -0.24342 | -0.01321 |
| 1110                | 0.9652  | 1.53241 | 0.19913 | 0.15331 | 0.47409 | -0.11012 | -0.242   | -0.0142  |
| 1115                | 0.9816  | 1.5606  | 0.23789 | 0.19569 | 0.49258 | -0.10817 | -0.23926 | -0.01523 |
| 1120                | 0.99584 | 1.58794 | 0.27429 | 0.23824 | 0.51078 | -0.10603 | -0.23498 | -0.01629 |
| 1125                | 1.00761 | 1.61442 | 0.30816 | 0.28092 | 0.52871 | -0.10373 | -0.22898 | -0.01738 |
| 1130                | 1.01668 | 1.64004 | 0.33938 | 0.32369 | 0.54636 | -0.10127 | -0.22118 | -0.0185  |
| 1135                | 1.02313 | 1.66484 | 0.36806 | 0.36651 | 0.56375 | -0.09867 | -0.21198 | -0.01964 |
| 1140                | 1.02709 | 1.68883 | 0.39433 | 0.40934 | 0.58091 | -0.09593 | -0.20188 | -0.02081 |
| 1145                | 1.02872 | 1.71205 | 0.41837 | 0.45217 | 0.59787 | -0.09304 | -0.1914  | -0.02199 |
| 1150                | 1.02817 | 1.73453 | 0.4403  | 0.49494 | 0.61465 | -0.09001 | -0.18106 | -0.02319 |
| 1155                | 1.02559 | 1.75629 | 0.4603  | 0.53762 | 0.63128 | -0.08684 | -0.17138 | -0.0244  |
| 1160                | 1.02111 | 1.77737 | 0.47851 | 0.58018 | 0.64779 | -0.08352 | -0.16287 | -0.02561 |
| 1165                | 1.01489 | 1.7978  | 0.49508 | 0.62259 | 0.6642  | -0.08006 | -0.15604 | -0.02682 |
| 1170                | 1.00709 | 1.81759 | 0.51017 | 0.66481 | 0.68055 | -0.07647 | -0.15123 | -0.02803 |
| 1175                | 0.99786 | 1.83673 | 0.52401 | 0.70683 | 0.69689 | -0.07271 | -0.14805 | -0.02923 |
| 1180                | 0.98737 | 1.8552  | 0.53683 | 0.74862 | 0.71327 | -0.06878 | -0.14595 | -0.03041 |
| 1185                | 0.9758  | 1.87296 | 0.54887 | 0.79018 | 0.72977 | -0.06466 | -0.14436 | -0.03156 |
| 1190                | 0.96331 | 1.89    | 0.56034 | 0.8315  | 0.74642 | -0.06033 | -0.14272 | -0.03268 |
| 1195                | 0.95008 | 1.90628 | 0.57149 | 0.87255 | 0.7633  | -0.05577 | -0.14046 | -0.03375 |
| 1200                | 0.93626 | 1.92179 | 0.58256 | 0.91332 | 0.78046 | -0.05097 | -0.13703 | -0.03476 |
| 1205                | 0.92203 | 1.9365  | 0.59376 | 0.95379 | 0.79796 | -0.04591 | -0.13185 | -0.03572 |
| 1210                | 0.90757 | 1.95038 | 0.60531 | 0.99396 | 0.81585 | -0.04057 | -0.12448 | -0.0366  |
| 1215                | 0.89304 | 1.96341 | 0.61726 | 1.03379 | 0.83412 | -0.03495 | -0.1149  | -0.0374  |
| 1220                | 0.87864 | 1.97556 | 0.62967 | 1.07325 | 0.85278 | -0.02905 | -0.10319 | -0.0381  |
| 1225                | 0.86453 | 1.9868  | 0.64256 | 1.11232 | 0.87181 | -0.02286 | -0.08944 | -0.03869 |
| 1230                | 0.85091 | 1.9971  | 0.65596 | 1.15095 | 0.8912  | -0.01639 | -0.07374 | -0.03915 |
| 1235                | 0.83795 | 2.00644 | 0.66993 | 1.18913 | 0.91096 | -0.00962 | -0.05619 | -0.03947 |
| 1240                | 0.82582 | 2.01479 | 0.68448 | 1.22682 | 0.93106 | -0.00255 | -0.03687 | -0.03963 |
| 1245                | 0.81473 | 2.02212 | 0.69966 | 1.26398 | 0.9515  | 0.00481  | -0.01587 | -0.03962 |
| 1250                | 0.80486 | 2.0284  | 0.71551 | 1.3006  | 0.97227 | 0.01247  | 0.00658  | -0.03943 |
| 1255                | 0.7966  | 2.03353 | 0.73205 | 1.33662 | 0.99334 | 0.0204   | 0.02967  | -0.03908 |
| 1260                | 0.79032 | 2.03741 | 0.74932 | 1.372   | 1.0147  | 0.02857  | 0.05245  | -0.0386  |
| 1265                | 0.78642 | 2.03993 | 0.76735 | 1.40669 | 1.03632 | 0.03694  | 0.07397  | -0.038   |
| 1270                | 0.78492 | 2.04109 | 0.78615 | 1.44068 | 1.05815 | 0.04549  | 0.09368  | -0.03732 |
| 1275                | 0.78537 | 2.04098 | 0.80574 | 1.47397 | 1.08018 | 0.05421  | 0.11146  | -0.03658 |
| 1280                | 0.78729 | 2.03971 | 0.8261  | 1.50657 | 1.10237 | 0.0631   | 0.12727  | -0.0358  |
| 1285                | 0.79021 | 2.03737 | 0.84724 | 1.53849 | 1.12468 | 0.07215  | 0.14103  | -0.035   |
| 1290                | 0.79375 | 2.03407 | 0.86916 | 1.56972 | 1.14706 | 0.08134  | 0.15264  | -0.03421 |
| 1295                | 0.79786 | 2.02989 | 0.89186 | 1.60028 | 1.16947 | 0.09069  | 0.16178  | -0.03347 |
| 1300                | 0.80263 | 2.02488 | 0.91536 | 1.63014 | 1.19182 | 0.10018  | 0.16808  | -0.03285 |
| 1305                | 0.80811 | 2.01914 | 0.93965 | 1.65929 | 1.21405 | 0.10981  | 0.17119  | -0.03239 |
| 1310                | 0.81435 | 2.01272 | 0.96476 | 1.68774 | 1.23609 | 0.11959  | 0.17074  | -0.03214 |
| 1315                | 0.82144 | 2.0057  | 0.99069 | 1.71547 | 1.25787 | 0.12949  | 0.16635  | -0.03216 |

Table 35: Normalized Legendre coefficients in  $K^-p \rightarrow \Sigma^+\pi^-$  (4/7)

| Momentum<br>(MeV/c) | A1/A0   | A2/A0   | A3/A0   | A4/A0   | A5/A0   | A6/A0   | A7/A0    | A8/A0    |
|---------------------|---------|---------|---------|---------|---------|---------|----------|----------|
| 1320                | 0.82936 | 1.99815 | 1.01744 | 1.74248 | 1.27932 | 0.13954 | 0.15783  | -0.03249 |
| 1325                | 0.83779 | 1.99015 | 1.04496 | 1.76877 | 1.30041 | 0.14973 | 0.14596  | -0.03314 |
| 1330                | 0.84665 | 1.9818  | 1.07325 | 1.79437 | 1.32111 | 0.1601  | 0.13175  | -0.03405 |
| 1335                | 0.85598 | 1.97322 | 1.10228 | 1.81929 | 1.3414  | 0.17067 | 0.11614  | -0.03517 |
| 1340                | 0.86584 | 1.96452 | 1.13207 | 1.84353 | 1.36125 | 0.18147 | 0.10006  | -0.03645 |
| 1345                | 0.87626 | 1.9558  | 1.16259 | 1.86713 | 1.38065 | 0.19253 | 0.08445  | -0.03781 |
| 1350                | 0.88729 | 1.94717 | 1.19385 | 1.89008 | 1.39956 | 0.20387 | 0.07024  | -0.0392  |
| 1355                | 0.89897 | 1.93876 | 1.22584 | 1.9124  | 1.41797 | 0.21552 | 0.05839  | -0.04056 |
| 1360                | 0.91133 | 1.93063 | 1.25852 | 1.9341  | 1.43584 | 0.22751 | 0.04964  | -0.04184 |
| 1365                | 0.92428 | 1.92278 | 1.29175 | 1.95515 | 1.45313 | 0.23983 | 0.04407  | -0.043   |
| 1370                | 0.93773 | 1.91515 | 1.32538 | 1.97551 | 1.46982 | 0.25248 | 0.04159  | -0.04401 |
| 1375                | 0.95159 | 1.90768 | 1.35924 | 1.99516 | 1.48588 | 0.26547 | 0.0418   | -0.04485 |
| 1380                | 0.96583 | 1.90033 | 1.39318 | 2.01405 | 1.50132 | 0.27876 | 0.04395  | -0.04548 |
| 1385                | 0.98042 | 1.89304 | 1.42703 | 2.03215 | 1.51615 | 0.29237 | 0.04726  | -0.0459  |
| 1390                | 0.9953  | 1.88573 | 1.46066 | 2.04944 | 1.53039 | 0.30627 | 0.05095  | -0.04606 |
| 1395                | 1.01046 | 1.87835 | 1.49391 | 2.06587 | 1.54404 | 0.32046 | 0.05424  | -0.04595 |
| 1400                | 1.02585 | 1.87084 | 1.52662 | 2.08142 | 1.55712 | 0.33492 | 0.05634  | -0.04555 |
| 1405                | 1.04143 | 1.86314 | 1.55865 | 2.09605 | 1.56963 | 0.34966 | 0.05648  | -0.04482 |
| 1410                | 1.05718 | 1.8552  | 1.58983 | 2.10973 | 1.58159 | 0.36465 | 0.05388  | -0.04374 |
| 1415                | 1.07304 | 1.84694 | 1.62001 | 2.12243 | 1.59301 | 0.37988 | 0.04775  | -0.04229 |
| 1420                | 1.08898 | 1.83832 | 1.64908 | 2.13412 | 1.6039  | 0.39535 | 0.03758  | -0.04044 |
| 1425                | 1.10484 | 1.82934 | 1.67699 | 2.14484 | 1.6143  | 0.41106 | 0.02383  | -0.03819 |
| 1430                | 1.12048 | 1.81999 | 1.70374 | 2.15463 | 1.62425 | 0.427   | 0.00724  | -0.03552 |
| 1435                | 1.13574 | 1.81027 | 1.72932 | 2.16352 | 1.63379 | 0.44316 | -0.01145 | -0.03242 |
| 1440                | 1.15046 | 1.80018 | 1.75373 | 2.17157 | 1.64296 | 0.45955 | -0.03152 | -0.02889 |
| 1445                | 1.16449 | 1.78973 | 1.77696 | 2.17881 | 1.65179 | 0.47617 | -0.05224 | -0.0249  |
| 1450                | 1.17767 | 1.77892 | 1.799   | 2.18528 | 1.66033 | 0.493   | -0.07288 | -0.02046 |
| 1455                | 1.18985 | 1.76774 | 1.81985 | 2.19103 | 1.66861 | 0.51005 | -0.09269 | -0.01555 |
| 1460                | 1.20086 | 1.75621 | 1.8395  | 2.1961  | 1.67668 | 0.52732 | -0.11096 | -0.01015 |
| 1465                | 1.21057 | 1.74432 | 1.85795 | 2.20053 | 1.68457 | 0.54479 | -0.12698 | -0.00427 |
| 1470                | 1.219   | 1.7322  | 1.87524 | 2.20436 | 1.69232 | 0.56245 | -0.14044 | 0.00207  |
| 1475                | 1.22629 | 1.72006 | 1.89148 | 2.20761 | 1.69992 | 0.58024 | -0.15137 | 0.00883  |
| 1480                | 1.2326  | 1.7081  | 1.90674 | 2.21031 | 1.70741 | 0.59813 | -0.15979 | 0.01594  |
| 1485                | 1.23807 | 1.69653 | 1.92113 | 2.2125  | 1.71479 | 0.61607 | -0.16572 | 0.02336  |
| 1490                | 1.24286 | 1.68556 | 1.93474 | 2.21421 | 1.72208 | 0.63402 | -0.16918 | 0.03103  |
| 1495                | 1.24712 | 1.67541 | 1.94765 | 2.21547 | 1.7293  | 0.65192 | -0.17019 | 0.03891  |
| 1500                | 1.251   | 1.66628 | 1.95997 | 2.21629 | 1.73646 | 0.66975 | -0.16879 | 0.04693  |
| 1505                | 1.25464 | 1.65837 | 1.97178 | 2.21673 | 1.74357 | 0.68744 | -0.16499 | 0.05505  |
| 1510                | 1.25822 | 1.65191 | 1.98318 | 2.2168  | 1.75066 | 0.70496 | -0.15881 | 0.06321  |
| 1515                | 1.26186 | 1.64709 | 1.99426 | 2.21654 | 1.75773 | 0.72227 | -0.15028 | 0.07137  |
| 1520                | 1.26574 | 1.64404 | 2.00509 | 2.21596 | 1.7648  | 0.73931 | -0.13954 | 0.07946  |
| 1525                | 1.27001 | 1.6427  | 2.01568 | 2.21509 | 1.77186 | 0.75605 | -0.12701 | 0.08744  |
| 1530                | 1.27484 | 1.64297 | 2.02605 | 2.21392 | 1.77888 | 0.77244 | -0.11314 | 0.09525  |
| 1535                | 1.28041 | 1.64477 | 2.03621 | 2.21246 | 1.78586 | 0.78844 | -0.09836 | 0.10284  |

Table 36: Normalized Legendre coefficients in  $K^-p \rightarrow \Sigma^+\pi^-$  (5/7)

| Momentum<br>(MeV/c) | A1/A0   | A2/A0   | A3/A0   | A4/A0   | A5/A0   | A6/A0   | A7/A0    | A8/A0   |
|---------------------|---------|---------|---------|---------|---------|---------|----------|---------|
| 1540                | 1.28686 | 1.64799 | 2.04616 | 2.21072 | 1.79279 | 0.80401 | -0.08314 | 0.11014 |
| 1545                | 1.29439 | 1.65256 | 2.05591 | 2.2087  | 1.79966 | 0.8191  | -0.06791 | 0.11712 |
| 1550                | 1.3031  | 1.65836 | 2.06547 | 2.20642 | 1.80644 | 0.83367 | -0.05309 | 0.12371 |
| 1555                | 1.3129  | 1.66525 | 2.07475 | 2.20382 | 1.81312 | 0.84769 | -0.03882 | 0.1299  |
| 1560                | 1.32356 | 1.67306 | 2.08365 | 2.20085 | 1.81969 | 0.86115 | -0.02508 | 0.1357  |
| 1565                | 1.33485 | 1.68162 | 2.09205 | 2.19746 | 1.82612 | 0.87402 | -0.0119  | 0.14112 |
| 1570                | 1.34654 | 1.69074 | 2.09985 | 2.19357 | 1.83239 | 0.88627 | 0.00073  | 0.14615 |
| 1575                | 1.35842 | 1.70026 | 2.10691 | 2.18914 | 1.83849 | 0.89789 | 0.01281  | 0.1508  |
| 1580                | 1.37025 | 1.71001 | 2.11314 | 2.1841  | 1.8444  | 0.90885 | 0.02433  | 0.15507 |
| 1585                | 1.38181 | 1.71981 | 2.11843 | 2.17841 | 1.8501  | 0.91914 | 0.03529  | 0.15897 |
| 1590                | 1.39288 | 1.72949 | 2.12265 | 2.17199 | 1.85557 | 0.92872 | 0.04568  | 0.1625  |
| 1595                | 1.40323 | 1.73887 | 2.1257  | 2.16479 | 1.86078 | 0.93759 | 0.0555   | 0.16566 |
| 1600                | 1.41263 | 1.74778 | 2.12746 | 2.15675 | 1.86573 | 0.9457  | 0.06474  | 0.16846 |
| 1605                | 1.42086 | 1.75605 | 2.12782 | 2.14782 | 1.8704  | 0.95306 | 0.07341  | 0.1709  |
| 1610                | 1.42772 | 1.76352 | 2.12669 | 2.13793 | 1.87475 | 0.95962 | 0.08151  | 0.17299 |
| 1615                | 1.43328 | 1.77017 | 2.12406 | 2.12708 | 1.87879 | 0.96539 | 0.08916  | 0.17472 |
| 1620                | 1.43768 | 1.77599 | 2.11996 | 2.11527 | 1.88249 | 0.97035 | 0.09653  | 0.17611 |
| 1625                | 1.4411  | 1.78103 | 2.11445 | 2.10249 | 1.88584 | 0.97449 | 0.10377  | 0.17715 |
| 1630                | 1.44369 | 1.7853  | 2.10756 | 2.08876 | 1.88883 | 0.97781 | 0.11105  | 0.17786 |
| 1635                | 1.44561 | 1.78882 | 2.09933 | 2.07406 | 1.89145 | 0.98031 | 0.11854  | 0.17823 |
| 1640                | 1.44703 | 1.79161 | 2.0898  | 2.05839 | 1.89369 | 0.98196 | 0.1264   | 0.17827 |
| 1645                | 1.4481  | 1.7937  | 2.07902 | 2.04178 | 1.89552 | 0.98277 | 0.1348   | 0.17798 |
| 1650                | 1.449   | 1.79509 | 2.06703 | 2.0242  | 1.89693 | 0.98272 | 0.14389  | 0.17737 |
| 1655                | 1.44987 | 1.79582 | 2.05386 | 2.00566 | 1.89793 | 0.98181 | 0.15384  | 0.17644 |
| 1660                | 1.4508  | 1.79591 | 2.03956 | 1.98617 | 1.89846 | 0.98003 | 0.16463  | 0.17518 |
| 1665                | 1.45177 | 1.79536 | 2.02422 | 1.96574 | 1.89851 | 0.97737 | 0.17604  | 0.17354 |
| 1670                | 1.45273 | 1.79421 | 2.0079  | 1.94436 | 1.89801 | 0.9738  | 0.18781  | 0.1715  |
| 1675                | 1.45366 | 1.79245 | 1.99068 | 1.92205 | 1.89694 | 0.96931 | 0.1997   | 0.16901 |
| 1680                | 1.45453 | 1.79012 | 1.97262 | 1.89882 | 1.89525 | 0.9639  | 0.21145  | 0.16602 |
| 1685                | 1.4553  | 1.78723 | 1.95379 | 1.87466 | 1.8929  | 0.95754 | 0.22282  | 0.16251 |
| 1690                | 1.45594 | 1.78379 | 1.93428 | 1.84959 | 1.88984 | 0.95022 | 0.23355  | 0.15843 |
| 1695                | 1.45642 | 1.77982 | 1.91414 | 1.82361 | 1.88604 | 0.94193 | 0.24341  | 0.15375 |
| 1700                | 1.4567  | 1.77534 | 1.89345 | 1.79673 | 1.88144 | 0.93265 | 0.25213  | 0.14842 |
| 1705                | 1.45676 | 1.77036 | 1.87229 | 1.76895 | 1.87602 | 0.92237 | 0.25948  | 0.1424  |
| 1710                | 1.45653 | 1.76489 | 1.85069 | 1.74029 | 1.86972 | 0.91108 | 0.26518  | 0.13566 |
| 1715                | 1.45585 | 1.75888 | 1.8286  | 1.71072 | 1.86253 | 0.89877 | 0.26888  | 0.12821 |
| 1720                | 1.45454 | 1.75226 | 1.80593 | 1.68023 | 1.85444 | 0.88545 | 0.27022  | 0.12005 |
| 1725                | 1.45241 | 1.74498 | 1.78259 | 1.6488  | 1.84541 | 0.87112 | 0.26884  | 0.11119 |
| 1730                | 1.44926 | 1.73696 | 1.75849 | 1.61643 | 1.83543 | 0.8558  | 0.26436  | 0.10163 |
| 1735                | 1.44492 | 1.72815 | 1.73354 | 1.58309 | 1.82449 | 0.83947 | 0.25641  | 0.0914  |
| 1740                | 1.43919 | 1.71847 | 1.70766 | 1.54877 | 1.81256 | 0.82215 | 0.24464  | 0.08048 |
| 1745                | 1.43192 | 1.70788 | 1.68076 | 1.51346 | 1.79963 | 0.80384 | 0.22872  | 0.06891 |
| 1750                | 1.42321 | 1.69643 | 1.6529  | 1.4772  | 1.78573 | 0.78458 | 0.20876  | 0.05669 |
| 1755                | 1.41325 | 1.68419 | 1.62417 | 1.44003 | 1.77092 | 0.76442 | 0.18503  | 0.04387 |

Table 37: Normalized Legendre coefficients in  $K^-p \rightarrow \Sigma^+\pi^-$  (6/7)

| Momentum<br>(MeV/c) | A1/A0   | A2/A0   | A3/A0   | A4/A0   | A5/A0   | A6/A0   | A7/A0    | A8/A0    |
|---------------------|---------|---------|---------|---------|---------|---------|----------|----------|
| 1760                | 1.40226 | 1.67124 | 1.59466 | 1.40201 | 1.75523 | 0.74341 | 0.15781  | 0.03049  |
| 1765                | 1.39045 | 1.65768 | 1.56447 | 1.3632  | 1.73872 | 0.72159 | 0.12737  | 0.01657  |
| 1770                | 1.37802 | 1.64358 | 1.53368 | 1.32364 | 1.72144 | 0.69903 | 0.094    | 0.00214  |
| 1775                | 1.36518 | 1.62903 | 1.5024  | 1.28339 | 1.70344 | 0.67576 | 0.05798  | -0.01274 |
| 1780                | 1.35214 | 1.61411 | 1.47071 | 1.24251 | 1.68477 | 0.65185 | 0.01957  | -0.02806 |
| 1785                | 1.3391  | 1.59891 | 1.43872 | 1.20104 | 1.66547 | 0.62732 | -0.02093 | -0.04378 |
| 1790                | 1.32627 | 1.58351 | 1.4065  | 1.15905 | 1.6456  | 0.60225 | -0.06326 | -0.05985 |
| 1795                | 1.31385 | 1.56799 | 1.37416 | 1.11658 | 1.6252  | 0.57668 | -0.10713 | -0.07626 |
| 1800                | 1.30206 | 1.55243 | 1.3418  | 1.07368 | 1.60433 | 0.55065 | -0.15227 | -0.09296 |
| 1805                | 1.29111 | 1.53692 | 1.3095  | 1.03042 | 1.58303 | 0.52422 | -0.1984  | -0.10991 |
| 1810                | 1.28119 | 1.52155 | 1.27735 | 0.98684 | 1.56136 | 0.49744 | -0.24524 | -0.12709 |
| 1815                | 1.27252 | 1.50639 | 1.24546 | 0.943   | 1.53936 | 0.47035 | -0.29251 | -0.14447 |
| 1820                | 1.2653  | 1.49154 | 1.21391 | 0.89895 | 1.51708 | 0.44301 | -0.33993 | -0.16199 |
| 1825                | 1.25974 | 1.47706 | 1.18281 | 0.85475 | 1.49457 | 0.41547 | -0.38723 | -0.17964 |
| 1830                | 1.25605 | 1.46305 | 1.15224 | 0.81044 | 1.47189 | 0.38777 | -0.43413 | -0.19737 |
| 1835                | 1.25443 | 1.4496  | 1.12229 | 0.76609 | 1.44907 | 0.35997 | -0.48035 | -0.21516 |
| 1840                | 1.25509 | 1.43678 | 1.09306 | 0.72174 | 1.42618 | 0.33212 | -0.5256  | -0.23297 |
| 1845                | 1.25803 | 1.42461 | 1.06458 | 0.67744 | 1.40325 | 0.30425 | -0.56974 | -0.25076 |

Table 38: Normalized Legendre coefficients in  $K^-p \rightarrow \Sigma^+\pi^-$  (7/7)

| Momentum<br>(MeV/c) | A1/A0   | A2/A0    | A3/A0    | A4/A0    | A5/A0 | A6/A0 | A7/A0 |
|---------------------|---------|----------|----------|----------|-------|-------|-------|
| 930                 | 0.18739 | -0.06    | -0.00621 | -2e-05   | 0     | 0     | 0     |
| 935                 | 0.22915 | -0.05104 | -0.00013 | -2e-05   | 0     | 0     | 0     |
| 940                 | 0.27087 | -0.04199 | 0.006    | -2e-05   | 0     | 0     | 0     |
| 945                 | 0.31247 | -0.0327  | 0.01223  | -2e-05   | 0     | 0     | 0     |
| 950                 | 0.35388 | -0.02306 | 0.01863  | -2e-05   | 0     | 0     | 0     |
| 955                 | 0.39503 | -0.01292 | 0.02525  | -2e-05   | 0     | 0     | 0     |
| 960                 | 0.43586 | -0.00217 | 0.03214  | -3e-05   | 0     | 0     | 0     |
| 965                 | 0.4763  | 0.00933  | 0.03938  | -3e-05   | 0     | 0     | 0     |
| 970                 | 0.51629 | 0.02171  | 0.04702  | -3e-05   | 0     | 0     | 0     |
| 975                 | 0.55575 | 0.03509  | 0.05511  | -3e-05   | 0     | 0     | 0     |
| 980                 | 0.59462 | 0.04962  | 0.06371  | -3e-05   | 0     | 0     | 0     |
| 985                 | 0.63291 | 0.06537  | 0.073    | -3e-05   | 0     | 0     | 0     |
| 990                 | 0.6706  | 0.08222  | 0.0833   | -3e-05   | 0     | 0     | 0     |
| 995                 | 0.70756 | 0.09998  | 0.09494  | -2e-05   | 0     | 0     | 0     |
| 1000                | 0.74362 | 0.11842  | 0.10816  | -2e-05   | 0     | 0     | 0     |
| 1005                | 0.77857 | 0.13733  | 0.12261  | -2e-05   | 0     | 0     | 0     |
| 1010                | 0.8121  | 0.15648  | 0.13737  | -1e-05   | 0     | 0     | 0     |
| 1015                | 0.84402 | 0.17556  | 0.15102  | -1e-05   | 0     | 0     | 0     |
| 1020                | 0.87447 | 0.19424  | 0.16201  | 0        | 0     | 0     | 0     |
| 1025                | 0.90358 | 0.21231  | 0.16943  | 1e-05    | 0     | 0     | 0     |
| 1030                | 0.93118 | 0.22961  | 0.17264  | 2e-05    | 0     | 0     | 0     |
| 1035                | 0.95642 | 0.24598  | 0.17205  | 4e-05    | 0     | 0     | 0     |
| 1040                | 0.9784  | 0.26128  | 0.16958  | 6e-05    | 0     | 0     | 0     |
| 1045                | 0.99681 | 0.2754   | 0.16737  | 8e-05    | 0     | 0     | 0     |
| 1050                | 1.01213 | 0.2883   | 0.16575  | 1e-04    | 0     | 0     | 0     |
| 1055                | 1.02473 | 0.29992  | 0.16397  | 0.00012  | 0     | 0     | 0     |
| 1060                | 1.03467 | 0.31018  | 0.16082  | 0.00015  | 0     | 0     | 0     |
| 1065                | 1.0417  | 0.31907  | 0.15599  | 0.00018  | 0     | 0     | 0     |
| 1070                | 1.04567 | 0.32661  | 0.14947  | 0.00021  | 0     | 0     | 0     |
| 1075                | 1.04705 | 0.3329   | 0.14185  | 0.00024  | 0     | 0     | 0     |
| 1080                | 1.04645 | 0.33806  | 0.13383  | 0.00027  | 0     | 0     | 0     |
| 1085                | 1.04451 | 0.34222  | 0.12613  | 3e-04    | 0     | 0     | 0     |
| 1090                | 1.04182 | 0.34551  | 0.11946  | 0.00032  | 0     | 0     | 0     |
| 1095                | 1.03903 | 0.34804  | 0.11454  | 0.00034  | 0     | 0     | 0     |
| 1100                | 1.03662 | 0.34992  | 0.11184  | 0.00036  | 0     | 0     | 0     |
| 1105                | 1.03464 | 0.35117  | 0.11087  | 0.00037  | 0     | 0     | 0     |
| 1110                | 1.03303 | 0.3518   | 0.11087  | 0.00037  | 0     | 0     | 0     |
| 1115                | 1.0317  | 0.35178  | 0.1111   | 0.00037  | 0     | 0     | 0     |
| 1120                | 1.03059 | 0.35112  | 0.11082  | 0.00035  | 0     | 0     | 0     |
| 1125                | 1.02963 | 0.34981  | 0.10927  | 0.00031  | 0     | 0     | 0     |
| 1130                | 1.02873 | 0.34786  | 0.10573  | 0.00027  | 0     | 0     | 0     |
| 1135                | 1.02779 | 0.34528  | 0.09967  | 2e-04    | 0     | 0     | 0     |
| 1140                | 1.02643 | 0.34217  | 0.09158  | 0.00012  | 0     | 0     | 0     |
| 1145                | 1.02426 | 0.33869  | 0.08216  | 2e-05    | 0     | 0     | 0     |
| 1150                | 1.02085 | 0.33495  | 0.07213  | -0.00011 | 0     | 0     | 0     |
| 1155                | 1.01581 | 0.33109  | 0.0622   | -0.00026 | 0     | 0     | 0     |

Table 39: Normalized Legendre coefficients in  $\pi N \rightarrow \Lambda K$  (1/7)

| Momentum<br>(MeV/c) | A1/A0   | A2/A0   | A3/A0    | A4/A0    | A5/A0  | A6/A0  | A7/A0  |
|---------------------|---------|---------|----------|----------|--------|--------|--------|
| 1160                | 1.00873 | 0.32726 | 0.05308  | -0.00044 | 0      | 0      | 0      |
| 1165                | 0.99942 | 0.32354 | 0.04523  | -0.00065 | 0      | 0      | 0      |
| 1170                | 0.98823 | 0.31998 | 0.03857  | -9e-04   | 0      | 0      | 0      |
| 1175                | 0.97557 | 0.31661 | 0.03292  | -0.00117 | 0      | 0      | 0      |
| 1180                | 0.96183 | 0.31345 | 0.02813  | -0.00148 | 0      | 0      | 0      |
| 1185                | 0.94743 | 0.31053 | 0.02403  | -0.00183 | 0      | 0      | 0      |
| 1190                | 0.93279 | 0.30788 | 0.02045  | -0.00221 | 1e-05  | -1e-05 | 0      |
| 1195                | 0.91829 | 0.30552 | 0.01722  | -0.00263 | 1e-05  | -1e-05 | 0      |
| 1200                | 0.90437 | 0.30349 | 0.0142   | -0.00309 | 1e-05  | -1e-05 | 0      |
| 1205                | 0.89141 | 0.30181 | 0.0112   | -0.0036  | 1e-05  | -1e-05 | 0      |
| 1210                | 0.87983 | 0.30052 | 0.00806  | -0.00414 | 1e-05  | -1e-05 | 0      |
| 1215                | 0.87005 | 0.29962 | 0.00463  | -0.00473 | 1e-05  | -1e-05 | 0      |
| 1220                | 0.86245 | 0.29917 | 0.00072  | -0.00537 | 1e-05  | -1e-05 | 0      |
| 1225                | 0.85746 | 0.29917 | -0.00381 | -0.00605 | 1e-05  | -1e-05 | 0      |
| 1230                | 0.85526 | 0.29965 | -0.00909 | -0.00678 | 1e-05  | -1e-05 | 0      |
| 1235                | 0.85551 | 0.30056 | -0.01516 | -0.00754 | 1e-05  | -2e-05 | 0      |
| 1240                | 0.85783 | 0.30188 | -0.02202 | -0.00833 | 1e-05  | -2e-05 | 0      |
| 1245                | 0.86183 | 0.30357 | -0.02969 | -0.00912 | 0      | -2e-05 | 0      |
| 1250                | 0.86711 | 0.30559 | -0.03818 | -0.00992 | 0      | -2e-05 | 0      |
| 1255                | 0.87328 | 0.30789 | -0.0475  | -0.0107  | 0      | -2e-05 | 0      |
| 1260                | 0.87995 | 0.31046 | -0.05768 | -0.01146 | 0      | -2e-05 | 0      |
| 1265                | 0.88672 | 0.31324 | -0.06872 | -0.01218 | 0      | -2e-05 | 0      |
| 1270                | 0.89321 | 0.3162  | -0.08064 | -0.01285 | 0      | -2e-05 | 0      |
| 1275                | 0.89901 | 0.31931 | -0.09346 | -0.01347 | 0      | -2e-05 | 0      |
| 1280                | 0.90375 | 0.32252 | -0.10718 | -0.01401 | 0      | -2e-05 | 0      |
| 1285                | 0.90702 | 0.3258  | -0.12182 | -0.01447 | -1e-05 | -2e-05 | 0      |
| 1290                | 0.90844 | 0.32912 | -0.13739 | -0.01483 | -1e-05 | -2e-05 | -1e-05 |
| 1295                | 0.90798 | 0.33251 | -0.15381 | -0.01508 | -1e-05 | -2e-05 | -1e-05 |
| 1300                | 0.90606 | 0.33607 | -0.17084 | -0.01516 | -2e-05 | -2e-05 | -1e-05 |
| 1305                | 0.90314 | 0.33995 | -0.18827 | -0.01504 | -2e-05 | -2e-05 | -1e-05 |
| 1310                | 0.89965 | 0.34425 | -0.20584 | -0.01466 | -2e-05 | -2e-05 | -1e-05 |
| 1315                | 0.89606 | 0.34911 | -0.22335 | -0.01398 | -3e-05 | -1e-05 | -1e-05 |
| 1320                | 0.89281 | 0.35464 | -0.24054 | -0.01297 | -3e-05 | -1e-05 | -2e-05 |
| 1325                | 0.89036 | 0.36097 | -0.2572  | -0.01157 | -4e-05 | -1e-05 | -2e-05 |
| 1330                | 0.88915 | 0.36823 | -0.27308 | -0.00975 | -5e-05 | 0      | -2e-05 |
| 1335                | 0.88959 | 0.37652 | -0.28798 | -0.00745 | -5e-05 | 0      | -2e-05 |
| 1340                | 0.89162 | 0.38589 | -0.30176 | -0.00461 | -6e-05 | 1e-05  | -3e-05 |
| 1345                | 0.89499 | 0.39635 | -0.31438 | -0.00118 | -6e-05 | 2e-05  | -3e-05 |
| 1350                | 0.89948 | 0.40792 | -0.32575 | 0.00291  | -7e-05 | 3e-05  | -3e-05 |
| 1355                | 0.90484 | 0.42061 | -0.3358  | 0.00773  | -8e-05 | 4e-05  | -4e-05 |
| 1360                | 0.91082 | 0.43443 | -0.34446 | 0.01335  | -8e-05 | 5e-05  | -4e-05 |
| 1365                | 0.91718 | 0.44939 | -0.35167 | 0.01983  | -9e-05 | 7e-05  | -4e-05 |
| 1370                | 0.92368 | 0.46552 | -0.35736 | 0.02723  | -1e-04 | 8e-05  | -4e-05 |
| 1375                | 0.93008 | 0.48281 | -0.36144 | 0.03562  | -1e-04 | 1e-04  | -5e-05 |

Table 40: Normalized Legendre coefficients in  $\pi N \rightarrow \Lambda K$  (2/7)



| Momentum<br>(MeV/c) | A1/A0   | A2/A0   | A3/A0    | A4/A0   | A5/A0    | A6/A0    | A7/A0   |
|---------------------|---------|---------|----------|---------|----------|----------|---------|
| 1380                | 0.93614 | 0.50128 | -0.36387 | 0.04506 | -0.00011 | 0.00012  | -5e-05  |
| 1385                | 0.94161 | 0.52096 | -0.36455 | 0.05562 | -0.00011 | 0.00014  | -5e-05  |
| 1390                | 0.94624 | 0.54184 | -0.36343 | 0.06737 | -0.00012 | 0.00016  | -5e-05  |
| 1395                | 0.94981 | 0.56394 | -0.36043 | 0.08036 | -0.00012 | 0.00018  | -5e-05  |
| 1400                | 0.95212 | 0.58725 | -0.35554 | 0.09464 | -0.00012 | 0.00021  | -5e-05  |
| 1405                | 0.95323 | 0.61167 | -0.34898 | 0.11013 | -0.00012 | 0.00023  | -5e-05  |
| 1410                | 0.95325 | 0.63706 | -0.34102 | 0.12669 | -0.00012 | 0.00026  | -5e-05  |
| 1415                | 0.95229 | 0.6633  | -0.33195 | 0.14424 | -0.00012 | 0.00029  | -5e-05  |
| 1420                | 0.95046 | 0.69026 | -0.32204 | 0.16264 | -0.00011 | 0.00032  | -4e-05  |
| 1425                | 0.94788 | 0.7178  | -0.31156 | 0.1818  | -1e-04   | 0.00035  | -4e-05  |
| 1430                | 0.94466 | 0.74581 | -0.30079 | 0.20158 | -9e-05   | 0.00038  | -3e-05  |
| 1435                | 0.9409  | 0.77415 | -0.29002 | 0.22189 | -8e-05   | 0.00041  | -3e-05  |
| 1440                | 0.93673 | 0.80269 | -0.2795  | 0.24261 | -6e-05   | 0.00044  | -2e-05  |
| 1445                | 0.93225 | 0.8313  | -0.26953 | 0.26362 | -4e-05   | 0.00047  | -1e-05  |
| 1450                | 0.92757 | 0.85985 | -0.26038 | 0.28481 | -1e-05   | 5e-04    | 1e-05   |
| 1455                | 0.92282 | 0.88822 | -0.25232 | 0.30607 | 2e-05    | 0.00052  | 2e-05   |
| 1460                | 0.91806 | 0.91629 | -0.24556 | 0.3273  | 6e-05    | 0.00055  | 4e-05   |
| 1465                | 0.9133  | 0.94406 | -0.24008 | 0.34847 | 1e-04    | 0.00057  | 6e-05   |
| 1470                | 0.90849 | 0.97153 | -0.23576 | 0.36956 | 0.00015  | 0.00058  | 8e-05   |
| 1475                | 0.90359 | 0.99871 | -0.2325  | 0.39056 | 0.00021  | 0.00059  | 0.00011 |
| 1480                | 0.89857 | 1.02561 | -0.2302  | 0.41146 | 0.00027  | 0.00059  | 0.00014 |
| 1485                | 0.89338 | 1.05224 | -0.22876 | 0.43223 | 0.00034  | 0.00059  | 0.00017 |
| 1490                | 0.88799 | 1.0786  | -0.22808 | 0.45286 | 0.00042  | 0.00057  | 2e-04   |
| 1495                | 0.88235 | 1.1047  | -0.22805 | 0.47333 | 5e-04    | 0.00054  | 0.00024 |
| 1500                | 0.87644 | 1.13056 | -0.22858 | 0.49364 | 0.00059  | 0.00049  | 0.00028 |
| 1505                | 0.87021 | 1.15617 | -0.22955 | 0.51376 | 0.00069  | 0.00043  | 0.00033 |
| 1510                | 0.86362 | 1.18155 | -0.23086 | 0.53368 | 8e-04    | 0.00035  | 0.00037 |
| 1515                | 0.85663 | 1.20671 | -0.23242 | 0.55338 | 0.00092  | 0.00026  | 0.00043 |
| 1520                | 0.84921 | 1.23163 | -0.23416 | 0.57284 | 0.00104  | 0.00014  | 0.00048 |
| 1525                | 0.84136 | 1.25616 | -0.23614 | 0.59195 | 0.00118  | 1e-05    | 0.00054 |
| 1530                | 0.83308 | 1.28016 | -0.23847 | 0.6106  | 0.00132  | -0.00015 | 6e-04   |
| 1535                | 0.82437 | 1.30346 | -0.24125 | 0.62869 | 0.00146  | -0.00034 | 0.00066 |
| 1540                | 0.81522 | 1.32589 | -0.24459 | 0.6461  | 0.0016   | -0.00055 | 0.00072 |
| 1545                | 0.80565 | 1.34729 | -0.2486  | 0.66271 | 0.00175  | -8e-04   | 0.00079 |
| 1550                | 0.79564 | 1.3675  | -0.25336 | 0.67841 | 0.00189  | -0.00107 | 0.00085 |
| 1555                | 0.78521 | 1.38636 | -0.259   | 0.6931  | 0.00204  | -0.00138 | 0.00091 |
| 1560                | 0.77436 | 1.4037  | -0.26561 | 0.70666 | 0.00217  | -0.00173 | 0.00096 |
| 1565                | 0.76308 | 1.41937 | -0.2733  | 0.71898 | 0.0023   | -0.00211 | 0.00101 |
| 1570                | 0.75138 | 1.4332  | -0.28217 | 0.72994 | 0.00243  | -0.00254 | 0.00106 |
| 1575                | 0.73925 | 1.44502 | -0.29233 | 0.73943 | 0.00254  | -0.00301 | 0.0011  |
| 1580                | 0.72671 | 1.45474 | -0.30383 | 0.74739 | 0.00264  | -0.00352 | 0.00114 |
| 1585                | 0.71375 | 1.46248 | -0.31657 | 0.75388 | 0.00272  | -0.00407 | 0.00116 |
| 1590                | 0.7004  | 1.46841 | -0.33037 | 0.75901 | 0.00278  | -0.00465 | 0.00118 |
| 1595                | 0.68665 | 1.47272 | -0.3451  | 0.76289 | 0.0028   | -0.00527 | 0.00118 |

Table 41: Normalized Legendre coefficients in  $\pi N \rightarrow \Lambda K$  (3/7)

| Momentum<br>(MeV/c) | A1/A0   | A2/A0   | A3/A0    | A4/A0   | A5/A0    | A6/A0    | A7/A0    |
|---------------------|---------|---------|----------|---------|----------|----------|----------|
| 1600                | 0.67251 | 1.4756  | -0.36058 | 0.76565 | 0.00278  | -0.00591 | 0.00115  |
| 1605                | 0.658   | 1.47722 | -0.37667 | 0.76737 | 0.00272  | -0.00657 | 0.00111  |
| 1610                | 0.64313 | 1.47777 | -0.3932  | 0.76819 | 0.00259  | -0.00725 | 0.00104  |
| 1615                | 0.6279  | 1.47743 | -0.41002 | 0.76821 | 0.00241  | -0.00795 | 0.00094  |
| 1620                | 0.61232 | 1.47637 | -0.42696 | 0.76754 | 0.00215  | -0.00865 | 0.00081  |
| 1625                | 0.59641 | 1.47479 | -0.44387 | 0.76629 | 0.00182  | -0.00935 | 0.00064  |
| 1630                | 0.58017 | 1.47287 | -0.4606  | 0.76457 | 0.0014   | -0.01005 | 0.00043  |
| 1635                | 0.56361 | 1.47078 | -0.47698 | 0.7625  | 0.00089  | -0.01075 | 0.00018  |
| 1640                | 0.54674 | 1.4687  | -0.49286 | 0.76019 | 0.00028  | -0.01143 | -0.00011 |
| 1645                | 0.52957 | 1.46683 | -0.50808 | 0.75774 | -0.00044 | -0.0121  | -0.00045 |
| 1650                | 0.51216 | 1.46529 | -0.5225  | 0.75525 | -0.00127 | -0.01274 | -0.00085 |
| 1655                | 0.49484 | 1.46406 | -0.53609 | 0.75274 | -0.00222 | -0.01333 | -0.0013  |
| 1660                | 0.47796 | 1.46306 | -0.54882 | 0.75023 | -0.0033  | -0.01384 | -0.00181 |
| 1665                | 0.46188 | 1.4622  | -0.56068 | 0.7477  | -0.00452 | -0.01424 | -0.00237 |
| 1670                | 0.44698 | 1.46141 | -0.57165 | 0.74517 | -0.00587 | -0.01449 | -0.003   |
| 1675                | 0.43363 | 1.46061 | -0.58171 | 0.74264 | -0.00737 | -0.01456 | -0.00369 |
| 1680                | 0.42219 | 1.45972 | -0.59084 | 0.74012 | -0.00902 | -0.01443 | -0.00444 |
| 1685                | 0.41302 | 1.45866 | -0.59903 | 0.73761 | -0.01083 | -0.01405 | -0.00527 |
| 1690                | 0.40649 | 1.45737 | -0.60625 | 0.73511 | -0.01281 | -0.01341 | -0.00616 |
| 1695                | 0.40298 | 1.45575 | -0.6125  | 0.73264 | -0.01495 | -0.01246 | -0.00712 |
| 1700                | 0.40284 | 1.45373 | -0.61774 | 0.73018 | -0.01727 | -0.01118 | -0.00816 |
| 1705                | 0.40645 | 1.45123 | -0.62196 | 0.72776 | -0.01978 | -0.00954 | -0.00928 |
| 1710                | 0.41402 | 1.44822 | -0.62516 | 0.72539 | -0.02247 | -0.00749 | -0.01047 |
| 1715                | 0.42517 | 1.44489 | -0.6274  | 0.72323 | -0.02531 | -0.005   | -0.01172 |
| 1720                | 0.43937 | 1.44146 | -0.62876 | 0.72143 | -0.02827 | -0.00201 | -0.01302 |
| 1725                | 0.45609 | 1.43817 | -0.62931 | 0.72016 | -0.0313  | 0.00154  | -0.01434 |
| 1730                | 0.4748  | 1.43525 | -0.62913 | 0.71959 | -0.03438 | 0.00569  | -0.01566 |
| 1735                | 0.49497 | 1.43292 | -0.6283  | 0.71989 | -0.03746 | 0.01051  | -0.01698 |
| 1740                | 0.51607 | 1.43142 | -0.6269  | 0.72121 | -0.04051 | 0.01603  | -0.01826 |
| 1745                | 0.53758 | 1.43098 | -0.62499 | 0.72373 | -0.04349 | 0.02233  | -0.0195  |
| 1750                | 0.55895 | 1.43183 | -0.62267 | 0.7276  | -0.04637 | 0.02944  | -0.02067 |
| 1755                | 0.57967 | 1.4342  | -0.61999 | 0.73301 | -0.0491  | 0.03742  | -0.02175 |
| 1760                | 0.5992  | 1.43833 | -0.61705 | 0.74011 | -0.05165 | 0.04632  | -0.02273 |
| 1765                | 0.61701 | 1.44443 | -0.61392 | 0.74907 | -0.05398 | 0.0562   | -0.0236  |
| 1770                | 0.63257 | 1.45275 | -0.61067 | 0.76005 | -0.05606 | 0.06712  | -0.02432 |
| 1775                | 0.64535 | 1.46351 | -0.60738 | 0.77322 | -0.05785 | 0.07911  | -0.02489 |
| 1780                | 0.65496 | 1.47687 | -0.60408 | 0.78868 | -0.05929 | 0.09221  | -0.02527 |
| 1785                | 0.66162 | 1.49263 | -0.60057 | 0.80621 | -0.06023 | 0.10632  | -0.02541 |
| 1790                | 0.66566 | 1.51054 | -0.5966  | 0.82552 | -0.06051 | 0.12132  | -0.02522 |
| 1795                | 0.66742 | 1.53032 | -0.59194 | 0.84633 | -0.05997 | 0.13708  | -0.02464 |
| 1800                | 0.66727 | 1.55172 | -0.58634 | 0.86836 | -0.05843 | 0.15349  | -0.02359 |
| 1805                | 0.66553 | 1.57446 | -0.57955 | 0.89131 | -0.05573 | 0.17042  | -0.02199 |
| 1810                | 0.66256 | 1.59828 | -0.57132 | 0.9149  | -0.05171 | 0.18775  | -0.01978 |
| 1815                | 0.6587  | 1.62291 | -0.56141 | 0.93885 | -0.04619 | 0.20535  | -0.01688 |

Table 42: Normalized Legendre coefficients in  $\pi N \rightarrow \Lambda K$  (4/7)

| Momentum<br>(MeV/c) | A1/A0   | A2/A0   | A3/A0    | A4/A0   | A5/A0    | A6/A0   | A7/A0    |
|---------------------|---------|---------|----------|---------|----------|---------|----------|
| 1820                | 0.6543  | 1.64809 | -0.54958 | 0.96288 | -0.03901 | 0.2231  | -0.01321 |
| 1825                | 0.64971 | 1.67356 | -0.53558 | 0.98668 | -0.03001 | 0.24088 | -0.00871 |
| 1830                | 0.64526 | 1.69904 | -0.51916 | 1.00999 | -0.01902 | 0.25856 | -0.00329 |
| 1835                | 0.64131 | 1.72427 | -0.50008 | 1.0325  | -0.00587 | 0.27603 | 0.00312  |
| 1840                | 0.63821 | 1.74898 | -0.47809 | 1.05395 | 0.00961  | 0.29315 | 0.01058  |
| 1845                | 0.63629 | 1.77291 | -0.45295 | 1.07404 | 0.02757  | 0.30981 | 0.01917  |
| 1850                | 0.63591 | 1.79579 | -0.42441 | 1.09248 | 0.04819  | 0.32589 | 0.02898  |
| 1855                | 0.63741 | 1.81736 | -0.39222 | 1.10899 | 0.07164  | 0.34125 | 0.04006  |
| 1860                | 0.64113 | 1.83735 | -0.35615 | 1.12328 | 0.09807  | 0.35578 | 0.0525   |
| 1865                | 0.64742 | 1.8555  | -0.31594 | 1.13507 | 0.12766  | 0.36936 | 0.06637  |
| 1870                | 0.65664 | 1.87153 | -0.27136 | 1.14408 | 0.16058  | 0.38186 | 0.08174  |
| 1875                | 0.66911 | 1.88519 | -0.22214 | 1.15001 | 0.19698  | 0.39315 | 0.09868  |
| 1880                | 0.68509 | 1.89627 | -0.16819 | 1.15266 | 0.23695  | 0.40315 | 0.11724  |
| 1885                | 0.70432 | 1.90488 | -0.10992 | 1.15218 | 0.28023  | 0.4119  | 0.1373   |
| 1890                | 0.72647 | 1.91118 | -0.04788 | 1.14879 | 0.3265   | 0.41946 | 0.15872  |
| 1895                | 0.75118 | 1.91533 | 0.01738  | 1.14272 | 0.37541  | 0.42591 | 0.18135  |
| 1900                | 0.77812 | 1.91751 | 0.08531  | 1.13419 | 0.42662  | 0.43131 | 0.20505  |
| 1905                | 0.80692 | 1.91788 | 0.15535  | 1.12342 | 0.47979  | 0.43573 | 0.22967  |
| 1910                | 0.83725 | 1.91661 | 0.22697  | 1.11064 | 0.53459  | 0.43925 | 0.25507  |
| 1915                | 0.86875 | 1.91386 | 0.2996   | 1.09608 | 0.59068  | 0.44194 | 0.28109  |
| 1920                | 0.90109 | 1.90981 | 0.37269  | 1.07996 | 0.64773  | 0.44385 | 0.30761  |
| 1925                | 0.9339  | 1.90461 | 0.4457   | 1.06251 | 0.70538  | 0.44508 | 0.33446  |
| 1930                | 0.96685 | 1.89844 | 0.51808  | 1.04394 | 0.76331  | 0.44567 | 0.36151  |
| 1935                | 0.99958 | 1.89146 | 0.58927  | 1.02449 | 0.82118  | 0.44571 | 0.38861  |
| 1940                | 1.03175 | 1.88384 | 0.65873  | 1.00439 | 0.87864  | 0.44526 | 0.41561  |
| 1945                | 1.06301 | 1.87575 | 0.72589  | 0.98385 | 0.93537  | 0.44439 | 0.44237  |
| 1950                | 1.09301 | 1.86735 | 0.79022  | 0.9631  | 0.99102  | 0.44318 | 0.46874  |
| 1955                | 1.1214  | 1.85881 | 0.85116  | 0.94236 | 1.04526  | 0.44169 | 0.49458  |
| 1960                | 1.14785 | 1.8503  | 0.90817  | 0.92187 | 1.09774  | 0.43999 | 0.51975  |
| 1965                | 1.17199 | 1.84198 | 0.96068  | 0.90184 | 1.14813  | 0.43816 | 0.54408  |
| 1970                | 1.19348 | 1.83402 | 1.00815  | 0.88251 | 1.1961   | 0.43625 | 0.56745  |
| 1975                | 1.21198 | 1.82659 | 1.05004  | 0.86409 | 1.2413   | 0.43435 | 0.58971  |
| 1980                | 1.22713 | 1.81986 | 1.08578  | 0.84681 | 1.28339  | 0.43252 | 0.6107   |
| 1985                | 1.23859 | 1.81398 | 1.11483  | 0.8309  | 1.32204  | 0.43084 | 0.63029  |
| 1990                | 1.24601 | 1.80914 | 1.13664  | 0.81658 | 1.35691  | 0.42936 | 0.64833  |
| 1995                | 1.24905 | 1.80549 | 1.15065  | 0.80408 | 1.38766  | 0.42817 | 0.66467  |
| 2000                | 1.24735 | 1.8032  | 1.15632  | 0.79362 | 1.41396  | 0.42732 | 0.67917  |
| 2005                | 1.2407  | 1.80242 | 1.15334  | 0.78541 | 1.43554  | 0.42692 | 0.6917   |
| 2010                | 1.22949 | 1.80321 | 1.14236  | 0.77959 | 1.45242  | 0.42713 | 0.70224  |
| 2015                | 1.21419 | 1.80564 | 1.12429  | 0.7763  | 1.4647   | 0.42812 | 0.71076  |
| 2020                | 1.19533 | 1.80973 | 1.10003  | 0.77565 | 1.47248  | 0.4301  | 0.71727  |
| 2025                | 1.17341 | 1.81555 | 1.07046  | 0.77778 | 1.47586  | 0.43325 | 0.72176  |
| 2030                | 1.14892 | 1.82314 | 1.0365   | 0.78281 | 1.47493  | 0.43775 | 0.7242   |
| 2035                | 1.12238 | 1.83254 | 0.99904  | 0.79087 | 1.4698   | 0.44379 | 0.7246   |

Table 43: Normalized Legendre coefficients in  $\pi N \rightarrow \Lambda K$  (5/7)

| Momentum<br>(MeV/c) | A1/A0   | A2/A0   | A3/A0   | A4/A0   | A5/A0   | A6/A0   | A7/A0   |
|---------------------|---------|---------|---------|---------|---------|---------|---------|
| 2040                | 1.09429 | 1.84381 | 0.95898 | 0.8021  | 1.46056 | 0.45155 | 0.72294 |
| 2045                | 1.06515 | 1.85699 | 0.91723 | 0.8166  | 1.44731 | 0.46123 | 0.71921 |
| 2050                | 1.03547 | 1.87214 | 0.87467 | 0.83452 | 1.43015 | 0.473   | 0.71341 |
| 2055                | 1.00576 | 1.88929 | 0.83222 | 0.85598 | 1.40917 | 0.48707 | 0.70551 |
| 2060                | 0.97644 | 1.90846 | 0.79062 | 0.88103 | 1.38453 | 0.50353 | 0.69555 |
| 2065                | 0.94767 | 1.92947 | 0.75007 | 0.90941 | 1.35653 | 0.52226 | 0.6837  |
| 2070                | 0.91954 | 1.95211 | 0.71063 | 0.94081 | 1.32555 | 0.54305 | 0.67014 |
| 2075                | 0.89213 | 1.97615 | 0.67234 | 0.97489 | 1.29194 | 0.5657  | 0.65508 |
| 2080                | 0.86552 | 2.0014  | 0.63526 | 1.01133 | 1.25607 | 0.58999 | 0.63872 |
| 2085                | 0.83981 | 2.02762 | 0.59943 | 1.04978 | 1.21831 | 0.61572 | 0.62125 |
| 2090                | 0.81506 | 2.0546  | 0.56491 | 1.08994 | 1.17903 | 0.64269 | 0.60288 |
| 2095                | 0.79138 | 2.08213 | 0.53175 | 1.13146 | 1.13857 | 0.67069 | 0.5838  |
| 2100                | 0.76883 | 2.11    | 0.5     | 1.17402 | 1.09732 | 0.69951 | 0.56422 |
| 2105                | 0.74751 | 2.13798 | 0.46972 | 1.2173  | 1.05563 | 0.72895 | 0.54432 |
| 2110                | 0.72751 | 2.16586 | 0.44094 | 1.26096 | 1.01387 | 0.7588  | 0.52432 |
| 2115                | 0.70889 | 2.19343 | 0.41374 | 1.30467 | 0.9724  | 0.78886 | 0.5044  |
| 2120                | 0.69174 | 2.22049 | 0.38814 | 1.34815 | 0.93155 | 0.81894 | 0.48475 |
| 2125                | 0.67605 | 2.24701 | 0.36417 | 1.39128 | 0.89144 | 0.84898 | 0.46544 |
| 2130                | 0.6618  | 2.27294 | 0.34183 | 1.43399 | 0.85218 | 0.87891 | 0.44653 |
| 2135                | 0.64897 | 2.29827 | 0.32114 | 1.47621 | 0.81386 | 0.90871 | 0.42808 |
| 2140                | 0.63754 | 2.32297 | 0.3021  | 1.51786 | 0.77658 | 0.9383  | 0.41014 |
| 2145                | 0.62749 | 2.34703 | 0.28473 | 1.55887 | 0.74042 | 0.96766 | 0.39278 |
| 2150                | 0.61881 | 2.37041 | 0.26902 | 1.59918 | 0.70547 | 0.99672 | 0.37603 |
| 2155                | 0.61148 | 2.39309 | 0.25499 | 1.63869 | 0.67185 | 1.02545 | 0.35997 |
| 2160                | 0.60547 | 2.41504 | 0.24265 | 1.67735 | 0.63963 | 1.05379 | 0.34465 |
| 2165                | 0.60077 | 2.43625 | 0.23201 | 1.71507 | 0.60891 | 1.08169 | 0.33013 |
| 2170                | 0.59735 | 2.45669 | 0.22308 | 1.75179 | 0.57979 | 1.10911 | 0.31645 |
| 2175                | 0.59521 | 2.47634 | 0.21586 | 1.78743 | 0.55236 | 1.136   | 0.30368 |
| 2180                | 0.59431 | 2.49517 | 0.21037 | 1.82192 | 0.52671 | 1.1623  | 0.29188 |
| 2185                | 0.59465 | 2.51315 | 0.20661 | 1.85518 | 0.50293 | 1.18798 | 0.2811  |
| 2190                | 0.59619 | 2.53027 | 0.20459 | 1.88715 | 0.48113 | 1.21298 | 0.27139 |
| 2195                | 0.59893 | 2.5465  | 0.20433 | 1.91774 | 0.46139 | 1.23725 | 0.26282 |
| 2200                | 0.60284 | 2.56181 | 0.20582 | 1.9469  | 0.44381 | 1.26075 | 0.25544 |
| 2205                | 0.60791 | 2.57618 | 0.20909 | 1.97453 | 0.42849 | 1.28343 | 0.2493  |
| 2210                | 0.61411 | 2.5896  | 0.21413 | 2.00058 | 0.41551 | 1.30524 | 0.24447 |
| 2215                | 0.62143 | 2.60202 | 0.22096 | 2.02496 | 0.40496 | 1.32612 | 0.24099 |
| 2220                | 0.62984 | 2.61344 | 0.22959 | 2.04761 | 0.39696 | 1.34604 | 0.23893 |
| 2225                | 0.63934 | 2.62382 | 0.24002 | 2.06845 | 0.39157 | 1.36495 | 0.23834 |
| 2230                | 0.64989 | 2.63314 | 0.25227 | 2.0874  | 0.38891 | 1.38278 | 0.23928 |
| 2235                | 0.66148 | 2.64138 | 0.26634 | 2.1044  | 0.38907 | 1.39951 | 0.24181 |
| 2240                | 0.67408 | 2.64852 | 0.28223 | 2.1194  | 0.3921  | 1.41509 | 0.24595 |
| 2245                | 0.68768 | 2.6546  | 0.29989 | 2.13244 | 0.39794 | 1.42955 | 0.25168 |
| 2250                | 0.70222 | 2.65965 | 0.31925 | 2.14359 | 0.40647 | 1.44294 | 0.25893 |
| 2255                | 0.71767 | 2.66371 | 0.34024 | 2.15294 | 0.4176  | 1.45528 | 0.26765 |

Table 44: Normalized Legendre coefficients in  $\pi N \rightarrow \Lambda K$  (6/7)

| Momentum<br>(MeV/c) | A1/A0   | A2/A0   | A3/A0   | A4/A0   | A5/A0   | A6/A0   | A7/A0   |
|---------------------|---------|---------|---------|---------|---------|---------|---------|
| 2260                | 0.73399 | 2.66683 | 0.36281 | 2.16054 | 0.43123 | 1.46664 | 0.27777 |
| 2265                | 0.75115 | 2.66903 | 0.38688 | 2.16649 | 0.44724 | 1.47703 | 0.28924 |
| 2270                | 0.76912 | 2.67037 | 0.41239 | 2.17083 | 0.46554 | 1.48652 | 0.30199 |
| 2275                | 0.78785 | 2.67088 | 0.43927 | 2.17366 | 0.48602 | 1.49514 | 0.31598 |
| 2280                | 0.80731 | 2.67059 | 0.46746 | 2.17504 | 0.50857 | 1.50293 | 0.33114 |
| 2285                | 0.82746 | 2.66956 | 0.49689 | 2.17504 | 0.5331  | 1.50993 | 0.34741 |
| 2290                | 0.84826 | 2.66782 | 0.5275  | 2.17375 | 0.55949 | 1.51618 | 0.36473 |
| 2295                | 0.86969 | 2.66541 | 0.55922 | 2.17122 | 0.58765 | 1.52173 | 0.38305 |
| 2300                | 0.89169 | 2.66236 | 0.59199 | 2.16753 | 0.61747 | 1.52662 | 0.40231 |
| 2305                | 0.91425 | 2.65872 | 0.62574 | 2.16276 | 0.64884 | 1.53089 | 0.42244 |
| 2310                | 0.93731 | 2.65453 | 0.6604  | 2.15697 | 0.68167 | 1.53458 | 0.44339 |
| 2315                | 0.96085 | 2.64983 | 0.69591 | 2.15025 | 0.71584 | 1.53773 | 0.46511 |
| 2320                | 0.98482 | 2.64466 | 0.7322  | 2.14266 | 0.75126 | 1.54038 | 0.48752 |
| 2325                | 1.00919 | 2.63905 | 0.76922 | 2.13427 | 0.78782 | 1.54258 | 0.51058 |
| 2330                | 1.03393 | 2.63304 | 0.80688 | 2.12516 | 0.82541 | 1.54437 | 0.53422 |
| 2335                | 1.05899 | 2.62669 | 0.84513 | 2.11541 | 0.86393 | 1.54578 | 0.55838 |
| 2340                | 1.08434 | 2.62001 | 0.88391 | 2.10507 | 0.90328 | 1.54686 | 0.58302 |
| 2345                | 1.10995 | 2.61307 | 0.92313 | 2.09423 | 0.94336 | 1.54766 | 0.60806 |
| 2350                | 1.13577 | 2.60588 | 0.96275 | 2.08296 | 0.98405 | 1.54821 | 0.63345 |
| 2355                | 1.16178 | 2.5985  | 1.0027  | 2.07133 | 1.02526 | 1.54855 | 0.65913 |
| 2360                | 1.18793 | 2.59097 | 1.0429  | 2.05941 | 1.06688 | 1.54873 | 0.68504 |
| 2365                | 1.21419 | 2.58332 | 1.0833  | 2.04728 | 1.10881 | 1.54878 | 0.71113 |
| 2370                | 1.24052 | 2.57559 | 1.12382 | 2.035   | 1.15094 | 1.54876 | 0.73733 |
| 2375                | 1.26688 | 2.56782 | 1.16441 | 2.02266 | 1.19317 | 1.54869 | 0.76358 |

Table 45: Normalized Legendre coefficients in  $\pi N \rightarrow \Lambda K$  (7/7)

| Momentum<br>(MeV/c) | A1/A0    | A2/A0    | A3/A0    | A4/A0    | A5/A0    | A6/A0    | A7/A0 | A8/A0 |
|---------------------|----------|----------|----------|----------|----------|----------|-------|-------|
| 1040                | 0.18188  | -0.04656 | -0.07595 | 0.01513  | 0.00374  | 0.00201  | 0.    | 0.    |
| 1045                | 0.16386  | -0.02812 | -0.07075 | 0.01418  | 0.00298  | 0.00194  | 0.    | 0.    |
| 1050                | 0.14587  | -0.00965 | -0.06554 | 0.01323  | 0.00222  | 0.00187  | 0.    | 0.    |
| 1055                | 0.12793  | 0.00891  | -0.0603  | 0.01228  | 0.00146  | 0.00179  | 0.    | 0.    |
| 1060                | 0.11008  | 0.02758  | -0.05502 | 0.01132  | 7e-04    | 0.00172  | 0.    | 0.    |
| 1065                | 0.09234  | 0.0464   | -0.0497  | 0.01034  | -7e-05   | 0.00165  | 0.    | 0.    |
| 1070                | 0.07475  | 0.06543  | -0.04431 | 0.00936  | -0.00084 | 0.00157  | 0.    | 0.    |
| 1075                | 0.05733  | 0.08469  | -0.03886 | 0.00836  | -0.00161 | 0.00149  | 0.    | 0.    |
| 1080                | 0.04011  | 0.10423  | -0.03331 | 0.00735  | -0.00238 | 0.00141  | 0.    | 0.    |
| 1085                | 0.02312  | 0.12408  | -0.02767 | 0.00631  | -0.00317 | 0.00133  | 0.    | 0.    |
| 1090                | 0.00638  | 0.14429  | -0.02192 | 0.00525  | -0.00395 | 0.00124  | 0.    | 0.    |
| 1095                | -0.01007 | 0.1649   | -0.01605 | 0.00417  | -0.00474 | 0.00116  | 0.    | 0.    |
| 1100                | -0.02621 | 0.18591  | -0.01004 | 0.00306  | -0.00554 | 0.00106  | 0.    | 0.    |
| 1105                | -0.04203 | 0.20727  | -0.00389 | 0.00193  | -0.00635 | 0.00097  | 0.    | 0.    |
| 1110                | -0.05753 | 0.22885  | 0.00243  | 0.00076  | -0.00716 | 0.00086  | 0.    | 0.    |
| 1115                | -0.0727  | 0.25057  | 0.00893  | -0.00045 | -0.00798 | 0.00076  | 0.    | 0.    |
| 1120                | -0.08753 | 0.27232  | 0.01561  | -0.0017  | -0.0088  | 0.00065  | 0.    | 0.    |
| 1125                | -0.10203 | 0.29401  | 0.02251  | -0.00298 | -0.00963 | 0.00053  | 0.    | 0.    |
| 1130                | -0.11619 | 0.31553  | 0.02963  | -0.00432 | -0.01046 | 4e-04    | 0.    | 0.    |
| 1135                | -0.13    | 0.33678  | 0.03699  | -0.0057  | -0.0113  | 0.00027  | 0.    | 0.    |
| 1140                | -0.14346 | 0.35766  | 0.0446   | -0.00713 | -0.01215 | 0.00013  | 0.    | 0.    |
| 1145                | -0.15657 | 0.37808  | 0.05247  | -0.00862 | -0.013   | -1e-05   | 0.    | 0.    |
| 1150                | -0.16932 | 0.39792  | 0.06063  | -0.01016 | -0.01385 | -0.00017 | 0.    | 0.    |
| 1155                | -0.1817  | 0.4171   | 0.06909  | -0.01177 | -0.01472 | -0.00033 | 0.    | 0.    |
| 1160                | -0.19372 | 0.43551  | 0.07785  | -0.01344 | -0.01558 | -0.00051 | 0.    | 0.    |
| 1165                | -0.20536 | 0.45308  | 0.08694  | -0.01518 | -0.01645 | -0.00069 | 0.    | 0.    |
| 1170                | -0.2166  | 0.4698   | 0.09635  | -0.01698 | -0.01732 | -0.00089 | 0.    | 0.    |
| 1175                | -0.22743 | 0.48566  | 0.10609  | -0.01885 | -0.01819 | -0.0011  | 0.    | 0.    |
| 1180                | -0.23783 | 0.50068  | 0.11617  | -0.02079 | -0.01905 | -0.00131 | 0.    | 0.    |
| 1185                | -0.24777 | 0.51485  | 0.12657  | -0.02281 | -0.01991 | -0.00154 | 0.    | 0.    |
| 1190                | -0.25724 | 0.52817  | 0.13732  | -0.02489 | -0.02076 | -0.00178 | 0.    | 0.    |
| 1195                | -0.26622 | 0.54063  | 0.1484   | -0.02705 | -0.0216  | -0.00204 | 0.    | 0.    |
| 1200                | -0.27469 | 0.55225  | 0.15982  | -0.02928 | -0.02242 | -0.00231 | 0.    | 0.    |
| 1205                | -0.28263 | 0.56301  | 0.17159  | -0.03158 | -0.02323 | -0.00259 | 0.    | 0.    |
| 1210                | -0.29002 | 0.57292  | 0.1837   | -0.03396 | -0.02402 | -0.00288 | 0.    | 0.    |
| 1215                | -0.29685 | 0.58199  | 0.19617  | -0.03642 | -0.02478 | -0.00319 | 0.    | 0.    |
| 1220                | -0.30309 | 0.5902   | 0.20898  | -0.03895 | -0.02552 | -0.00352 | 0.    | 0.    |
| 1225                | -0.30872 | 0.59755  | 0.22215  | -0.04156 | -0.02623 | -0.00386 | 0.    | 0.    |
| 1230                | -0.31373 | 0.60409  | 0.23567  | -0.04425 | -0.02691 | -0.00421 | 0.    | 0.    |
| 1235                | -0.31816 | 0.60992  | 0.2495   | -0.04702 | -0.02756 | -0.00459 | 0.    | 0.    |
| 1240                | -0.32203 | 0.61513  | 0.26362  | -0.04984 | -0.02815 | -0.00497 | 0.    | 0.    |
| 1245                | -0.32535 | 0.61986  | 0.27799  | -0.05274 | -0.0287  | -0.00537 | 0.    | 0.    |
| 1250                | -0.32816 | 0.62422  | 0.29257  | -0.05568 | -0.02919 | -0.00579 | 0.    | 0.    |
| 1255                | -0.33049 | 0.62831  | 0.30735  | -0.05868 | -0.02961 | -0.00622 | 0.    | 0.    |
| 1260                | -0.33236 | 0.63225  | 0.32228  | -0.06172 | -0.02996 | -0.00667 | 0.    | 0.    |
| 1265                | -0.3338  | 0.63615  | 0.33733  | -0.0648  | -0.03024 | -0.00713 | 0.    | 0.    |

Table 46: Normalized Legendre coefficients in  $\pi^- p \rightarrow \Sigma^0 K^0$  (1/6)

| Momentum<br>(MeV/c) | A1/A0    | A2/A0   | A3/A0   | A4/A0    | A5/A0    | A6/A0    | A7/A0 | A8/A0 |
|---------------------|----------|---------|---------|----------|----------|----------|-------|-------|
| 1270                | -0.33482 | 0.64013 | 0.35246 | -0.06792 | -0.03042 | -0.0076  | 0.    | 0.    |
| 1275                | -0.33547 | 0.6443  | 0.36766 | -0.07106 | -0.03052 | -0.00809 | 0.    | 0.    |
| 1280                | -0.33576 | 0.64877 | 0.38287 | -0.07422 | -0.03051 | -0.00859 | 0.    | 0.    |
| 1285                | -0.33573 | 0.65366 | 0.39808 | -0.0774  | -0.0304  | -0.00911 | 0.    | 0.    |
| 1290                | -0.33539 | 0.65907 | 0.41324 | -0.0806  | -0.03018 | -0.00964 | 0.    | 0.    |
| 1295                | -0.33477 | 0.6651  | 0.42834 | -0.08379 | -0.02983 | -0.01018 | 0.    | 0.    |
| 1300                | -0.33388 | 0.67178 | 0.44333 | -0.08696 | -0.02935 | -0.01073 | 0.    | 0.    |
| 1305                | -0.33274 | 0.67915 | 0.4582  | -0.0901  | -0.02873 | -0.01129 | 0.    | 0.    |
| 1310                | -0.33138 | 0.68725 | 0.47292 | -0.09319 | -0.02795 | -0.01186 | 0.    | 0.    |
| 1315                | -0.32979 | 0.69613 | 0.48747 | -0.0962  | -0.027   | -0.01244 | 0.    | 0.    |
| 1320                | -0.328   | 0.70582 | 0.50181 | -0.09912 | -0.02587 | -0.01302 | 0.    | 0.    |
| 1325                | -0.32602 | 0.71635 | 0.51593 | -0.10193 | -0.02455 | -0.0136  | 0.    | 0.    |
| 1330                | -0.32387 | 0.72778 | 0.52979 | -0.10461 | -0.02303 | -0.01419 | 0.    | 0.    |
| 1335                | -0.32157 | 0.74013 | 0.54338 | -0.10715 | -0.02129 | -0.01477 | 0.    | 0.    |
| 1340                | -0.31911 | 0.75329 | 0.5567  | -0.10955 | -0.01932 | -0.01535 | 0.    | 0.    |
| 1345                | -0.31652 | 0.76713 | 0.56975 | -0.11183 | -0.01711 | -0.01592 | 0.    | 0.    |
| 1350                | -0.31379 | 0.78149 | 0.58256 | -0.11401 | -0.01463 | -0.01648 | 0.    | 0.    |
| 1355                | -0.31094 | 0.79624 | 0.59512 | -0.11609 | -0.01188 | -0.01702 | 0.    | 0.    |
| 1360                | -0.30797 | 0.81121 | 0.60747 | -0.11811 | -0.00884 | -0.01754 | 0.    | 0.    |
| 1365                | -0.30488 | 0.82628 | 0.6196  | -0.12007 | -0.0055  | -0.01804 | 0.    | 0.    |
| 1370                | -0.30169 | 0.84128 | 0.63153 | -0.12199 | -0.00183 | -0.01851 | 0.    | 0.    |
| 1375                | -0.29841 | 0.85607 | 0.64327 | -0.12389 | 0.00217  | -0.01894 | 0.    | 0.    |
| 1380                | -0.29503 | 0.87051 | 0.65484 | -0.12577 | 0.00653  | -0.01935 | 0.    | 0.    |
| 1385                | -0.29157 | 0.88445 | 0.66625 | -0.12767 | 0.01125  | -0.01971 | 0.    | 0.    |
| 1390                | -0.28803 | 0.89774 | 0.6775  | -0.12959 | 0.01636  | -0.02002 | 0.    | 0.    |
| 1395                | -0.28442 | 0.91023 | 0.68862 | -0.13156 | 0.02186  | -0.02029 | 0.    | 0.    |
| 1400                | -0.28074 | 0.9218  | 0.69961 | -0.13357 | 0.02778  | -0.02051 | 0.    | 0.    |
| 1405                | -0.27699 | 0.9324  | 0.71048 | -0.13564 | 0.03412  | -0.02067 | 0.    | 0.    |
| 1410                | -0.27316 | 0.94199 | 0.72125 | -0.13776 | 0.0409   | -0.02076 | 0.    | 0.    |
| 1415                | -0.26923 | 0.95056 | 0.73193 | -0.13992 | 0.04813  | -0.02077 | 0.    | 0.    |
| 1420                | -0.26519 | 0.95808 | 0.74253 | -0.14212 | 0.05582  | -0.02071 | 0.    | 0.    |
| 1425                | -0.26103 | 0.96451 | 0.75305 | -0.14435 | 0.06398  | -0.02055 | 0.    | 0.    |
| 1430                | -0.25674 | 0.96982 | 0.76351 | -0.1466  | 0.07263  | -0.02031 | 0.    | 0.    |
| 1435                | -0.25231 | 0.97399 | 0.77393 | -0.14888 | 0.08177  | -0.01996 | 0.    | 0.    |
| 1440                | -0.24772 | 0.97699 | 0.7843  | -0.15118 | 0.09142  | -0.0195  | 0.    | 0.    |
| 1445                | -0.24297 | 0.9788  | 0.79465 | -0.15349 | 0.10159  | -0.01892 | 0.    | 0.    |
| 1450                | -0.23805 | 0.97937 | 0.80498 | -0.15581 | 0.11229  | -0.01821 | 0.    | 0.    |
| 1455                | -0.23293 | 0.9787  | 0.81531 | -0.15813 | 0.12353  | -0.01738 | 0.    | 0.    |
| 1460                | -0.22762 | 0.97675 | 0.82564 | -0.16044 | 0.13533  | -0.01641 | 0.    | 0.    |
| 1465                | -0.22209 | 0.97364 | 0.83596 | -0.16272 | 0.14767  | -0.01528 | 0.    | 0.    |
| 1470                | -0.21634 | 0.96945 | 0.84628 | -0.16494 | 0.16055  | -0.014   | 0.    | 0.    |
| 1475                | -0.21034 | 0.96431 | 0.85659 | -0.16707 | 0.17396  | -0.01255 | 0.    | 0.    |
| 1480                | -0.20408 | 0.95831 | 0.86688 | -0.16907 | 0.1879   | -0.01092 | 0.    | 0.    |
| 1485                | -0.19755 | 0.95157 | 0.87714 | -0.17092 | 0.20235  | -0.00911 | 0.    | 0.    |

Table 47: Normalized Legendre coefficients in  $\pi^- p \rightarrow \Sigma^0 K^0$  (2/6)

| Momentum<br>(MeV/c) | A1/A0    | A2/A0   | A3/A0   | A4/A0    | A5/A0   | A6/A0    | A7/A0 | A8/A0 |
|---------------------|----------|---------|---------|----------|---------|----------|-------|-------|
| 1490                | -0.19073 | 0.9442  | 0.88738 | -0.17258 | 0.21731 | -0.00709 | 0.    | 0.    |
| 1495                | -0.18361 | 0.9363  | 0.89758 | -0.17403 | 0.23277 | -0.00486 | 0.    | 0.    |
| 1500                | -0.17616 | 0.92798 | 0.90773 | -0.17524 | 0.24872 | -0.00242 | 0.    | 0.    |
| 1505                | -0.16839 | 0.91935 | 0.91784 | -0.17617 | 0.26515 | 0.00026  | 0.    | 0.    |
| 1510                | -0.16026 | 0.91051 | 0.92789 | -0.17679 | 0.28206 | 0.00317  | 0.    | 0.    |
| 1515                | -0.15177 | 0.90158 | 0.93788 | -0.17708 | 0.29943 | 0.00633  | 0.    | 0.    |
| 1520                | -0.14291 | 0.89266 | 0.9478  | -0.177   | 0.31726 | 0.00976  | 0.    | 0.    |
| 1525                | -0.13368 | 0.88383 | 0.95762 | -0.1765  | 0.33549 | 0.01345  | 0.    | 0.    |
| 1530                | -0.1241  | 0.87515 | 0.9673  | -0.17551 | 0.35406 | 0.01741  | 0.    | 0.    |
| 1535                | -0.11418 | 0.86671 | 0.9768  | -0.17398 | 0.37293 | 0.02167  | 0.    | 0.    |
| 1540                | -0.10394 | 0.85857 | 0.98609 | -0.17185 | 0.39203 | 0.02622  | 0.    | 0.    |
| 1545                | -0.09338 | 0.85081 | 0.99514 | -0.16906 | 0.41131 | 0.03107  | 0.    | 0.    |
| 1550                | -0.08253 | 0.84351 | 1.0039  | -0.16555 | 0.43072 | 0.03623  | 0.    | 0.    |
| 1555                | -0.0714  | 0.83672 | 1.01235 | -0.16127 | 0.45019 | 0.04172  | 0.    | 0.    |
| 1560                | -0.05999 | 0.83054 | 1.02044 | -0.15615 | 0.46967 | 0.04754  | 0.    | 0.    |
| 1565                | -0.04833 | 0.82502 | 1.02813 | -0.15013 | 0.48911 | 0.0537   | 0.    | 0.    |
| 1570                | -0.03643 | 0.82025 | 1.0354  | -0.14316 | 0.50844 | 0.06021  | 0.    | 0.    |
| 1575                | -0.02429 | 0.81629 | 1.04221 | -0.13518 | 0.52762 | 0.06708  | 0.    | 0.    |
| 1580                | -0.01194 | 0.8132  | 1.04852 | -0.12614 | 0.54659 | 0.07431  | 0.    | 0.    |
| 1585                | 6e-04    | 0.81094 | 1.05435 | -0.11607 | 0.56533 | 0.08191  | 0.    | 0.    |
| 1590                | 0.01333  | 0.80944 | 1.0597  | -0.10499 | 0.58383 | 0.08987  | 0.    | 0.    |
| 1595                | 0.02622  | 0.80866 | 1.06461 | -0.09294 | 0.60206 | 0.0982   | 0.    | 0.    |
| 1600                | 0.03926  | 0.80853 | 1.06907 | -0.07995 | 0.62002 | 0.10688  | 0.    | 0.    |
| 1605                | 0.05242  | 0.80899 | 1.0731  | -0.06606 | 0.63769 | 0.11592  | 0.    | 0.    |
| 1610                | 0.06569  | 0.80999 | 1.07673 | -0.0513  | 0.65505 | 0.12532  | 0.    | 0.    |
| 1615                | 0.07905  | 0.81145 | 1.07996 | -0.03571 | 0.67209 | 0.13508  | 0.    | 0.    |
| 1620                | 0.09249  | 0.81333 | 1.08281 | -0.01931 | 0.6888  | 0.14519  | 0.    | 0.    |
| 1625                | 0.10598  | 0.81556 | 1.08529 | -0.00214 | 0.70514 | 0.15565  | 0.    | 0.    |
| 1630                | 0.11951  | 0.81809 | 1.08742 | 0.01576  | 0.72112 | 0.16646  | 0.    | 0.    |
| 1635                | 0.13306  | 0.82085 | 1.08922 | 0.03437  | 0.73672 | 0.17762  | 0.    | 0.    |
| 1640                | 0.14662  | 0.82378 | 1.09069 | 0.05364  | 0.75191 | 0.18912  | 0.    | 0.    |
| 1645                | 0.16016  | 0.82683 | 1.09186 | 0.07355  | 0.76669 | 0.20097  | 0.    | 0.    |
| 1650                | 0.17367  | 0.82994 | 1.09274 | 0.09406  | 0.78104 | 0.21316  | 0.    | 0.    |
| 1655                | 0.18715  | 0.83306 | 1.09333 | 0.11511  | 0.79498 | 0.22566  | 0.    | 0.    |
| 1660                | 0.20061  | 0.83616 | 1.09366 | 0.13665  | 0.80851 | 0.23843  | 0.    | 0.    |
| 1665                | 0.21404  | 0.8392  | 1.09373 | 0.15861  | 0.82165 | 0.25144  | 0.    | 0.    |
| 1670                | 0.22745  | 0.84213 | 1.09356 | 0.18094  | 0.83442 | 0.26466  | 0.    | 0.    |
| 1675                | 0.24084  | 0.84492 | 1.09315 | 0.20358  | 0.84682 | 0.27805  | 0.    | 0.    |
| 1680                | 0.25423  | 0.84753 | 1.09251 | 0.22648  | 0.85888 | 0.29158  | 0.    | 0.    |
| 1685                | 0.2676   | 0.84991 | 1.09167 | 0.24957  | 0.8706  | 0.30522  | 0.    | 0.    |
| 1690                | 0.28096  | 0.85203 | 1.09062 | 0.2728   | 0.882   | 0.31892  | 0.    | 0.    |
| 1695                | 0.29432  | 0.85385 | 1.08938 | 0.29611  | 0.8931  | 0.33266  | 0.    | 0.    |
| 1700                | 0.30768  | 0.85532 | 1.08797 | 0.31943  | 0.9039  | 0.34641  | 0.    | 0.    |
| 1705                | 0.32104  | 0.85641 | 1.08639 | 0.34272  | 0.91442 | 0.36013  | 0.    | 0.    |

Table 48: Normalized Legendre coefficients in  $\pi^- p \rightarrow \Sigma^0 K^0$  (3/6)



| Momentum<br>(MeV/c) | A1/A0   | A2/A0   | A3/A0   | A4/A0   | A5/A0   | A6/A0   | A7/A0 | A8/A0 |
|---------------------|---------|---------|---------|---------|---------|---------|-------|-------|
| 1710                | 0.33441 | 0.85709 | 1.08465 | 0.36592 | 0.92468 | 0.37378 | 0.    | 0.    |
| 1715                | 0.34774 | 0.8574  | 1.08275 | 0.389   | 0.93468 | 0.38736 | 0.    | 0.    |
| 1720                | 0.36102 | 0.85739 | 1.08069 | 0.41194 | 0.94443 | 0.40084 | 0.    | 0.    |
| 1725                | 0.3742  | 0.85709 | 1.07845 | 0.43471 | 0.95393 | 0.41423 | 0.    | 0.    |
| 1730                | 0.38726 | 0.85657 | 1.07604 | 0.45729 | 0.9632  | 0.42751 | 0.    | 0.    |
| 1735                | 0.40016 | 0.85586 | 1.07344 | 0.47966 | 0.97223 | 0.44067 | 0.    | 0.    |
| 1740                | 0.41288 | 0.85501 | 1.07065 | 0.5018  | 0.98104 | 0.45369 | 0.    | 0.    |
| 1745                | 0.42537 | 0.85408 | 1.06767 | 0.52368 | 0.98963 | 0.46656 | 0.    | 0.    |
| 1750                | 0.43761 | 0.85312 | 1.06448 | 0.54527 | 0.99801 | 0.47928 | 0.    | 0.    |
| 1755                | 0.44956 | 0.85216 | 1.06109 | 0.56656 | 1.00619 | 0.49182 | 0.    | 0.    |
| 1760                | 0.4612  | 0.85126 | 1.05749 | 0.58752 | 1.01417 | 0.50419 | 0.    | 0.    |
| 1765                | 0.47248 | 0.85047 | 1.05367 | 0.60813 | 1.02196 | 0.51636 | 0.    | 0.    |
| 1770                | 0.48338 | 0.84982 | 1.04962 | 0.62836 | 1.02956 | 0.52834 | 0.    | 0.    |
| 1775                | 0.49387 | 0.84939 | 1.04535 | 0.6482  | 1.03699 | 0.54009 | 0.    | 0.    |
| 1780                | 0.50391 | 0.84919 | 1.04084 | 0.66762 | 1.04424 | 0.55162 | 0.    | 0.    |
| 1785                | 0.51352 | 0.84924 | 1.0361  | 0.68662 | 1.05131 | 0.56292 | 0.    | 0.    |
| 1790                | 0.52271 | 0.84953 | 1.03113 | 0.70521 | 1.05818 | 0.57399 | 0.    | 0.    |
| 1795                | 0.53149 | 0.85007 | 1.02593 | 0.72339 | 1.06484 | 0.58483 | 0.    | 0.    |
| 1800                | 0.53988 | 0.85085 | 1.02049 | 0.74116 | 1.07128 | 0.59544 | 0.    | 0.    |
| 1805                | 0.54788 | 0.85186 | 1.01483 | 0.75854 | 1.07748 | 0.6058  | 0.    | 0.    |
| 1810                | 0.55553 | 0.85311 | 1.00895 | 0.77552 | 1.08342 | 0.61593 | 0.    | 0.    |
| 1815                | 0.56281 | 0.85459 | 1.00284 | 0.79211 | 1.0891  | 0.62582 | 0.    | 0.    |
| 1820                | 0.56976 | 0.8563  | 0.9965  | 0.80831 | 1.0945  | 0.63547 | 0.    | 0.    |
| 1825                | 0.57638 | 0.85823 | 0.98994 | 0.82413 | 1.0996  | 0.64487 | 0.    | 0.    |
| 1830                | 0.58269 | 0.86039 | 0.98317 | 0.83957 | 1.1044  | 0.65403 | 0.    | 0.    |
| 1835                | 0.58871 | 0.86277 | 0.97617 | 0.85463 | 1.10887 | 0.66293 | 0.    | 0.    |
| 1840                | 0.59443 | 0.86538 | 0.96896 | 0.86933 | 1.11301 | 0.67159 | 0.    | 0.    |
| 1845                | 0.59989 | 0.86819 | 0.96153 | 0.88366 | 1.11681 | 0.68    | 0.    | 0.    |
| 1850                | 0.60508 | 0.87122 | 0.95388 | 0.89763 | 1.12024 | 0.68815 | 0.    | 0.    |
| 1855                | 0.61003 | 0.87447 | 0.94602 | 0.91124 | 1.12329 | 0.69605 | 0.    | 0.    |
| 1860                | 0.61475 | 0.87792 | 0.93795 | 0.9245  | 1.12596 | 0.70369 | 0.    | 0.    |
| 1865                | 0.61926 | 0.88158 | 0.92967 | 0.93741 | 1.12822 | 0.71107 | 0.    | 0.    |
| 1870                | 0.62356 | 0.88544 | 0.92118 | 0.94998 | 1.13006 | 0.71818 | 0.    | 0.    |
| 1875                | 0.62767 | 0.88951 | 0.91248 | 0.9622  | 1.13148 | 0.72504 | 0.    | 0.    |
| 1880                | 0.6316  | 0.89378 | 0.90358 | 0.97409 | 1.13245 | 0.73163 | 0.    | 0.    |
| 1885                | 0.63537 | 0.89833 | 0.89449 | 0.98565 | 1.133   | 0.73795 | 0.    | 0.    |
| 1890                | 0.63898 | 0.90323 | 0.88523 | 0.99687 | 1.13314 | 0.744   | 0.    | 0.    |
| 1895                | 0.64246 | 0.90855 | 0.87582 | 1.00776 | 1.13289 | 0.74977 | 0.    | 0.    |
| 1900                | 0.64581 | 0.91436 | 0.86626 | 1.01832 | 1.13227 | 0.75527 | 0.    | 0.    |
| 1905                | 0.64904 | 0.92075 | 0.85659 | 1.02854 | 1.1313  | 0.76049 | 0.    | 0.    |
| 1910                | 0.65217 | 0.92778 | 0.84681 | 1.03844 | 1.12999 | 0.76543 | 0.    | 0.    |
| 1915                | 0.65522 | 0.93553 | 0.83694 | 1.048   | 1.12837 | 0.77008 | 0.    | 0.    |
| 1920                | 0.65818 | 0.94407 | 0.82701 | 1.05723 | 1.12645 | 0.77445 | 0.    | 0.    |
| 1925                | 0.66108 | 0.95349 | 0.81703 | 1.06614 | 1.12425 | 0.77852 | 0.    | 0.    |

Table 49: Normalized Legendre coefficients in  $\pi^- p \rightarrow \Sigma^0 K^0$  (4/6)

| Momentum<br>(MeV/c) | A1/A0   | A2/A0   | A3/A0   | A4/A0   | A5/A0   | A6/A0   | A7/A0 | A8/A0 |
|---------------------|---------|---------|---------|---------|---------|---------|-------|-------|
| 1930                | 0.66392 | 0.96384 | 0.80701 | 1.07471 | 1.12178 | 0.7823  | 0.    | 0.    |
| 1935                | 0.66673 | 0.97522 | 0.79697 | 1.08296 | 1.11907 | 0.78579 | 0.    | 0.    |
| 1940                | 0.6695  | 0.98768 | 0.78693 | 1.09088 | 1.11614 | 0.78898 | 0.    | 0.    |
| 1945                | 0.67226 | 1.00132 | 0.77691 | 1.09848 | 1.113   | 0.79186 | 0.    | 0.    |
| 1950                | 0.67502 | 1.01619 | 0.76692 | 1.10575 | 1.10967 | 0.79444 | 0.    | 0.    |
| 1955                | 0.67778 | 1.03238 | 0.75698 | 1.11269 | 1.10617 | 0.79672 | 0.    | 0.    |
| 1960                | 0.68056 | 1.04995 | 0.74712 | 1.11931 | 1.10252 | 0.79868 | 0.    | 0.    |
| 1965                | 0.68338 | 1.06899 | 0.73733 | 1.12561 | 1.09874 | 0.80033 | 0.    | 0.    |
| 1970                | 0.68624 | 1.08957 | 0.72765 | 1.13158 | 1.09484 | 0.80167 | 0.    | 0.    |
| 1975                | 0.68916 | 1.11176 | 0.71809 | 1.13724 | 1.09084 | 0.80269 | 0.    | 0.    |
| 1980                | 0.69215 | 1.13564 | 0.70866 | 1.14257 | 1.08676 | 0.80339 | 0.    | 0.    |
| 1985                | 0.69523 | 1.16128 | 0.69939 | 1.14758 | 1.08262 | 0.80376 | 0.    | 0.    |
| 1990                | 0.6984  | 1.18876 | 0.69029 | 1.15227 | 1.07844 | 0.80381 | 0.    | 0.    |
| 1995                | 0.70167 | 1.21815 | 0.68138 | 1.15664 | 1.07423 | 0.80353 | 0.    | 0.    |
| 2000                | 0.70507 | 1.24952 | 0.67267 | 1.1607  | 1.07002 | 0.80292 | 0.    | 0.    |
| 2005                | 0.70859 | 1.2829  | 0.66418 | 1.16444 | 1.06581 | 0.80198 | 0.    | 0.    |
| 2010                | 0.71222 | 1.31813 | 0.6559  | 1.16793 | 1.06158 | 0.80076 | 0.    | 0.    |
| 2015                | 0.71594 | 1.35499 | 0.64783 | 1.17122 | 1.05728 | 0.79932 | 0.    | 0.    |
| 2020                | 0.71974 | 1.39327 | 0.63995 | 1.17438 | 1.05289 | 0.7977  | 0.    | 0.    |
| 2025                | 0.72358 | 1.43275 | 0.63226 | 1.17745 | 1.04836 | 0.79597 | 0.    | 0.    |
| 2030                | 0.72745 | 1.47323 | 0.62475 | 1.18051 | 1.04367 | 0.79418 | 0.    | 0.    |
| 2035                | 0.73133 | 1.51448 | 0.6174  | 1.18361 | 1.03876 | 0.79238 | 0.    | 0.    |
| 2040                | 0.73519 | 1.5563  | 0.61021 | 1.18681 | 1.03362 | 0.79063 | 0.    | 0.    |
| 2045                | 0.73903 | 1.59846 | 0.60318 | 1.19018 | 1.02819 | 0.78898 | 0.    | 0.    |
| 2050                | 0.74281 | 1.64077 | 0.59628 | 1.19377 | 1.02245 | 0.78748 | 0.    | 0.    |
| 2055                | 0.74651 | 1.683   | 0.58951 | 1.19764 | 1.01636 | 0.7862  | 0.    | 0.    |
| 2060                | 0.75013 | 1.72495 | 0.58287 | 1.20184 | 1.00989 | 0.78518 | 0.    | 0.    |
| 2065                | 0.75367 | 1.76647 | 0.57638 | 1.20635 | 1.00308 | 0.78441 | 0.    | 0.    |
| 2070                | 0.75714 | 1.80742 | 0.57004 | 1.21116 | 0.99597 | 0.78388 | 0.    | 0.    |
| 2075                | 0.76056 | 1.84767 | 0.56388 | 1.21622 | 0.98861 | 0.7836  | 0.    | 0.    |
| 2080                | 0.76395 | 1.88707 | 0.55791 | 1.22151 | 0.98104 | 0.78355 | 0.    | 0.    |
| 2085                | 0.76732 | 1.92548 | 0.55216 | 1.227   | 0.97332 | 0.78371 | 0.    | 0.    |
| 2090                | 0.77069 | 1.96276 | 0.54665 | 1.23267 | 0.96548 | 0.78409 | 0.    | 0.    |
| 2095                | 0.77407 | 1.99878 | 0.54138 | 1.23849 | 0.95758 | 0.78467 | 0.    | 0.    |
| 2100                | 0.77748 | 2.03339 | 0.53639 | 1.24443 | 0.94966 | 0.78545 | 0.    | 0.    |
| 2105                | 0.78093 | 2.06646 | 0.53168 | 1.25046 | 0.94176 | 0.7864  | 0.    | 0.    |
| 2110                | 0.78443 | 2.09785 | 0.52728 | 1.25655 | 0.93393 | 0.78754 | 0.    | 0.    |
| 2115                | 0.78801 | 2.12741 | 0.5232  | 1.26267 | 0.92622 | 0.78884 | 0.    | 0.    |
| 2120                | 0.79168 | 2.15503 | 0.51946 | 1.26881 | 0.91867 | 0.79029 | 0.    | 0.    |
| 2125                | 0.79544 | 2.18067 | 0.51607 | 1.27496 | 0.91132 | 0.79191 | 0.    | 0.    |
| 2130                | 0.79929 | 2.20434 | 0.51302 | 1.28111 | 0.9042  | 0.79369 | 0.    | 0.    |
| 2135                | 0.80323 | 2.226   | 0.51031 | 1.28726 | 0.89735 | 0.79563 | 0.    | 0.    |
| 2140                | 0.80726 | 2.24567 | 0.50795 | 1.29342 | 0.89079 | 0.79774 | 0.    | 0.    |
| 2145                | 0.81139 | 2.26332 | 0.50593 | 1.29958 | 0.88457 | 0.80002 | 0.    | 0.    |

Table 50: Normalized Legendre coefficients in  $\pi^- p \rightarrow \Sigma^0 K^0$  (5/6)

| Momentum<br>(MeV/c) | A1/A0   | A2/A0   | A3/A0   | A4/A0   | A5/A0   | A6/A0   | A7/A0 | A8/A0 |
|---------------------|---------|---------|---------|---------|---------|---------|-------|-------|
| 2150                | 0.81561 | 2.27894 | 0.50426 | 1.30575 | 0.87871 | 0.80247 | 0.    | 0.    |
| 2155                | 0.81994 | 2.29253 | 0.50293 | 1.31191 | 0.87325 | 0.80509 | 0.    | 0.    |
| 2160                | 0.82435 | 2.30407 | 0.50195 | 1.31807 | 0.86823 | 0.80789 | 0.    | 0.    |
| 2165                | 0.82887 | 2.31355 | 0.50131 | 1.32423 | 0.86368 | 0.81087 | 0.    | 0.    |
| 2170                | 0.83349 | 2.32096 | 0.50102 | 1.33039 | 0.85963 | 0.81403 | 0.    | 0.    |
| 2175                | 0.83821 | 2.3263  | 0.50107 | 1.33654 | 0.85612 | 0.81737 | 0.    | 0.    |
| 2180                | 0.84303 | 2.32955 | 0.50147 | 1.34269 | 0.85317 | 0.8209  | 0.    | 0.    |
| 2185                | 0.84796 | 2.33069 | 0.50221 | 1.34883 | 0.85083 | 0.82462 | 0.    | 0.    |
| 2190                | 0.85299 | 2.32973 | 0.5033  | 1.35497 | 0.84913 | 0.82852 | 0.    | 0.    |
| 2195                | 0.85813 | 2.32665 | 0.50473 | 1.3611  | 0.8481  | 0.83262 | 0.    | 0.    |
| 2200                | 0.86337 | 2.32144 | 0.50652 | 1.36722 | 0.84778 | 0.83692 | 0.    | 0.    |
| 2205                | 0.86873 | 2.31409 | 0.50865 | 1.37333 | 0.8482  | 0.84141 | 0.    | 0.    |
| 2210                | 0.87419 | 2.30458 | 0.51112 | 1.37943 | 0.84939 | 0.84611 | 0.    | 0.    |
| 2215                | 0.87976 | 2.29291 | 0.51395 | 1.38551 | 0.85138 | 0.851   | 0.    | 0.    |
| 2220                | 0.88545 | 2.27907 | 0.51712 | 1.39159 | 0.85422 | 0.8561  | 0.    | 0.    |
| 2225                | 0.89125 | 2.26305 | 0.52063 | 1.39765 | 0.85794 | 0.86141 | 0.    | 0.    |
| 2230                | 0.89716 | 2.24483 | 0.5245  | 1.40369 | 0.86256 | 0.86693 | 0.    | 0.    |
| 2235                | 0.90319 | 2.22441 | 0.52871 | 1.40972 | 0.86813 | 0.87267 | 0.    | 0.    |
| 2240                | 0.90933 | 2.20179 | 0.53328 | 1.41573 | 0.87466 | 0.87861 | 0.    | 0.    |
| 2245                | 0.91559 | 2.17703 | 0.53817 | 1.42173 | 0.88214 | 0.88476 | 0.    | 0.    |
| 2250                | 0.92195 | 2.15022 | 0.54339 | 1.42771 | 0.89052 | 0.89111 | 0.    | 0.    |
| 2255                | 0.92842 | 2.12143 | 0.54892 | 1.43367 | 0.89978 | 0.89766 | 0.    | 0.    |
| 2260                | 0.93499 | 2.09074 | 0.55475 | 1.43962 | 0.90987 | 0.90438 | 0.    | 0.    |
| 2265                | 0.94165 | 2.05824 | 0.56086 | 1.44556 | 0.92077 | 0.91129 | 0.    | 0.    |
| 2270                | 0.94841 | 2.02399 | 0.56725 | 1.45148 | 0.93243 | 0.91836 | 0.    | 0.    |
| 2275                | 0.95525 | 1.98809 | 0.5739  | 1.45739 | 0.94483 | 0.92559 | 0.    | 0.    |
| 2280                | 0.96218 | 1.9506  | 0.5808  | 1.46328 | 0.95792 | 0.93298 | 0.    | 0.    |
| 2285                | 0.96919 | 1.91161 | 0.58793 | 1.46917 | 0.97168 | 0.94051 | 0.    | 0.    |
| 2290                | 0.97627 | 1.8712  | 0.59529 | 1.47504 | 0.98606 | 0.94818 | 0.    | 0.    |
| 2295                | 0.98342 | 1.82945 | 0.60286 | 1.48091 | 1.00104 | 0.95598 | 0.    | 0.    |
| 2300                | 0.99064 | 1.78643 | 0.61063 | 1.48676 | 1.01657 | 0.96391 | 0.    | 0.    |
| 2305                | 0.99792 | 1.74223 | 0.61858 | 1.49261 | 1.03263 | 0.97194 | 0.    | 0.    |
| 2310                | 1.00526 | 1.69692 | 0.62671 | 1.49844 | 1.04917 | 0.98009 | 0.    | 0.    |
| 2315                | 1.01265 | 1.65058 | 0.635   | 1.50427 | 1.06617 | 0.98833 | 0.    | 0.    |
| 2320                | 1.02009 | 1.6033  | 0.64344 | 1.51009 | 1.08358 | 0.99667 | 0.    | 0.    |
| 2325                | 1.02758 | 1.55515 | 0.65201 | 1.51591 | 1.10138 | 1.00509 | 0.    | 0.    |
| 2330                | 1.03511 | 1.50621 | 0.66071 | 1.52172 | 1.11953 | 1.01359 | 0.    | 0.    |
| 2335                | 1.04268 | 1.45656 | 0.66952 | 1.52752 | 1.13799 | 1.02215 | 0.    | 0.    |
| 2340                | 1.05028 | 1.40628 | 0.67843 | 1.53332 | 1.15672 | 1.03078 | 0.    | 0.    |
| 2345                | 1.05791 | 1.35545 | 0.68743 | 1.53911 | 1.1757  | 1.03946 | 0.    | 0.    |
| 2350                | 1.06556 | 1.30415 | 0.6965  | 1.5449  | 1.19489 | 1.04819 | 0.    | 0.    |
| 2355                | 1.07323 | 1.25246 | 0.70563 | 1.55069 | 1.21425 | 1.05695 | 0.    | 0.    |
| 2360                | 1.08093 | 1.20045 | 0.71481 | 1.55647 | 1.23375 | 1.06575 | 0.    | 0.    |
| 2365                | 1.08863 | 1.14821 | 0.72403 | 1.56225 | 1.25335 | 1.07456 | 0.    | 0.    |
| 2370                | 1.09634 | 1.09581 | 0.73327 | 1.56804 | 1.27302 | 1.0834  | 0.    | 0.    |
| 2375                | 1.10406 | 1.04334 | 0.74253 | 1.57382 | 1.29273 | 1.09224 | 0.    | 0.    |

Table 51: Normalized Legendre coefficients in  $\pi^- p \rightarrow \Sigma^0 K^0$  (6/6)

| Momentum<br>(MeV/c) | A1/A0    | A2/A0    | A3/A0   | A4/A0    | A5/A0   | A6/A0    | A7/A0    | A8/A0    |
|---------------------|----------|----------|---------|----------|---------|----------|----------|----------|
| 1105                | -0.94614 | 0.13062  | 0.15332 | -0.38197 | 0.29933 | -0.63182 | 0.22245  | 0.2047   |
| 1110                | -0.92514 | 0.10676  | 0.19258 | -0.38582 | 0.29026 | -0.59597 | 0.2148   | 0.19724  |
| 1115                | -0.90417 | 0.08301  | 0.23175 | -0.38957 | 0.28119 | -0.56031 | 0.20716  | 0.18979  |
| 1120                | -0.88327 | 0.05949  | 0.27072 | -0.39315 | 0.27209 | -0.52506 | 0.19953  | 0.18234  |
| 1125                | -0.86247 | 0.03632  | 0.30939 | -0.39646 | 0.26297 | -0.49042 | 0.19192  | 0.17492  |
| 1130                | -0.8418  | 0.01362  | 0.34765 | -0.39941 | 0.25382 | -0.45659 | 0.18434  | 0.16751  |
| 1135                | -0.82129 | -0.00851 | 0.38541 | -0.40192 | 0.24462 | -0.42377 | 0.17679  | 0.16012  |
| 1140                | -0.80099 | -0.02993 | 0.42257 | -0.40389 | 0.23536 | -0.39217 | 0.16929  | 0.15276  |
| 1145                | -0.78091 | -0.05054 | 0.45902 | -0.40522 | 0.22604 | -0.36199 | 0.16183  | 0.14544  |
| 1150                | -0.7611  | -0.07022 | 0.49467 | -0.40585 | 0.21665 | -0.33343 | 0.15443  | 0.13815  |
| 1155                | -0.74159 | -0.08885 | 0.52941 | -0.40566 | 0.20717 | -0.3067  | 0.1471   | 0.1309   |
| 1160                | -0.7224  | -0.10632 | 0.56314 | -0.40458 | 0.19761 | -0.282   | 0.13983  | 0.12371  |
| 1165                | -0.70354 | -0.12258 | 0.59581 | -0.40256 | 0.18797 | -0.25936 | 0.13263  | 0.11656  |
| 1170                | -0.68498 | -0.13762 | 0.62737 | -0.39958 | 0.17827 | -0.2387  | 0.12553  | 0.10948  |
| 1175                | -0.66669 | -0.15144 | 0.65779 | -0.39563 | 0.16855 | -0.21996 | 0.11851  | 0.10247  |
| 1180                | -0.64863 | -0.16402 | 0.68704 | -0.39067 | 0.15883 | -0.20306 | 0.11159  | 0.09553  |
| 1185                | -0.63078 | -0.17537 | 0.71507 | -0.38471 | 0.14914 | -0.18792 | 0.10479  | 0.08867  |
| 1190                | -0.61311 | -0.18548 | 0.74186 | -0.37772 | 0.1395  | -0.17446 | 0.09809  | 0.0819   |
| 1195                | -0.5956  | -0.19435 | 0.76737 | -0.36969 | 0.12994 | -0.16261 | 0.09152  | 0.07523  |
| 1200                | -0.5782  | -0.20196 | 0.79156 | -0.3606  | 0.1205  | -0.15229 | 0.08509  | 0.06867  |
| 1205                | -0.56089 | -0.20832 | 0.8144  | -0.35042 | 0.11118 | -0.14342 | 0.07879  | 0.06221  |
| 1210                | -0.54365 | -0.21341 | 0.83585 | -0.33915 | 0.10203 | -0.13593 | 0.07264  | 0.05588  |
| 1215                | -0.52644 | -0.21724 | 0.85588 | -0.32677 | 0.09306 | -0.12974 | 0.06664  | 0.04967  |
| 1220                | -0.50923 | -0.2198  | 0.87445 | -0.31326 | 0.08431 | -0.12478 | 0.06081  | 0.0436   |
| 1225                | -0.49204 | -0.22113 | 0.89156 | -0.29867 | 0.07581 | -0.12094 | 0.05514  | 0.03766  |
| 1230                | -0.4749  | -0.22129 | 0.90727 | -0.28311 | 0.06762 | -0.11813 | 0.04963  | 0.03185  |
| 1235                | -0.45787 | -0.22038 | 0.92164 | -0.26669 | 0.0598  | -0.11623 | 0.04427  | 0.02618  |
| 1240                | -0.44101 | -0.21848 | 0.93471 | -0.24955 | 0.05241 | -0.11512 | 0.03907  | 0.02064  |
| 1245                | -0.42437 | -0.21567 | 0.94654 | -0.2318  | 0.04551 | -0.1147  | 0.03402  | 0.01523  |
| 1250                | -0.40799 | -0.21204 | 0.95719 | -0.21357 | 0.03915 | -0.11485 | 0.0291   | 0.00995  |
| 1255                | -0.39194 | -0.20767 | 0.96672 | -0.19496 | 0.03339 | -0.11546 | 0.02432  | 0.00479  |
| 1260                | -0.37626 | -0.20265 | 0.97517 | -0.17612 | 0.02829 | -0.11642 | 0.01967  | -0.00025 |
| 1265                | -0.36101 | -0.19705 | 0.9826  | -0.15715 | 0.02391 | -0.11761 | 0.01515  | -0.00517 |
| 1270                | -0.34624 | -0.19097 | 0.98907 | -0.13818 | 0.02031 | -0.11893 | 0.01075  | -0.00997 |
| 1275                | -0.33201 | -0.18448 | 0.99464 | -0.11933 | 0.01754 | -0.12026 | 0.00646  | -0.01465 |
| 1280                | -0.31836 | -0.17767 | 0.99935 | -0.10071 | 0.01566 | -0.12149 | 0.00229  | -0.01922 |
| 1285                | -0.30534 | -0.17062 | 1.00326 | -0.08245 | 0.01473 | -0.12251 | -0.00178 | -0.02367 |
| 1290                | -0.29298 | -0.16337 | 1.00644 | -0.06463 | 0.01474 | -0.12326 | -0.00574 | -0.02802 |
| 1295                | -0.28127 | -0.15592 | 1.00894 | -0.04729 | 0.01562 | -0.12373 | -0.0096  | -0.03226 |
| 1300                | -0.27019 | -0.14829 | 1.01082 | -0.03048 | 0.01733 | -0.1239  | -0.01337 | -0.0364  |
| 1305                | -0.25975 | -0.14048 | 1.01214 | -0.01423 | 0.01979 | -0.12375 | -0.01704 | -0.04044 |
| 1310                | -0.24992 | -0.13249 | 1.01296 | 0.0014   | 0.02296 | -0.12327 | -0.02062 | -0.04439 |
| 1315                | -0.24071 | -0.12434 | 1.01334 | 0.01636  | 0.02677 | -0.12244 | -0.0241  | -0.04825 |
| 1320                | -0.23211 | -0.11602 | 1.01334 | 0.03062  | 0.03117 | -0.12125 | -0.0275  | -0.05202 |
| 1325                | -0.22411 | -0.10755 | 1.01302 | 0.04412  | 0.03608 | -0.11967 | -0.03082 | -0.0557  |

Table 52: Normalized Legendre coefficients in  $\pi^+p \rightarrow \Sigma^+K^+$  (1/7)

| Momentum<br>(MeV/c) | A1/A0    | A2/A0    | A3/A0   | A4/A0   | A5/A0   | A6/A0    | A7/A0    | A8/A0    |
|---------------------|----------|----------|---------|---------|---------|----------|----------|----------|
| 1330                | -0.21669 | -0.09894 | 1.01244 | 0.05683 | 0.04146 | -0.11769 | -0.03405 | -0.05931 |
| 1335                | -0.20985 | -0.09018 | 1.01164 | 0.06873 | 0.04726 | -0.1153  | -0.0372  | -0.06284 |
| 1340                | -0.20356 | -0.08129 | 1.01058 | 0.07985 | 0.0534  | -0.11252 | -0.04027 | -0.0663  |
| 1345                | -0.1978  | -0.07227 | 1.00928 | 0.0902  | 0.05986 | -0.10934 | -0.04327 | -0.06969 |
| 1350                | -0.19254 | -0.06312 | 1.00772 | 0.09984 | 0.06658 | -0.10577 | -0.0462  | -0.07301 |
| 1355                | -0.18776 | -0.05386 | 1.00587 | 0.10877 | 0.0735  | -0.10181 | -0.04906 | -0.07626 |
| 1360                | -0.18344 | -0.04449 | 1.00374 | 0.11704 | 0.08057 | -0.09747 | -0.05185 | -0.07945 |
| 1365                | -0.17954 | -0.03502 | 1.00131 | 0.12466 | 0.08776 | -0.09276 | -0.05457 | -0.08257 |
| 1370                | -0.17605 | -0.02545 | 0.99856 | 0.13168 | 0.09499 | -0.08768 | -0.05724 | -0.08564 |
| 1375                | -0.17294 | -0.01579 | 0.9955  | 0.13811 | 0.10224 | -0.08224 | -0.05984 | -0.08866 |
| 1380                | -0.1702  | -0.00605 | 0.99209 | 0.14399 | 0.10943 | -0.07644 | -0.06239 | -0.09161 |
| 1385                | -0.16779 | 0.00381  | 0.98832 | 0.14938 | 0.1165  | -0.07025 | -0.06488 | -0.09452 |
| 1390                | -0.16573 | 0.0138   | 0.98412 | 0.15434 | 0.12336 | -0.06361 | -0.06731 | -0.09737 |
| 1395                | -0.164   | 0.02398  | 0.97947 | 0.15895 | 0.1299  | -0.05648 | -0.06967 | -0.10017 |
| 1400                | -0.1626  | 0.03439  | 0.9743  | 0.16329 | 0.13604 | -0.04879 | -0.07197 | -0.10292 |
| 1405                | -0.16152 | 0.04506  | 0.96858 | 0.16742 | 0.14169 | -0.04049 | -0.0742  | -0.10562 |
| 1410                | -0.16076 | 0.05603  | 0.96225 | 0.17143 | 0.14675 | -0.03153 | -0.07636 | -0.10826 |
| 1415                | -0.16032 | 0.06735  | 0.95526 | 0.17539 | 0.15112 | -0.02185 | -0.07844 | -0.11086 |
| 1420                | -0.16018 | 0.07904  | 0.94758 | 0.17937 | 0.15471 | -0.01139 | -0.08045 | -0.1134  |
| 1425                | -0.16032 | 0.09115  | 0.93916 | 0.18348 | 0.15743 | -0.00014 | -0.08237 | -0.11589 |
| 1430                | -0.16072 | 0.10365  | 0.93    | 0.18788 | 0.15919 | 0.01187  | -0.08421 | -0.11833 |
| 1435                | -0.16131 | 0.11654  | 0.92008 | 0.19276 | 0.15988 | 0.02457  | -0.08596 | -0.12072 |
| 1440                | -0.16205 | 0.1298   | 0.90941 | 0.1983  | 0.15942 | 0.03792  | -0.08761 | -0.12307 |
| 1445                | -0.16288 | 0.14342  | 0.89797 | 0.20467 | 0.15771 | 0.05186  | -0.08916 | -0.12536 |
| 1450                | -0.16377 | 0.15738  | 0.88576 | 0.21207 | 0.15465 | 0.06634  | -0.09061 | -0.12762 |
| 1455                | -0.16466 | 0.17168  | 0.87277 | 0.22066 | 0.15015 | 0.08129  | -0.09195 | -0.12982 |
| 1460                | -0.16551 | 0.18629  | 0.85905 | 0.23052 | 0.14422 | 0.09666  | -0.09317 | -0.13198 |
| 1465                | -0.16627 | 0.20112  | 0.84472 | 0.2415  | 0.13711 | 0.11238  | -0.09429 | -0.13409 |
| 1470                | -0.16693 | 0.2161   | 0.82995 | 0.25341 | 0.12908 | 0.12838  | -0.09532 | -0.13613 |
| 1475                | -0.16745 | 0.23114  | 0.81489 | 0.26605 | 0.12041 | 0.14458  | -0.09627 | -0.13811 |
| 1480                | -0.16779 | 0.24618  | 0.7997  | 0.27923 | 0.11139 | 0.16091  | -0.09713 | -0.14    |
| 1485                | -0.16791 | 0.26112  | 0.78452 | 0.29277 | 0.10228 | 0.17731  | -0.09793 | -0.14181 |
| 1490                | -0.1678  | 0.27589  | 0.76952 | 0.30647 | 0.09336 | 0.19369  | -0.09867 | -0.14352 |
| 1495                | -0.1674  | 0.29043  | 0.75483 | 0.3202  | 0.08487 | 0.20999  | -0.09936 | -0.14512 |
| 1500                | -0.1667  | 0.30482  | 0.74056 | 0.33397 | 0.07697 | 0.22618  | -0.10001 | -0.14661 |
| 1505                | -0.16566 | 0.31913  | 0.7268  | 0.34786 | 0.06978 | 0.24223  | -0.10063 | -0.14797 |
| 1510                | -0.16426 | 0.33345  | 0.71365 | 0.36195 | 0.06342 | 0.25811  | -0.10122 | -0.14918 |
| 1515                | -0.16248 | 0.34775  | 0.70117 | 0.37616 | 0.05796 | 0.27376  | -0.10179 | -0.15025 |
| 1520                | -0.16029 | 0.36189  | 0.68942 | 0.39033 | 0.05345 | 0.28907  | -0.10234 | -0.15116 |
| 1525                | -0.15769 | 0.37579  | 0.67848 | 0.40443 | 0.04992 | 0.30396  | -0.10285 | -0.1519  |
| 1530                | -0.15466 | 0.38951  | 0.66844 | 0.41854 | 0.04734 | 0.31837  | -0.10332 | -0.15246 |
| 1535                | -0.1512  | 0.40308  | 0.65936 | 0.43276 | 0.04569 | 0.33227  | -0.10376 | -0.15285 |
| 1540                | -0.1473  | 0.41655  | 0.65133 | 0.44722 | 0.04496 | 0.34558  | -0.10416 | -0.15304 |
| 1545                | -0.14295 | 0.42994  | 0.64444 | 0.46201 | 0.04513 | 0.35827  | -0.10452 | -0.15303 |

Table 53: Normalized Legendre coefficients in  $\pi^+p \rightarrow \Sigma^+K^+$  (2/7)

| Momentum<br>(MeV/c) | A1/A0    | A2/A0   | A3/A0   | A4/A0   | A5/A0   | A6/A0   | A7/A0    | A8/A0    |
|---------------------|----------|---------|---------|---------|---------|---------|----------|----------|
| 1550                | -0.13812 | 0.44331 | 0.63877 | 0.47723 | 0.04617 | 0.37028 | -0.10483 | -0.15281 |
| 1555                | -0.13285 | 0.45667 | 0.63433 | 0.49295 | 0.04807 | 0.38161 | -0.10509 | -0.15238 |
| 1560                | -0.12715 | 0.46998 | 0.63098 | 0.50907 | 0.0508  | 0.39235 | -0.10532 | -0.15175 |
| 1565                | -0.1211  | 0.48319 | 0.62859 | 0.52549 | 0.05434 | 0.4026  | -0.1055  | -0.15093 |
| 1570                | -0.11473 | 0.49626 | 0.62699 | 0.5421  | 0.05865 | 0.41247 | -0.10565 | -0.14993 |
| 1575                | -0.10809 | 0.50913 | 0.62604 | 0.55881 | 0.06373 | 0.42208 | -0.10577 | -0.14877 |
| 1580                | -0.10123 | 0.52176 | 0.62558 | 0.57551 | 0.06953 | 0.43151 | -0.10585 | -0.14745 |
| 1585                | -0.09421 | 0.53411 | 0.62545 | 0.5921  | 0.07604 | 0.44089 | -0.10592 | -0.14599 |
| 1590                | -0.08706 | 0.54614 | 0.62557 | 0.60853 | 0.0832  | 0.45027 | -0.10596 | -0.1444  |
| 1595                | -0.07979 | 0.55784 | 0.62586 | 0.62474 | 0.09096 | 0.45965 | -0.10598 | -0.14269 |
| 1600                | -0.07245 | 0.56918 | 0.62625 | 0.6407  | 0.09925 | 0.46907 | -0.106   | -0.14085 |
| 1605                | -0.06505 | 0.58016 | 0.62668 | 0.65638 | 0.10801 | 0.47852 | -0.106   | -0.13891 |
| 1610                | -0.05762 | 0.59074 | 0.62707 | 0.67175 | 0.11718 | 0.48804 | -0.106   | -0.13687 |
| 1615                | -0.05018 | 0.60091 | 0.62737 | 0.68675 | 0.12668 | 0.49763 | -0.106   | -0.13474 |
| 1620                | -0.04276 | 0.61068 | 0.62751 | 0.70139 | 0.13648 | 0.50729 | -0.106   | -0.13252 |
| 1625                | -0.03535 | 0.62007 | 0.62748 | 0.71565 | 0.14651 | 0.51701 | -0.106   | -0.13022 |
| 1630                | -0.02796 | 0.62911 | 0.62727 | 0.72955 | 0.15674 | 0.52673 | -0.10601 | -0.12786 |
| 1635                | -0.02059 | 0.63784 | 0.62686 | 0.74311 | 0.16713 | 0.53644 | -0.10603 | -0.12544 |
| 1640                | -0.01324 | 0.6463  | 0.62623 | 0.75633 | 0.17762 | 0.54609 | -0.10605 | -0.12297 |
| 1645                | -0.00591 | 0.65451 | 0.62538 | 0.76923 | 0.18819 | 0.55565 | -0.10608 | -0.12045 |
| 1650                | 0.00139  | 0.66253 | 0.62428 | 0.78182 | 0.19879 | 0.5651  | -0.10612 | -0.1179  |
| 1655                | 0.00868  | 0.67037 | 0.62293 | 0.7941  | 0.20937 | 0.57439 | -0.10617 | -0.11533 |
| 1660                | 0.01593  | 0.67807 | 0.62131 | 0.8061  | 0.2199  | 0.58348 | -0.10623 | -0.11274 |
| 1665                | 0.02316  | 0.68568 | 0.6194  | 0.81783 | 0.23032 | 0.59236 | -0.1063  | -0.11014 |
| 1670                | 0.03036  | 0.69322 | 0.61719 | 0.82929 | 0.24061 | 0.60098 | -0.10638 | -0.10754 |
| 1675                | 0.03754  | 0.70073 | 0.61467 | 0.84049 | 0.2507  | 0.60931 | -0.10647 | -0.10495 |
| 1680                | 0.04468  | 0.70824 | 0.61182 | 0.85146 | 0.26058 | 0.61732 | -0.10658 | -0.10237 |
| 1685                | 0.05179  | 0.7158  | 0.60863 | 0.8622  | 0.27018 | 0.62497 | -0.1067  | -0.09982 |
| 1690                | 0.05886  | 0.72342 | 0.60508 | 0.87271 | 0.27946 | 0.63223 | -0.10684 | -0.09731 |
| 1695                | 0.06591  | 0.73112 | 0.60118 | 0.88299 | 0.28841 | 0.63907 | -0.10699 | -0.09483 |
| 1700                | 0.07293  | 0.73887 | 0.59694 | 0.893   | 0.29698 | 0.64545 | -0.10717 | -0.09241 |
| 1705                | 0.07993  | 0.74664 | 0.59238 | 0.90269 | 0.30516 | 0.65133 | -0.10736 | -0.09003 |
| 1710                | 0.08691  | 0.75441 | 0.58751 | 0.91203 | 0.31293 | 0.65668 | -0.10758 | -0.08772 |
| 1715                | 0.09388  | 0.76215 | 0.58234 | 0.92098 | 0.32025 | 0.66148 | -0.10782 | -0.08547 |
| 1720                | 0.10084  | 0.76985 | 0.5769  | 0.92954 | 0.32711 | 0.66572 | -0.10809 | -0.08329 |
| 1725                | 0.10779  | 0.77748 | 0.57123 | 0.93769 | 0.33352 | 0.66945 | -0.10838 | -0.08119 |
| 1730                | 0.11473  | 0.78502 | 0.56535 | 0.94547 | 0.33947 | 0.67271 | -0.10869 | -0.07918 |
| 1735                | 0.12166  | 0.79245 | 0.5593  | 0.95286 | 0.34495 | 0.67554 | -0.10902 | -0.07725 |
| 1740                | 0.12857  | 0.79975 | 0.55311 | 0.95988 | 0.34998 | 0.67799 | -0.10938 | -0.07542 |
| 1745                | 0.13547  | 0.80689 | 0.54682 | 0.96655 | 0.35453 | 0.68008 | -0.10975 | -0.07369 |
| 1750                | 0.14236  | 0.81386 | 0.54046 | 0.97285 | 0.35862 | 0.68187 | -0.11014 | -0.07206 |
| 1755                | 0.14923  | 0.82063 | 0.53405 | 0.97881 | 0.36224 | 0.6834  | -0.11054 | -0.07055 |
| 1760                | 0.15609  | 0.82719 | 0.52764 | 0.98443 | 0.36538 | 0.6847  | -0.11096 | -0.06915 |
| 1765                | 0.16293  | 0.83351 | 0.52126 | 0.98972 | 0.36805 | 0.68582 | -0.1114  | -0.06788 |

Table 54: Normalized Legendre coefficients in  $\pi^+p \rightarrow \Sigma^+K^+$  (3/7)

| Momentum<br>(MeV/c) | A1/A0   | A2/A0   | A3/A0   | A4/A0   | A5/A0   | A6/A0   | A7/A0    | A8/A0    |
|---------------------|---------|---------|---------|---------|---------|---------|----------|----------|
| 1770                | 0.16976 | 0.83957 | 0.51493 | 0.99469 | 0.37023 | 0.68679 | -0.11184 | -0.06673 |
| 1775                | 0.17657 | 0.84536 | 0.5087  | 0.99933 | 0.37194 | 0.68766 | -0.1123  | -0.06572 |
| 1780                | 0.18336 | 0.85084 | 0.50258 | 1.00367 | 0.37317 | 0.68847 | -0.11276 | -0.06485 |
| 1785                | 0.19009 | 0.856   | 0.49662 | 1.00768 | 0.37395 | 0.6892  | -0.11323 | -0.06413 |
| 1790                | 0.19674 | 0.86081 | 0.49082 | 1.01134 | 0.37429 | 0.68985 | -0.1137  | -0.06355 |
| 1795                | 0.20326 | 0.86526 | 0.48522 | 1.01465 | 0.37424 | 0.69042 | -0.11416 | -0.06312 |
| 1800                | 0.20962 | 0.86932 | 0.47982 | 1.01757 | 0.37382 | 0.69088 | -0.11461 | -0.06286 |
| 1805                | 0.21579 | 0.87298 | 0.47467 | 1.02009 | 0.37305 | 0.69124 | -0.11505 | -0.06275 |
| 1810                | 0.22172 | 0.8762  | 0.46977 | 1.0222  | 0.37196 | 0.69148 | -0.11547 | -0.06281 |
| 1815                | 0.22742 | 0.87899 | 0.46514 | 1.02388 | 0.37061 | 0.6916  | -0.11586 | -0.06304 |
| 1820                | 0.23286 | 0.88135 | 0.46074 | 1.02515 | 0.36904 | 0.69159 | -0.11622 | -0.06343 |
| 1825                | 0.23807 | 0.88327 | 0.45655 | 1.02601 | 0.36732 | 0.69146 | -0.11655 | -0.06399 |
| 1830                | 0.24305 | 0.88477 | 0.45254 | 1.02648 | 0.36551 | 0.69121 | -0.11683 | -0.06471 |
| 1835                | 0.2478  | 0.88586 | 0.4487  | 1.02655 | 0.36368 | 0.69084 | -0.11707 | -0.06558 |
| 1840                | 0.25232 | 0.88654 | 0.445   | 1.02625 | 0.36189 | 0.69035 | -0.11725 | -0.06662 |
| 1845                | 0.25663 | 0.88681 | 0.4414  | 1.02558 | 0.36021 | 0.68975 | -0.11736 | -0.06781 |
| 1850                | 0.26072 | 0.88668 | 0.43789 | 1.02454 | 0.35868 | 0.68902 | -0.11741 | -0.06915 |
| 1855                | 0.26461 | 0.88616 | 0.43444 | 1.02315 | 0.35739 | 0.68818 | -0.11739 | -0.07064 |
| 1860                | 0.2683  | 0.88526 | 0.43103 | 1.02142 | 0.35638 | 0.68723 | -0.11729 | -0.07228 |
| 1865                | 0.27179 | 0.88397 | 0.42763 | 1.01936 | 0.35573 | 0.68616 | -0.1171  | -0.07407 |
| 1870                | 0.27509 | 0.88231 | 0.42421 | 1.01697 | 0.35549 | 0.68497 | -0.11683 | -0.076   |
| 1875                | 0.2782  | 0.88028 | 0.42075 | 1.01426 | 0.35573 | 0.68367 | -0.11645 | -0.07808 |
| 1880                | 0.28114 | 0.87788 | 0.41722 | 1.01124 | 0.35651 | 0.68226 | -0.11597 | -0.08029 |
| 1885                | 0.28391 | 0.87515 | 0.41361 | 1.00795 | 0.35788 | 0.68074 | -0.11539 | -0.08265 |
| 1890                | 0.28657 | 0.87216 | 0.40992 | 1.00444 | 0.35986 | 0.67908 | -0.11469 | -0.08513 |
| 1895                | 0.28917 | 0.86899 | 0.40614 | 1.0008  | 0.36248 | 0.67727 | -0.11389 | -0.08774 |
| 1900                | 0.29176 | 0.86572 | 0.40227 | 0.99711 | 0.36575 | 0.67529 | -0.11297 | -0.09047 |
| 1905                | 0.2944  | 0.86244 | 0.39831 | 0.99344 | 0.3697  | 0.67313 | -0.11195 | -0.09332 |
| 1910                | 0.29714 | 0.85921 | 0.39426 | 0.98985 | 0.37433 | 0.67078 | -0.11082 | -0.09628 |
| 1915                | 0.3     | 0.85606 | 0.39014 | 0.98635 | 0.37962 | 0.66822 | -0.10957 | -0.09935 |
| 1920                | 0.30299 | 0.85298 | 0.38597 | 0.98292 | 0.38555 | 0.66549 | -0.10821 | -0.10252 |
| 1925                | 0.30612 | 0.84996 | 0.38177 | 0.97952 | 0.39207 | 0.6626  | -0.10674 | -0.10578 |
| 1930                | 0.3094  | 0.84699 | 0.37755 | 0.97614 | 0.39915 | 0.65955 | -0.10515 | -0.10914 |
| 1935                | 0.31283 | 0.84406 | 0.37334 | 0.97273 | 0.40676 | 0.65637 | -0.10345 | -0.11259 |
| 1940                | 0.31643 | 0.84117 | 0.36916 | 0.96929 | 0.41485 | 0.65306 | -0.10163 | -0.11612 |
| 1945                | 0.32021 | 0.83831 | 0.36503 | 0.96577 | 0.42339 | 0.64965 | -0.0997  | -0.11973 |
| 1950                | 0.32418 | 0.83547 | 0.36097 | 0.96215 | 0.43235 | 0.64615 | -0.09765 | -0.12341 |
| 1955                | 0.32835 | 0.83264 | 0.357   | 0.95841 | 0.44169 | 0.64256 | -0.09547 | -0.12717 |
| 1960                | 0.33272 | 0.82981 | 0.35313 | 0.95452 | 0.45138 | 0.63891 | -0.09318 | -0.13099 |
| 1965                | 0.3373  | 0.82698 | 0.3494  | 0.95046 | 0.46137 | 0.63521 | -0.09076 | -0.13488 |
| 1970                | 0.34212 | 0.82414 | 0.34581 | 0.94618 | 0.47163 | 0.63148 | -0.08822 | -0.13882 |
| 1975                | 0.34716 | 0.82128 | 0.3424  | 0.94168 | 0.48214 | 0.62772 | -0.08556 | -0.14281 |
| 1980                | 0.35244 | 0.81839 | 0.33921 | 0.93696 | 0.49286 | 0.62395 | -0.08278 | -0.14686 |
| 1985                | 0.35793 | 0.81546 | 0.33628 | 0.93204 | 0.50378 | 0.62017 | -0.07987 | -0.15094 |

Table 55: Normalized Legendre coefficients in  $\pi^+p \rightarrow \Sigma^+K^+$  (4/7)

| Momentum<br>(MeV/c) | A1/A0   | A2/A0   | A3/A0   | A4/A0   | A5/A0   | A6/A0   | A7/A0    | A8/A0    |
|---------------------|---------|---------|---------|---------|---------|---------|----------|----------|
| 1990                | 0.36362 | 0.81249 | 0.33367 | 0.92693 | 0.51489 | 0.61638 | -0.07685 | -0.15505 |
| 1995                | 0.3695  | 0.80947 | 0.33142 | 0.92167 | 0.52616 | 0.6126  | -0.07372 | -0.15918 |
| 2000                | 0.37557 | 0.80638 | 0.3296  | 0.91626 | 0.5376  | 0.60883 | -0.07047 | -0.16334 |
| 2005                | 0.38179 | 0.80326 | 0.32819 | 0.91074 | 0.54915 | 0.60509 | -0.0671  | -0.1675  |
| 2010                | 0.38815 | 0.80015 | 0.32716 | 0.90515 | 0.56081 | 0.60143 | -0.06363 | -0.17166 |
| 2015                | 0.39462 | 0.7971  | 0.32646 | 0.89952 | 0.57253 | 0.59787 | -0.06005 | -0.17582 |
| 2020                | 0.40118 | 0.79416 | 0.32605 | 0.8939  | 0.58428 | 0.59447 | -0.05636 | -0.17995 |
| 2025                | 0.40779 | 0.79138 | 0.32589 | 0.88831 | 0.59603 | 0.59126 | -0.05257 | -0.18406 |
| 2030                | 0.41443 | 0.78881 | 0.32593 | 0.8828  | 0.60774 | 0.58827 | -0.04866 | -0.18814 |
| 2035                | 0.42108 | 0.78649 | 0.32614 | 0.87741 | 0.61939 | 0.58555 | -0.04466 | -0.19217 |
| 2040                | 0.42771 | 0.78448 | 0.32648 | 0.87217 | 0.63095 | 0.58314 | -0.04055 | -0.19614 |
| 2045                | 0.4343  | 0.78283 | 0.32689 | 0.86712 | 0.64237 | 0.58107 | -0.03633 | -0.20006 |
| 2050                | 0.44082 | 0.78157 | 0.32734 | 0.8623  | 0.65363 | 0.57938 | -0.03202 | -0.2039  |
| 2055                | 0.44724 | 0.78077 | 0.32779 | 0.85775 | 0.66469 | 0.57812 | -0.0276  | -0.20766 |
| 2060                | 0.45354 | 0.78047 | 0.3282  | 0.8535  | 0.67553 | 0.57732 | -0.02309 | -0.21133 |
| 2065                | 0.4597  | 0.78072 | 0.32851 | 0.84959 | 0.68611 | 0.57701 | -0.01848 | -0.21491 |
| 2070                | 0.46568 | 0.78157 | 0.3287  | 0.84607 | 0.69639 | 0.57725 | -0.01377 | -0.21837 |
| 2075                | 0.47143 | 0.78303 | 0.32871 | 0.84292 | 0.70636 | 0.57806 | -0.00896 | -0.22172 |
| 2080                | 0.47686 | 0.78509 | 0.32848 | 0.84013 | 0.71598 | 0.57948 | -0.00406 | -0.22495 |
| 2085                | 0.48188 | 0.78773 | 0.32797 | 0.83768 | 0.72524 | 0.58154 | 0.00093  | -0.22805 |
| 2090                | 0.48641 | 0.79094 | 0.32711 | 0.83553 | 0.73411 | 0.58428 | 0.00601  | -0.231   |
| 2095                | 0.49037 | 0.79472 | 0.32585 | 0.83367 | 0.74256 | 0.58772 | 0.01118  | -0.23381 |
| 2100                | 0.49366 | 0.79904 | 0.32414 | 0.83207 | 0.75058 | 0.5919  | 0.01644  | -0.23647 |
| 2105                | 0.49624 | 0.80389 | 0.32195 | 0.83071 | 0.75815 | 0.59681 | 0.02178  | -0.23896 |
| 2110                | 0.49816 | 0.80918 | 0.31935 | 0.82953 | 0.76531 | 0.60238 | 0.02721  | -0.24129 |
| 2115                | 0.49948 | 0.81487 | 0.31641 | 0.82851 | 0.77211 | 0.60852 | 0.03272  | -0.24344 |
| 2120                | 0.50026 | 0.82088 | 0.31321 | 0.82758 | 0.77857 | 0.61513 | 0.0383   | -0.24542 |
| 2125                | 0.50056 | 0.82715 | 0.30981 | 0.82672 | 0.78474 | 0.62213 | 0.04397  | -0.24723 |
| 2130                | 0.50044 | 0.8336  | 0.3063  | 0.82587 | 0.79067 | 0.62942 | 0.04971  | -0.24885 |
| 2135                | 0.49996 | 0.84017 | 0.30274 | 0.82499 | 0.79638 | 0.63691 | 0.05552  | -0.25028 |
| 2140                | 0.49918 | 0.84679 | 0.29921 | 0.82405 | 0.80192 | 0.64451 | 0.0614   | -0.25152 |
| 2145                | 0.49816 | 0.8534  | 0.29578 | 0.82298 | 0.80733 | 0.65213 | 0.06735  | -0.25257 |
| 2150                | 0.49696 | 0.85993 | 0.29252 | 0.82176 | 0.81265 | 0.65968 | 0.07337  | -0.25341 |
| 2155                | 0.49565 | 0.86631 | 0.2895  | 0.82034 | 0.81792 | 0.66707 | 0.07946  | -0.25406 |
| 2160                | 0.49428 | 0.87251 | 0.28679 | 0.81869 | 0.82315 | 0.67424 | 0.0856   | -0.25449 |
| 2165                | 0.49291 | 0.87852 | 0.28443 | 0.81682 | 0.82835 | 0.68115 | 0.09182  | -0.25473 |
| 2170                | 0.49162 | 0.88433 | 0.28247 | 0.81472 | 0.83352 | 0.68777 | 0.0981   | -0.25475 |
| 2175                | 0.49046 | 0.88995 | 0.28095 | 0.81239 | 0.83868 | 0.69406 | 0.10444  | -0.25457 |
| 2180                | 0.48949 | 0.89536 | 0.27992 | 0.80982 | 0.84381 | 0.69997 | 0.11086  | -0.25418 |
| 2185                | 0.48879 | 0.90056 | 0.27942 | 0.807   | 0.84893 | 0.70549 | 0.11735  | -0.25358 |
| 2190                | 0.48842 | 0.90554 | 0.27951 | 0.80394 | 0.85403 | 0.71055 | 0.12391  | -0.25277 |
| 2195                | 0.48843 | 0.9103  | 0.28022 | 0.80063 | 0.85913 | 0.71514 | 0.13054  | -0.25176 |
| 2200                | 0.48889 | 0.91482 | 0.28161 | 0.79707 | 0.86422 | 0.71922 | 0.13725  | -0.25053 |
| 2205                | 0.48982 | 0.91912 | 0.28367 | 0.7933  | 0.86934 | 0.72283 | 0.14403  | -0.24909 |

Table 56: Normalized Legendre coefficients in  $\pi^+p \rightarrow \Sigma^+K^+$  (5/7)



| Momentum<br>(MeV/c) | A1/A0   | A2/A0   | A3/A0   | A4/A0   | A5/A0   | A6/A0   | A7/A0   | A8/A0    |
|---------------------|---------|---------|---------|---------|---------|---------|---------|----------|
| 2210                | 0.4912  | 0.9232  | 0.28639 | 0.7894  | 0.87452 | 0.72605 | 0.15087 | -0.24744 |
| 2215                | 0.49301 | 0.92707 | 0.28974 | 0.78543 | 0.8798  | 0.72899 | 0.15778 | -0.24558 |
| 2220                | 0.49524 | 0.93074 | 0.29369 | 0.78147 | 0.88522 | 0.73175 | 0.16474 | -0.24351 |
| 2225                | 0.49787 | 0.93422 | 0.29822 | 0.7776  | 0.89083 | 0.7344  | 0.17175 | -0.24122 |
| 2230                | 0.50089 | 0.93753 | 0.30331 | 0.77388 | 0.89667 | 0.73706 | 0.17881 | -0.23871 |
| 2235                | 0.50427 | 0.94067 | 0.30894 | 0.7704  | 0.90277 | 0.73982 | 0.1859  | -0.23598 |
| 2240                | 0.508   | 0.94365 | 0.31507 | 0.76723 | 0.90918 | 0.74276 | 0.19303 | -0.23304 |
| 2245                | 0.51205 | 0.94648 | 0.32167 | 0.76443 | 0.91593 | 0.74598 | 0.20019 | -0.22988 |
| 2250                | 0.51641 | 0.9492  | 0.32868 | 0.76206 | 0.92297 | 0.7495  | 0.20737 | -0.2265  |
| 2255                | 0.52101 | 0.95185 | 0.336   | 0.76017 | 0.93022 | 0.75331 | 0.21457 | -0.22289 |
| 2260                | 0.52581 | 0.95446 | 0.34353 | 0.75879 | 0.93762 | 0.7574  | 0.22179 | -0.21908 |
| 2265                | 0.53077 | 0.95707 | 0.35118 | 0.75797 | 0.94507 | 0.76177 | 0.229   | -0.21504 |
| 2270                | 0.53584 | 0.95972 | 0.35885 | 0.75775 | 0.95251 | 0.7664  | 0.23622 | -0.21079 |
| 2275                | 0.54099 | 0.96245 | 0.36644 | 0.75818 | 0.95985 | 0.77129 | 0.24343 | -0.20631 |
| 2280                | 0.54615 | 0.96531 | 0.37387 | 0.7593  | 0.96701 | 0.77643 | 0.25063 | -0.20163 |
| 2285                | 0.5513  | 0.96832 | 0.38104 | 0.76114 | 0.97393 | 0.78182 | 0.25781 | -0.19672 |
| 2290                | 0.55637 | 0.97153 | 0.38784 | 0.76377 | 0.98051 | 0.78743 | 0.26496 | -0.19161 |
| 2295                | 0.56134 | 0.97498 | 0.3942  | 0.7672  | 0.9867  | 0.79328 | 0.27209 | -0.18627 |
| 2300                | 0.56619 | 0.97866 | 0.4001  | 0.77142 | 0.99246 | 0.79937 | 0.27918 | -0.18073 |
| 2305                | 0.57092 | 0.98258 | 0.40554 | 0.77638 | 0.99779 | 0.80572 | 0.28624 | -0.17498 |
| 2310                | 0.57554 | 0.98672 | 0.41053 | 0.78203 | 1.0027  | 0.81236 | 0.29326 | -0.16902 |
| 2315                | 0.58005 | 0.99108 | 0.41507 | 0.78832 | 1.00719 | 0.8193  | 0.30024 | -0.16286 |
| 2320                | 0.58445 | 0.99565 | 0.41919 | 0.79521 | 1.01125 | 0.82658 | 0.30717 | -0.1565  |
| 2325                | 0.58875 | 1.00043 | 0.42288 | 0.80265 | 1.01489 | 0.8342  | 0.31406 | -0.14995 |
| 2330                | 0.59294 | 1.0054  | 0.42615 | 0.81059 | 1.01809 | 0.8422  | 0.3209  | -0.14321 |
| 2335                | 0.59702 | 1.01057 | 0.42902 | 0.81897 | 1.02088 | 0.85059 | 0.32769 | -0.13629 |
| 2340                | 0.60101 | 1.01591 | 0.43149 | 0.82776 | 1.02323 | 0.8594  | 0.33442 | -0.12918 |
| 2345                | 0.60491 | 1.02144 | 0.43357 | 0.83691 | 1.02516 | 0.86865 | 0.3411  | -0.12189 |
| 2350                | 0.60869 | 1.02714 | 0.43525 | 0.84638 | 1.02664 | 0.87834 | 0.34772 | -0.11443 |
| 2355                | 0.61231 | 1.03305 | 0.43655 | 0.85621 | 1.02762 | 0.88845 | 0.35428 | -0.10679 |
| 2360                | 0.61572 | 1.03919 | 0.43744 | 0.86642 | 1.02803 | 0.89895 | 0.36077 | -0.09899 |
| 2365                | 0.61886 | 1.04558 | 0.43793 | 0.87705 | 1.02781 | 0.90981 | 0.3672  | -0.09103 |
| 2370                | 0.62167 | 1.05226 | 0.438   | 0.88814 | 1.0269  | 0.921   | 0.37355 | -0.08291 |
| 2375                | 0.6241  | 1.05925 | 0.43764 | 0.8997  | 1.02524 | 0.93248 | 0.37983 | -0.07463 |
| 2380                | 0.62609 | 1.06658 | 0.43686 | 0.91178 | 1.02275 | 0.94422 | 0.38604 | -0.06621 |
| 2385                | 0.62761 | 1.07425 | 0.43564 | 0.92439 | 1.01942 | 0.95621 | 0.39216 | -0.05765 |
| 2390                | 0.62867 | 1.08225 | 0.43401 | 0.9375  | 1.01527 | 0.96843 | 0.39821 | -0.04895 |
| 2395                | 0.62929 | 1.09054 | 0.43198 | 0.95108 | 1.01035 | 0.98089 | 0.40419 | -0.04013 |
| 2400                | 0.6295  | 1.09908 | 0.4296  | 0.9651  | 1.0047  | 0.99357 | 0.4101  | -0.03119 |
| 2405                | 0.6293  | 1.10785 | 0.42686 | 0.97951 | 0.99837 | 1.00648 | 0.41594 | -0.02213 |
| 2410                | 0.62872 | 1.11682 | 0.4238  | 0.9943  | 0.9914  | 1.0196  | 0.42171 | -0.01297 |
| 2415                | 0.62778 | 1.12594 | 0.42043 | 1.00942 | 0.98384 | 1.03294 | 0.42742 | -0.00372 |
| 2420                | 0.6265  | 1.1352  | 0.41678 | 1.02485 | 0.97573 | 1.0465  | 0.43307 | 0.00562  |
| 2425                | 0.6249  | 1.14456 | 0.41287 | 1.04055 | 0.96711 | 1.06025 | 0.43866 | 0.01503  |
| 2430                | 0.62298 | 1.15399 | 0.40873 | 1.05648 | 0.95803 | 1.07421 | 0.4442  | 0.02452  |
| 2435                | 0.62079 | 1.16345 | 0.40436 | 1.07263 | 0.94853 | 1.08837 | 0.44968 | 0.03407  |

Table 57: Normalized Legendre coefficients in  $\pi^+p \rightarrow \Sigma^+K^+$  (6/7)

| Momentum<br>(MeV/c) | A1/A0   | A2/A0   | A3/A0   | A4/A0   | A5/A0   | A6/A0   | A7/A0   | A8/A0   |
|---------------------|---------|---------|---------|---------|---------|---------|---------|---------|
| 2440                | 0.61833 | 1.17291 | 0.3998  | 1.08894 | 0.93866 | 1.10272 | 0.45511 | 0.04368 |
| 2445                | 0.61563 | 1.18237 | 0.39507 | 1.1054  | 0.92847 | 1.11725 | 0.4605  | 0.05333 |
| 2450                | 0.61273 | 1.19182 | 0.39019 | 1.12199 | 0.918   | 1.13193 | 0.46585 | 0.06302 |
| 2455                | 0.60967 | 1.20126 | 0.3852  | 1.13867 | 0.9073  | 1.14673 | 0.47117 | 0.07275 |
| 2460                | 0.60647 | 1.2107  | 0.38011 | 1.15544 | 0.89642 | 1.16162 | 0.47647 | 0.0825  |
| 2465                | 0.60319 | 1.22014 | 0.37495 | 1.17226 | 0.88542 | 1.17659 | 0.48175 | 0.09227 |
| 2470                | 0.59984 | 1.22958 | 0.36976 | 1.18912 | 0.87434 | 1.19159 | 0.48702 | 0.10205 |
| 2475                | 0.59648 | 1.23901 | 0.36454 | 1.20599 | 0.86322 | 1.20662 | 0.49228 | 0.11184 |

Table 58: Normalized Legendre coefficients in  $\pi^+p \rightarrow \Sigma^+K^+$  (7/7)
